# Supplementary material for: Logic Explained Networks
Source: arXiv:2108.05149 source file (2021-08-11)
Supplement: Supplementary file 1 [file supplementary_tables.tex]

% Please add the following required packages to your document preamble:
% \usepackage{multirow}
% \usepackage{graphicx}
\begin{table}[]
\centering
\caption{XOR explanations}
\label{tab:my-table}
\resizebox{\textwidth}{!}{%
\begin{tabular}{clllll}
\hline
\multirow{2}{*}{\textbf{Method}} &
  \multicolumn{2}{c}{\textbf{Positive explanation}} &
  \multicolumn{2}{c}{\textbf{Negative explanation}} &
  \multicolumn{1}{c}{\multirow{2}{*}{\textbf{Model's accuracy}}} \\
 &
  \textbf{Formula} &
  \textbf{Accuracy (\%)} &
  \textbf{Formula} &
  \textbf{Accuracy (\%)} &
  \multicolumn{1}{c}{} \\ \hline
\multirow{10}{*}{LIME} &
  $(c1 \wedge  \neg c2) \vee (c2 \wedge  \neg c1)$ &
  $100.00$ &
  $(c1 \wedge c2) \vee ( \neg c1 \wedge  \neg c2)$ &
  $100.00$ &
  $100.00$ \\
 &
  $(c1 \wedge  \neg c2) \vee (c2 \wedge  \neg c1)$ &
  $100.00$ &
  $(c1 \wedge c2) \vee ( \neg c1 \wedge  \neg c2)$ &
  $100.00$ &
  $100.00$ \\
 &
  $(c1 \wedge  \neg c2) \vee (c2 \wedge  \neg c1)$ &
  $100.00$ &
  $(c1 \wedge c2) \vee ( \neg c1 \wedge  \neg c2)$ &
  $100.00$ &
  $100.00$ \\
 &
  $(c1 \wedge  \neg c2) \vee (c2 \wedge  \neg c1)$ &
  $100.00$ &
  $(c1 \wedge c2) \vee ( \neg c1 \wedge  \neg c2)$ &
  $100.00$ &
  $100.00$ \\
 &
  $(c1 \wedge  \neg c2) \vee (c2 \wedge  \neg c1)$ &
  $100.00$ &
  $(c1 \wedge c2) \vee ( \neg c1 \wedge  \neg c2)$ &
  $100.00$ &
  $100.00$ \\
 &
  $(c1 \wedge  \neg c2) \vee (c2 \wedge  \neg c1)$ &
  $100.00$ &
  $(c1 \wedge c2) \vee ( \neg c1 \wedge  \neg c2)$ &
  $100.00$ &
  $100.00$ \\
 &
  $(c1 \wedge  \neg c2) \vee (c2 \wedge  \neg c1)$ &
  $100.00$ &
  $(c1 \wedge c2) \vee ( \neg c1 \wedge  \neg c2)$ &
  $100.00$ &
  $100.00$ \\
 &
  $(c1 \wedge  \neg c2) \vee (c2 \wedge  \neg c1)$ &
  $100.00$ &
  $(c1 \wedge c2) \vee ( \neg c1 \wedge  \neg c2)$ &
  $100.00$ &
  $100.00$ \\
 &
  $(c1 \wedge  \neg c2) \vee (c2 \wedge  \neg c1)$ &
  $100.00$ &
  $(c1 \wedge c2) \vee ( \neg c1 \wedge  \neg c2)$ &
  $100.00$ &
  $100.00$ \\
 &
  $(c1 \wedge  \neg c2) \vee (c2 \wedge  \neg c1)$ &
  $100.00$ &
  $(c1 \wedge c2) \vee ( \neg c1 \wedge  \neg c2)$ &
  $100.00$ &
  $100.00$ \\ \hline
\multirow{10}{*}{Pruning} &
  $(c1 \wedge  \neg c2) \vee (c2 \wedge  \neg c1)$ &
  $100.00$ &
  $(c1 \wedge c2) \vee ( \neg c1 \wedge  \neg c2)$ &
  $100.00$ &
  $100.00$ \\
 &
  $(c1 \wedge  \neg c2) \vee (c2 \wedge  \neg c1)$ &
  $100.00$ &
  $(c1 \wedge c2) \vee ( \neg c1 \wedge  \neg c2)$ &
  $100.00$ &
  $100.00$ \\
 &
  $(c1 \wedge  \neg c2) \vee (c2 \wedge  \neg c1)$ &
  $100.00$ &
  $(c1 \wedge c2) \vee ( \neg c1 \wedge  \neg c2)$ &
  $100.00$ &
  $100.00$ \\
 &
  $(c1 \wedge  \neg c2) \vee (c2 \wedge  \neg c1)$ &
  $100.00$ &
  $(c1 \wedge c2) \vee ( \neg c1 \wedge  \neg c2)$ &
  $100.00$ &
  $100.00$ \\
 &
  $(c1 \wedge  \neg c2) \vee (c2 \wedge  \neg c1)$ &
  $100.00$ &
  $(c1 \wedge c2) \vee ( \neg c1 \wedge  \neg c2)$ &
  $100.00$ &
  $100.00$ \\
 &
  $(c1 \wedge  \neg c2) \vee (c2 \wedge  \neg c1)$ &
  $100.00$ &
  $(c1 \wedge c2) \vee ( \neg c1 \wedge  \neg c2)$ &
  $100.00$ &
  $100.00$ \\
 &
  $(c1 \wedge  \neg c2) \vee (c2 \wedge  \neg c1)$ &
  $100.00$ &
  $(c1 \wedge c2) \vee ( \neg c1 \wedge  \neg c2)$ &
  $100.00$ &
  $100.00$ \\
 &
  $(c1 \wedge  \neg c2) \vee (c2 \wedge  \neg c1)$ &
  $100.00$ &
  $(c1 \wedge c2) \vee ( \neg c1 \wedge  \neg c2)$ &
  $100.00$ &
  $100.00$ \\
 &
  $(c1 \wedge  \neg c2) \vee (c2 \wedge  \neg c1)$ &
  $100.00$ &
  $(c1 \wedge c2) \vee ( \neg c1 \wedge  \neg c2)$ &
  $100.00$ &
  $100.00$ \\
 &
  $(c1 \wedge  \neg c2) \vee (c2 \wedge  \neg c1)$ &
  $100.00$ &
  $(c1 \wedge c2) \vee ( \neg c1 \wedge  \neg c2)$ &
  $100.00$ &
  $100.00$ \\ \hline
\multirow{10}{*}{$\psi$ net} &
  $((c1 \wedge  \neg c2) \vee (c2 \wedge  \neg c1))$ &
  $100.00$ &
  $( \neg c1 \wedge  \neg c2)$ &
  $88.89$ &
  $88.89$ \\
 &
  $((c1 \wedge  \neg c2) \vee (c2 \wedge  \neg c1))$ &
  $100.00$ &
  $((c1 \wedge c2) \vee ( \neg c1 \wedge  \neg c2))$ &
  $100.00$ &
  $77.78$ \\
 &
  $((c1 \wedge  \neg c2) \vee (c2 \wedge  \neg c1))$ &
  $100.00$ &
  $((c1 \wedge c2) \vee ( \neg c1 \wedge  \neg c2))$ &
  $100.00$ &
  $100.00$ \\
 &
  $((c1 \wedge  \neg c2) \vee (c2 \wedge  \neg c1))$ &
  $100.00$ &
  $(c2 \vee  \neg c1)$ &
  $44.44$ &
  $44.44$ \\
 &
  $((c1 \wedge  \neg c2) \vee (c2 \wedge  \neg c1))$ &
  $100.00$ &
  $((c1 \wedge c2) \vee ( \neg c1 \wedge  \neg c2))$ &
  $100.00$ &
  $77.78$ \\
 &
  $(c2 \wedge  \neg c1)$ &
  $77.78$ &
  $((c1 \wedge c2) \vee ( \neg c1 \wedge  \neg c2))$ &
  $100.00$ &
  $100.00$ \\
 &
  $(c2 \wedge  \neg c1)$ &
  $77.78$ &
  $( \neg c1 \wedge  \neg c2)$ &
  $88.89$ &
  $44.44$ \\
 &
  $(c1 \wedge  \neg c2)$ &
  $44.44$ &
  $((c1 \wedge c2) \vee ( \neg c1 \wedge  \neg c2))$ &
  $100.00$ &
  $100.00$ \\
 &
  $((c1 \wedge  \neg c2) \vee (c2 \wedge  \neg c1))$ &
  $100.00$ &
  $(c1 \wedge c2)$ &
  $88.89$ &
  $77.78$ \\
 &
  $(c1 \vee c2)$ &
  $100.00$ &
  $(c1 \vee  \neg c2)$ &
  $77.78$ &
  $77.78$ \\ \hline
\multirow{10}{*}{Decision tree} &
  $(c2  \leq  0.50 \wedge c1 > 0.50) \vee (c2 > 0.50 \wedge c1  \leq  0.50)$ &
  $100.00$ &
  $(c2  \leq  0.50 \wedge c1  \leq  0.50) \vee (c2 > 0.50 \wedge c1 > 0.50)$ &
  $100.00$ &
  $100.00$ \\
 &
  $(c1  \leq  0.50 \wedge c2 > 0.50) \vee (c1 > 0.50 \wedge c2  \leq  0.50)$ &
  $100.00$ &
  $(c1  \leq  0.50 \wedge c2  \leq  0.50) \vee (c1 > 0.50 \wedge c2 > 0.50)$ &
  $100.00$ &
  $100.00$ \\
 &
  $(c1  \leq  0.50 \wedge c2 > 0.50) \vee (c1 > 0.50 \wedge c2  \leq  0.50)$ &
  $100.00$ &
  $(c1  \leq  0.50 \wedge c2  \leq  0.50) \vee (c1 > 0.50 \wedge c2 > 0.50)$ &
  $100.00$ &
  $100.00$ \\
 &
  $(c1  \leq  0.50 \wedge c2 > 0.50) \vee (c1 > 0.50 \wedge c2  \leq  0.50)$ &
  $100.00$ &
  $(c1  \leq  0.50 \wedge c2  \leq  0.50) \vee (c1 > 0.50 \wedge c2 > 0.50)$ &
  $100.00$ &
  $100.00$ \\
 &
  $(c1  \leq  0.50 \wedge c2 > 0.50) \vee (c1 > 0.50 \wedge c2  \leq  0.50)$ &
  $100.00$ &
  $(c1  \leq  0.50 \wedge c2  \leq  0.50) \vee (c1 > 0.50 \wedge c2 > 0.50)$ &
  $100.00$ &
  $100.00$ \\
 &
  $(c2  \leq  0.50 \wedge c1 > 0.50) \vee (c2 > 0.50 \wedge c1  \leq  0.50)$ &
  $100.00$ &
  $(c2  \leq  0.50 \wedge c1  \leq  0.50) \vee (c2 > 0.50 \wedge c1 > 0.50)$ &
  $100.00$ &
  $100.00$ \\
 &
  $(c1  \leq  0.50 \wedge c2 > 0.50) \vee (c1 > 0.50 \wedge c2  \leq  0.50)$ &
  $100.00$ &
  $(c1  \leq  0.50 \wedge c2  \leq  0.50) \vee (c1 > 0.50 \wedge c2 > 0.50)$ &
  $100.00$ &
  $100.00$ \\
 &
  $(c2  \leq  0.50 \wedge c1 > 0.50) \vee (c2 > 0.50 \wedge c1  \leq  0.50)$ &
  $100.00$ &
  $(c2  \leq  0.50 \wedge c1  \leq  0.50) \vee (c2 > 0.50 \wedge c1 > 0.50)$ &
  $100.00$ &
  $100.00$ \\
 &
  $(c2  \leq  0.50 \wedge c1 > 0.50) \vee (c2 > 0.50 \wedge c1  \leq  0.50)$ &
  $100.00$ &
  $(c2  \leq  0.50 \wedge c1  \leq  0.50) \vee (c2 > 0.50 \wedge c1 > 0.50)$ &
  $100.00$ &
  $100.00$ \\
 &
  $(c1  \leq  0.50 \wedge c2 > 0.50) \vee (c1 > 0.50 \wedge c2  \leq  0.50)$ &
  $100.00$ &
  $(c1  \leq  0.50 \wedge c2  \leq  0.50) \vee (c1 > 0.50 \wedge c2 > 0.50)$ &
  $100.00$ &
  $100.00$ \\ \hline
\multirow{10}{*}{ReLU} &
  $(c1 \wedge  \neg c2) \vee (c2 \wedge  \neg c1)$ &
  $100.00$ &
  $(c1 \wedge c2) \vee ( \neg c1 \wedge  \neg c2)$ &
  $100.00$ &
  $100.00$ \\
 &
  $(c1 \wedge  \neg c2) \vee (c2 \wedge  \neg c1)$ &
  $100.00$ &
  $(c1 \wedge c2) \vee ( \neg c1 \wedge  \neg c2)$ &
  $100.00$ &
  $100.00$ \\
 &
  $(c1 \wedge  \neg c2) \vee (c2 \wedge  \neg c1)$ &
  $100.00$ &
  $(c1 \wedge c2) \vee ( \neg c1 \wedge  \neg c2)$ &
  $100.00$ &
  $100.00$ \\
 &
  $(c1 \wedge  \neg c2) \vee (c2 \wedge  \neg c1)$ &
  $100.00$ &
  $(c1 \wedge c2) \vee ( \neg c1 \wedge  \neg c2)$ &
  $100.00$ &
  $100.00$ \\
 &
  $(c1 \wedge  \neg c2) \vee (c2 \wedge  \neg c1)$ &
  $100.00$ &
  $(c1 \wedge c2) \vee ( \neg c1 \wedge  \neg c2)$ &
  $100.00$ &
  $100.00$ \\
 &
  $c1 \vee c2$ &
  $100.00$ &
  $(c1 \wedge c2) \vee ( \neg c1 \wedge  \neg c2)$ &
  $100.00$ &
  $100.00$ \\
 &
  $ \neg c1 \vee  \neg c2$ &
  $100.00$ &
  $c2 \vee  \neg c1$ &
  $44.44$ &
  $100.00$ \\
 &
  $(c1 \wedge  \neg c2) \vee (c2 \wedge  \neg c1)$ &
  $100.00$ &
  $(c1 \wedge c2) \vee ( \neg c1 \wedge  \neg c2)$ &
  $100.00$ &
  $100.00$ \\
 &
  $(c1 \wedge  \neg c2) \vee (c2 \wedge  \neg c1)$ &
  $100.00$ &
  $(c1 \wedge c2) \vee ( \neg c1 \wedge  \neg c2)$ &
  $100.00$ &
  $100.00$ \\
 &
  $(c1 \wedge  \neg c2) \vee (c2 \wedge  \neg c1)$ &
  $100.00$ &
  $(c1 \wedge c2) \vee ( \neg c1 \wedge  \neg c2)$ &
  $100.00$ &
  $100.00$ \\ \hline
\end{tabular}%
}
\end{table}

% Please add the following required packages to your document preamble:
% \usepackage{multirow}
% \usepackage{graphicx}
\begin{table}[]
\centering
\caption{MNIST explanations}
\label{tab:exp_formula_mnist_cbm}
\resizebox{\textwidth}{!}{%
\begin{tabular}{c|p{10cm}|l|p{10cm}|ll}
\hline
\multirow{2}{*}{\textbf{Method}} &
  \multicolumn{2}{c}{\textbf{Odd explanation}} &
  \multicolumn{2}{c}{\textbf{Even explanation}} &
  \multicolumn{1}{c}{\multirow{2}{*}{\textbf{Model's accuracy}}} \\
 &
  \textbf{Formula} &
  \textbf{Accuracy (\%)} &
  \textbf{Formula} &
  \textbf{Accuracy (\%)} &
  \multicolumn{1}{c}{} \\ \hline
\multirow{10}{*}{Pruning} &
  $ \neg c0 \wedge  \neg c2 \wedge  \neg c4 \wedge  \neg c6 \wedge  \neg c8$ &
  $100.00$ &
  $c0 \vee c2 \vee c4 \vee c6 \vee c8$ &
  $100.00$ &
  $100.00$ \\
 &
  $c1 \vee c3 \vee c5 \vee c7 \vee c9$ &
  $100.00$ &
  $ \neg c1 \wedge  \neg c3 \wedge  \neg c5 \wedge  \neg c7 \wedge  \neg c9$ &
  $100.00$ &
  $100.00$ \\
 &
  $c1 \vee c3 \vee c5 \vee c7 \vee c9$ &
  $100.00$ &
  $ \neg c1 \wedge  \neg c3 \wedge  \neg c5 \wedge  \neg c7 \wedge  \neg c9$ &
  $100.00$ &
  $100.00$ \\
 &
  $ \neg c0 \wedge  \neg c2 \wedge  \neg c4 \wedge  \neg c6 \wedge  \neg c8$ &
  $100.00$ &
  $c0 \vee c2 \vee c4 \vee c6 \vee c8$ &
  $100.00$ &
  $100.00$ \\
 &
  $c1 \vee c3 \vee c5 \vee c7 \vee c9$ &
  $100.00$ &
  $ \neg c1 \wedge  \neg c3 \wedge  \neg c5 \wedge  \neg c7 \wedge  \neg c9$ &
  $100.00$ &
  $100.00$ \\
 &
  $c1 \vee c3 \vee c5 \vee c7 \vee c9$ &
  $100.00$ &
  $ \neg c1 \wedge  \neg c3 \wedge  \neg c5 \wedge  \neg c7 \wedge  \neg c9$ &
  $100.00$ &
  $100.00$ \\
 &
  $c1 \vee c3 \vee c5 \vee c7 \vee c9$ &
  $100.00$ &
  $ \neg c1 \wedge  \neg c3 \wedge  \neg c5 \wedge  \neg c7 \wedge  \neg c9$ &
  $100.00$ &
  $100.00$ \\
 &
  $ \neg c0 \wedge  \neg c2 \wedge  \neg c4 \wedge  \neg c6 \wedge  \neg c8$ &
  $100.00$ &
  $c0 \vee c2 \vee c4 \vee c6 \vee c8$ &
  $100.00$ &
  $100.00$ \\
 &
  $ \neg c0 \wedge  \neg c2 \wedge  \neg c4 \wedge  \neg c6 \wedge  \neg c8$ &
  $100.00$ &
  $c0 \vee c2 \vee c4 \vee c6 \vee c8$ &
  $100.00$ &
  $100.00$ \\
 &
  $c1 \vee c3 \vee c5 \vee c7 \vee c9$ &
  $100.00$ &
  $ \neg c1 \wedge  \neg c3 \wedge  \neg c5 \wedge  \neg c7 \wedge  \neg c9$ &
  $100.00$ &
  $100.00$ \\ \hline
\multirow{10}{*}{$\psi$ net} &
  $(c7 \wedge  \neg c4)$ &
  $59.54$ &
  $( \neg c3 \wedge  \neg c5)$ &
  $68.28$ &
  $89.91$ \\
 &
  $( \neg c4 \wedge (c1 \vee c3) \wedge (c1 \vee  \neg c8))$ &
  $49.13$ &
  $( \neg c1 \wedge (c0 \vee c6) \wedge (c0 \vee  \neg c3) \wedge (c4 \vee  \neg c5))$ &
  $58.18$ &
  $79.63$ \\
 &
  $( \neg c8 \wedge (c1 \vee  \neg c2) \wedge (c3 \vee  \neg c0) \wedge ( \neg c2 \vee  \neg c6))$ &
  $19.56$ &
  $( \neg c1 \wedge  \neg c9 \wedge (c0 \vee  \neg c7))$ &
  $59.54$ &
  $80.98$ \\
 &
  $(c7 \vee c9 \vee ( \neg c4 \wedge  \neg c8) \vee (c3 \wedge  \neg c0 \wedge  \neg c4))$ &
  $39.83$ &
  $( \neg c3 \wedge (c2 \vee c4 \vee c8) \wedge (c2 \vee c8 \vee  \neg c7))$ &
  $59.54$ &
  $80.62$ \\
 &
  $( \neg c4 \wedge  \neg c8 \wedge (c7 \vee  \neg c6) \wedge (c9 \vee  \neg c2))$ &
  $40.69$ &
  $((c0 \wedge c8) \vee (c2 \wedge c8) \vee (c0 \wedge  \neg c1) \vee (c2 \wedge  \neg c1) \vee ( \neg c5 \wedge  \neg c7))$ &
  $68.46$ &
  $90.18$ \\
 &
  $( \neg c0 \wedge  \neg c2 \wedge  \neg c6 \wedge  \neg c8)$ &
  $90.18$ &
  $( \neg c5 \wedge (c4 \vee  \neg c9))$ &
  $59.35$ &
  $68.27$ \\
 &
  $(c5 \wedge  \neg c4)$ &
  $58.18$ &
  $(c0 \vee c2 \vee c4 \vee c6)$ &
  $90.26$ &
  $90.26$ \\
 &
  $( \neg c2 \wedge  \neg c8 \wedge (c1 \vee  \neg c0) \wedge (c9 \vee  \neg c4))$ &
  $39.12$ &
  $(c0 \vee c6 \vee (c8 \wedge  \neg c7))$ &
  $79.86$ &
  $79.86$ \\
 &
  $( \neg c0 \vee  \neg c6)$ &
  $29.88$ &
  $( \neg c1 \wedge  \neg c3 \wedge (c6 \vee  \neg c9) \wedge ( \neg c7 \vee  \neg c9))$ &
  $59.35$ &
  $91.08$ \\
 &
  $( \neg c0 \wedge  \neg c2 \wedge  \neg c6 \wedge  \neg c8)$ &
  $90.18$ &
  $( \neg c1 \wedge  \neg c3 \wedge (c2 \vee  \neg c9))$ &
  $59.35$ &
  $80.80$ \\ \hline
\multirow{10}{*}{Decision tree} &
  $(h4  \leq  0.50 \wedge h0  \leq  0.50 \wedge h9  \leq  0.50 \wedge h3  \leq  0.50 \wedge h7  \leq  0.50 \wedge h2  \leq  0.50 \wedge h8  \leq  0.50 \wedge h6  \leq  0.50 \wedge h5  \leq  0.50) \vee (h4  \leq  0.50 \wedge h0  \leq  0.50 \wedge h9  \leq  0.50 \wedge h3  \leq  0.50 \wedge h7  \leq  0.50 \wedge h2  \leq  0.50 \wedge h8  \leq  0.50 \wedge h6  \leq  0.50 \wedge h5 > 0.50) \vee (h4  \leq  0.50 \wedge h0  \leq  0.50 \wedge h9  \leq  0.50 \wedge h3  \leq  0.50 \wedge h7  \leq  0.50 \wedge h2  \leq  0.50 \wedge h8  \leq  0.50 \wedge h6 > 0.50) \vee (h4  \leq  0.50 \wedge h0  \leq  0.50 \wedge h9  \leq  0.50 \wedge h3  \leq  0.50 \wedge h7  \leq  0.50 \wedge h2  \leq  0.50 \wedge h8 > 0.50) \vee (h4  \leq  0.50 \wedge h0  \leq  0.50 \wedge h9  \leq  0.50 \wedge h3  \leq  0.50 \wedge h7  \leq  0.50 \wedge h2 > 0.50)$ &
  $97.95$ &
  $(h4  \leq  0.50 \wedge h0  \leq  0.50 \wedge h9  \leq  0.50 \wedge h3  \leq  0.50 \wedge h7 > 0.50) \vee (h4  \leq  0.50 \wedge h0  \leq  0.50 \wedge h9  \leq  0.50 \wedge h3 > 0.50) \vee (h4  \leq  0.50 \wedge h0  \leq  0.50 \wedge h9 > 0.50) \vee (h4  \leq  0.50 \wedge h0 > 0.50) \vee (h4 > 0.50)$ &
  $97.95$ &
  $97.95$ \\
 &
  $(h4  \leq  0.50 \wedge h0  \leq  0.50 \wedge h9  \leq  0.50 \wedge h3  \leq  0.50 \wedge h7  \leq  0.50 \wedge h2  \leq  0.50 \wedge h8  \leq  0.50 \wedge h6  \leq  0.50 \wedge h1  \leq  0.50) \vee (h4  \leq  0.50 \wedge h0  \leq  0.50 \wedge h9  \leq  0.50 \wedge h3  \leq  0.50 \wedge h7  \leq  0.50 \wedge h2  \leq  0.50 \wedge h8  \leq  0.50 \wedge h6  \leq  0.50 \wedge h1 > 0.50) \vee (h4  \leq  0.50 \wedge h0  \leq  0.50 \wedge h9  \leq  0.50 \wedge h3  \leq  0.50 \wedge h7  \leq  0.50 \wedge h2  \leq  0.50 \wedge h8  \leq  0.50 \wedge h6 > 0.50) \vee (h4  \leq  0.50 \wedge h0  \leq  0.50 \wedge h9  \leq  0.50 \wedge h3  \leq  0.50 \wedge h7  \leq  0.50 \wedge h2  \leq  0.50 \wedge h8 > 0.50) \vee (h4  \leq  0.50 \wedge h0  \leq  0.50 \wedge h9  \leq  0.50 \wedge h3  \leq  0.50 \wedge h7  \leq  0.50 \wedge h2 > 0.50)$ &
  $97.95$ &
  $(h4  \leq  0.50 \wedge h0  \leq  0.50 \wedge h9  \leq  0.50 \wedge h3  \leq  0.50 \wedge h7 > 0.50) \vee (h4  \leq  0.50 \wedge h0  \leq  0.50 \wedge h9  \leq  0.50 \wedge h3 > 0.50) \vee (h4  \leq  0.50 \wedge h0  \leq  0.50 \wedge h9 > 0.50) \vee (h4  \leq  0.50 \wedge h0 > 0.50) \vee (h4 > 0.50)$ &
  $97.95$ &
  $97.95$ \\
 &
  $(h4  \leq  0.50 \wedge h0  \leq  0.50 \wedge h9  \leq  0.50 \wedge h3  \leq  0.50 \wedge h7  \leq  0.50 \wedge h2  \leq  0.50 \wedge h8  \leq  0.50 \wedge h6  \leq  0.50 \wedge h1  \leq  0.50) \vee (h4  \leq  0.50 \wedge h0  \leq  0.50 \wedge h9  \leq  0.50 \wedge h3  \leq  0.50 \wedge h7  \leq  0.50 \wedge h2  \leq  0.50 \wedge h8  \leq  0.50 \wedge h6  \leq  0.50 \wedge h1 > 0.50) \vee (h4  \leq  0.50 \wedge h0  \leq  0.50 \wedge h9  \leq  0.50 \wedge h3  \leq  0.50 \wedge h7  \leq  0.50 \wedge h2  \leq  0.50 \wedge h8  \leq  0.50 \wedge h6 > 0.50) \vee (h4  \leq  0.50 \wedge h0  \leq  0.50 \wedge h9  \leq  0.50 \wedge h3  \leq  0.50 \wedge h7  \leq  0.50 \wedge h2  \leq  0.50 \wedge h8 > 0.50) \vee (h4  \leq  0.50 \wedge h0  \leq  0.50 \wedge h9  \leq  0.50 \wedge h3  \leq  0.50 \wedge h7  \leq  0.50 \wedge h2 > 0.50)$ &
  $97.95$ &
  $(h4  \leq  0.50 \wedge h0  \leq  0.50 \wedge h9  \leq  0.50 \wedge h3  \leq  0.50 \wedge h7 > 0.50) \vee (h4  \leq  0.50 \wedge h0  \leq  0.50 \wedge h9  \leq  0.50 \wedge h3 > 0.50) \vee (h4  \leq  0.50 \wedge h0  \leq  0.50 \wedge h9 > 0.50) \vee (h4  \leq  0.50 \wedge h0 > 0.50) \vee (h4 > 0.50)$ &
  $97.95$ &
  $97.95$ \\
 &
  $(h4  \leq  0.50 \wedge h0  \leq  0.50 \wedge h9  \leq  0.50 \wedge h3  \leq  0.50 \wedge h7  \leq  0.50 \wedge h2  \leq  0.50 \wedge h8  \leq  0.50 \wedge h6  \leq  0.50 \wedge h5  \leq  0.50) \vee (h4  \leq  0.50 \wedge h0  \leq  0.50 \wedge h9  \leq  0.50 \wedge h3  \leq  0.50 \wedge h7  \leq  0.50 \wedge h2  \leq  0.50 \wedge h8  \leq  0.50 \wedge h6  \leq  0.50 \wedge h5 > 0.50) \vee (h4  \leq  0.50 \wedge h0  \leq  0.50 \wedge h9  \leq  0.50 \wedge h3  \leq  0.50 \wedge h7  \leq  0.50 \wedge h2  \leq  0.50 \wedge h8  \leq  0.50 \wedge h6 > 0.50) \vee (h4  \leq  0.50 \wedge h0  \leq  0.50 \wedge h9  \leq  0.50 \wedge h3  \leq  0.50 \wedge h7  \leq  0.50 \wedge h2  \leq  0.50 \wedge h8 > 0.50) \vee (h4  \leq  0.50 \wedge h0  \leq  0.50 \wedge h9  \leq  0.50 \wedge h3  \leq  0.50 \wedge h7  \leq  0.50 \wedge h2 > 0.50)$ &
  $97.95$ &
  $(h4  \leq  0.50 \wedge h0  \leq  0.50 \wedge h9  \leq  0.50 \wedge h3  \leq  0.50 \wedge h7 > 0.50) \vee (h4  \leq  0.50 \wedge h0  \leq  0.50 \wedge h9  \leq  0.50 \wedge h3 > 0.50) \vee (h4  \leq  0.50 \wedge h0  \leq  0.50 \wedge h9 > 0.50) \vee (h4  \leq  0.50 \wedge h0 > 0.50) \vee (h4 > 0.50)$ &
  $97.95$ &
  $97.95$ \\
 &
  $(h4  \leq  0.50 \wedge h0  \leq  0.50 \wedge h9  \leq  0.50 \wedge h3  \leq  0.50 \wedge h7  \leq  0.50 \wedge h2  \leq  0.50 \wedge h8  \leq  0.50 \wedge h6  \leq  0.50 \wedge h1  \leq  0.50) \vee (h4  \leq  0.50 \wedge h0  \leq  0.50 \wedge h9  \leq  0.50 \wedge h3  \leq  0.50 \wedge h7  \leq  0.50 \wedge h2  \leq  0.50 \wedge h8  \leq  0.50 \wedge h6  \leq  0.50 \wedge h1 > 0.50) \vee (h4  \leq  0.50 \wedge h0  \leq  0.50 \wedge h9  \leq  0.50 \wedge h3  \leq  0.50 \wedge h7  \leq  0.50 \wedge h2  \leq  0.50 \wedge h8  \leq  0.50 \wedge h6 > 0.50) \vee (h4  \leq  0.50 \wedge h0  \leq  0.50 \wedge h9  \leq  0.50 \wedge h3  \leq  0.50 \wedge h7  \leq  0.50 \wedge h2  \leq  0.50 \wedge h8 > 0.50) \vee (h4  \leq  0.50 \wedge h0  \leq  0.50 \wedge h9  \leq  0.50 \wedge h3  \leq  0.50 \wedge h7  \leq  0.50 \wedge h2 > 0.50)$ &
  $97.95$ &
  $(h4  \leq  0.50 \wedge h0  \leq  0.50 \wedge h9  \leq  0.50 \wedge h3  \leq  0.50 \wedge h7 > 0.50) \vee (h4  \leq  0.50 \wedge h0  \leq  0.50 \wedge h9  \leq  0.50 \wedge h3 > 0.50) \vee (h4  \leq  0.50 \wedge h0  \leq  0.50 \wedge h9 > 0.50) \vee (h4  \leq  0.50 \wedge h0 > 0.50) \vee (h4 > 0.50)$ &
  $97.95$ &
  $97.95$ \\
 &
  $(h4  \leq  0.50 \wedge h0  \leq  0.50 \wedge h9  \leq  0.50 \wedge h3  \leq  0.50 \wedge h7  \leq  0.50 \wedge h2  \leq  0.50 \wedge h8  \leq  0.50 \wedge h6  \leq  0.50 \wedge h1  \leq  0.50) \vee (h4  \leq  0.50 \wedge h0  \leq  0.50 \wedge h9  \leq  0.50 \wedge h3  \leq  0.50 \wedge h7  \leq  0.50 \wedge h2  \leq  0.50 \wedge h8  \leq  0.50 \wedge h6  \leq  0.50 \wedge h1 > 0.50) \vee (h4  \leq  0.50 \wedge h0  \leq  0.50 \wedge h9  \leq  0.50 \wedge h3  \leq  0.50 \wedge h7  \leq  0.50 \wedge h2  \leq  0.50 \wedge h8  \leq  0.50 \wedge h6 > 0.50) \vee (h4  \leq  0.50 \wedge h0  \leq  0.50 \wedge h9  \leq  0.50 \wedge h3  \leq  0.50 \wedge h7  \leq  0.50 \wedge h2  \leq  0.50 \wedge h8 > 0.50) \vee (h4  \leq  0.50 \wedge h0  \leq  0.50 \wedge h9  \leq  0.50 \wedge h3  \leq  0.50 \wedge h7  \leq  0.50 \wedge h2 > 0.50)$ &
  $97.95$ &
  $(h4  \leq  0.50 \wedge h0  \leq  0.50 \wedge h9  \leq  0.50 \wedge h3  \leq  0.50 \wedge h7 > 0.50) \vee (h4  \leq  0.50 \wedge h0  \leq  0.50 \wedge h9  \leq  0.50 \wedge h3 > 0.50) \vee (h4  \leq  0.50 \wedge h0  \leq  0.50 \wedge h9 > 0.50) \vee (h4  \leq  0.50 \wedge h0 > 0.50) \vee (h4 > 0.50)$ &
  $97.95$ &
  $97.95$ \\
 &
  $(h4  \leq  0.50 \wedge h0  \leq  0.50 \wedge h9  \leq  0.50 \wedge h3  \leq  0.50 \wedge h7  \leq  0.50 \wedge h2  \leq  0.50 \wedge h8  \leq  0.50 \wedge h6  \leq  0.50 \wedge h5  \leq  0.50) \vee (h4  \leq  0.50 \wedge h0  \leq  0.50 \wedge h9  \leq  0.50 \wedge h3  \leq  0.50 \wedge h7  \leq  0.50 \wedge h2  \leq  0.50 \wedge h8  \leq  0.50 \wedge h6  \leq  0.50 \wedge h5 > 0.50) \vee (h4  \leq  0.50 \wedge h0  \leq  0.50 \wedge h9  \leq  0.50 \wedge h3  \leq  0.50 \wedge h7  \leq  0.50 \wedge h2  \leq  0.50 \wedge h8  \leq  0.50 \wedge h6 > 0.50) \vee (h4  \leq  0.50 \wedge h0  \leq  0.50 \wedge h9  \leq  0.50 \wedge h3  \leq  0.50 \wedge h7  \leq  0.50 \wedge h2  \leq  0.50 \wedge h8 > 0.50) \vee (h4  \leq  0.50 \wedge h0  \leq  0.50 \wedge h9  \leq  0.50 \wedge h3  \leq  0.50 \wedge h7  \leq  0.50 \wedge h2 > 0.50)$ &
  $97.95$ &
  $(h4  \leq  0.50 \wedge h0  \leq  0.50 \wedge h9  \leq  0.50 \wedge h3  \leq  0.50 \wedge h7 > 0.50) \vee (h4  \leq  0.50 \wedge h0  \leq  0.50 \wedge h9  \leq  0.50 \wedge h3 > 0.50) \vee (h4  \leq  0.50 \wedge h0  \leq  0.50 \wedge h9 > 0.50) \vee (h4  \leq  0.50 \wedge h0 > 0.50) \vee (h4 > 0.50)$ &
  $97.95$ &
  $97.95$ \\
 &
  $(h4  \leq  0.50 \wedge h0  \leq  0.50 \wedge h9  \leq  0.50 \wedge h3  \leq  0.50 \wedge h7  \leq  0.50 \wedge h2  \leq  0.50 \wedge h8  \leq  0.50 \wedge h6  \leq  0.50 \wedge h5  \leq  0.50) \vee (h4  \leq  0.50 \wedge h0  \leq  0.50 \wedge h9  \leq  0.50 \wedge h3  \leq  0.50 \wedge h7  \leq  0.50 \wedge h2  \leq  0.50 \wedge h8  \leq  0.50 \wedge h6  \leq  0.50 \wedge h5 > 0.50) \vee (h4  \leq  0.50 \wedge h0  \leq  0.50 \wedge h9  \leq  0.50 \wedge h3  \leq  0.50 \wedge h7  \leq  0.50 \wedge h2  \leq  0.50 \wedge h8  \leq  0.50 \wedge h6 > 0.50) \vee (h4  \leq  0.50 \wedge h0  \leq  0.50 \wedge h9  \leq  0.50 \wedge h3  \leq  0.50 \wedge h7  \leq  0.50 \wedge h2  \leq  0.50 \wedge h8 > 0.50) \vee (h4  \leq  0.50 \wedge h0  \leq  0.50 \wedge h9  \leq  0.50 \wedge h3  \leq  0.50 \wedge h7  \leq  0.50 \wedge h2 > 0.50)$ &
  $97.95$ &
  $(h4  \leq  0.50 \wedge h0  \leq  0.50 \wedge h9  \leq  0.50 \wedge h3  \leq  0.50 \wedge h7 > 0.50) \vee (h4  \leq  0.50 \wedge h0  \leq  0.50 \wedge h9  \leq  0.50 \wedge h3 > 0.50) \vee (h4  \leq  0.50 \wedge h0  \leq  0.50 \wedge h9 > 0.50) \vee (h4  \leq  0.50 \wedge h0 > 0.50) \vee (h4 > 0.50)$ &
  $97.95$ &
  $97.95$ \\
 &
  $(h4  \leq  0.50 \wedge h0  \leq  0.50 \wedge h9  \leq  0.50 \wedge h3  \leq  0.50 \wedge h7  \leq  0.50 \wedge h2  \leq  0.50 \wedge h8  \leq  0.50 \wedge h6  \leq  0.50 \wedge h1  \leq  0.50) \vee (h4  \leq  0.50 \wedge h0  \leq  0.50 \wedge h9  \leq  0.50 \wedge h3  \leq  0.50 \wedge h7  \leq  0.50 \wedge h2  \leq  0.50 \wedge h8  \leq  0.50 \wedge h6  \leq  0.50 \wedge h1 > 0.50) \vee (h4  \leq  0.50 \wedge h0  \leq  0.50 \wedge h9  \leq  0.50 \wedge h3  \leq  0.50 \wedge h7  \leq  0.50 \wedge h2  \leq  0.50 \wedge h8  \leq  0.50 \wedge h6 > 0.50) \vee (h4  \leq  0.50 \wedge h0  \leq  0.50 \wedge h9  \leq  0.50 \wedge h3  \leq  0.50 \wedge h7  \leq  0.50 \wedge h2  \leq  0.50 \wedge h8 > 0.50) \vee (h4  \leq  0.50 \wedge h0  \leq  0.50 \wedge h9  \leq  0.50 \wedge h3  \leq  0.50 \wedge h7  \leq  0.50 \wedge h2 > 0.50)$ &
  $97.95$ &
  $(h4  \leq  0.50 \wedge h0  \leq  0.50 \wedge h9  \leq  0.50 \wedge h3  \leq  0.50 \wedge h7 > 0.50) \vee (h4  \leq  0.50 \wedge h0  \leq  0.50 \wedge h9  \leq  0.50 \wedge h3 > 0.50) \vee (h4  \leq  0.50 \wedge h0  \leq  0.50 \wedge h9 > 0.50) \vee (h4  \leq  0.50 \wedge h0 > 0.50) \vee (h4 > 0.50)$ &
  $97.95$ &
  $97.95$ \\
 &
  $(h4  \leq  0.50 \wedge h0  \leq  0.50 \wedge h9  \leq  0.50 \wedge h3  \leq  0.50 \wedge h7  \leq  0.50 \wedge h2  \leq  0.50 \wedge h8  \leq  0.50 \wedge h6  \leq  0.50 \wedge h1  \leq  0.50) \vee (h4  \leq  0.50 \wedge h0  \leq  0.50 \wedge h9  \leq  0.50 \wedge h3  \leq  0.50 \wedge h7  \leq  0.50 \wedge h2  \leq  0.50 \wedge h8  \leq  0.50 \wedge h6  \leq  0.50 \wedge h1 > 0.50) \vee (h4  \leq  0.50 \wedge h0  \leq  0.50 \wedge h9  \leq  0.50 \wedge h3  \leq  0.50 \wedge h7  \leq  0.50 \wedge h2  \leq  0.50 \wedge h8  \leq  0.50 \wedge h6 > 0.50) \vee (h4  \leq  0.50 \wedge h0  \leq  0.50 \wedge h9  \leq  0.50 \wedge h3  \leq  0.50 \wedge h7  \leq  0.50 \wedge h2  \leq  0.50 \wedge h8 > 0.50) \vee (h4  \leq  0.50 \wedge h0  \leq  0.50 \wedge h9  \leq  0.50 \wedge h3  \leq  0.50 \wedge h7  \leq  0.50 \wedge h2 > 0.50)$ &
  $97.95$ &
  $(h4  \leq  0.50 \wedge h0  \leq  0.50 \wedge h9  \leq  0.50 \wedge h3  \leq  0.50 \wedge h7 > 0.50) \vee (h4  \leq  0.50 \wedge h0  \leq  0.50 \wedge h9  \leq  0.50 \wedge h3 > 0.50) \vee (h4  \leq  0.50 \wedge h0  \leq  0.50 \wedge h9 > 0.50) \vee (h4  \leq  0.50 \wedge h0 > 0.50) \vee (h4 > 0.50)$ &
  $97.95$ &
  $97.95$ \\ \hline
\multirow{10}{*}{ReLU} &
  $c1 \vee c5 \vee c9 \vee ( \neg c0 \wedge  \neg c2 \wedge  \neg c4 \wedge  \neg c6 \wedge  \neg c8)$ &
  $69.64$ &
  $c0 \vee c2 \vee c4 \vee c6 \vee c8$ &
  $100.00$ &
  $100.00$ \\
 &
  $c1 \vee c3 \vee c5 \vee c7 \vee c9$ &
  $100.00$ &
  $ \neg c3$ &
  $59.36$ &
  $100.00$ \\
 &
  $c1 \vee c3 \vee c5 \vee c7 \vee c9$ &
  $100.00$ &
  $ \neg c1 \wedge  \neg c3 \wedge  \neg c5 \wedge  \neg c7 \wedge  \neg c9$ &
  $100.00$ &
  $100.00$ \\
 &
  $c9 \vee ( \neg c0 \wedge  \neg c2 \wedge  \neg c4 \wedge  \neg c6 \wedge  \neg c8)$ &
  $89.91$ &
  $c0 \vee c2 \vee c4 \vee c6 \vee c8$ &
  $100.00$ &
  $100.00$ \\
 &
  $c1 \vee c3 \vee c5 \vee c7 \vee c9$ &
  $100.00$ &
  $c0 \vee ( \neg c1 \wedge  \neg c3 \wedge  \neg c5 \wedge  \neg c7 \wedge  \neg c9)$ &
  $100.00$ &
  $100.00$ \\
 &
  $c1 \vee c3 \vee c5 \vee c7 \vee c9$ &
  $100.00$ &
  $ \neg c1 \wedge  \neg c3 \wedge  \neg c5 \wedge  \neg c7 \wedge  \neg c9$ &
  $100.00$ &
  $100.00$ \\
 &
  $c1 \vee c3 \vee c5 \vee c7 \vee c9$ &
  $100.00$ &
  $ \neg c1 \wedge  \neg c3 \wedge  \neg c5 \wedge  \neg c7 \wedge  \neg c9$ &
  $100.00$ &
  $100.00$ \\
 &
  $( \neg c0 \wedge  \neg c2 \wedge  \neg c7 \wedge  \neg c8) \vee ( \neg c0 \wedge  \neg c2 \wedge  \neg c4 \wedge  \neg c6 \wedge  \neg c8)$ &
  $40.14$ &
  $c0 \vee c2 \vee c4 \vee c6 \vee c8$ &
  $100.00$ &
  $100.00$ \\
 &
  $ \neg c0 \wedge  \neg c2 \wedge  \neg c4 \wedge  \neg c6 \wedge  \neg c8$ &
  $100.00$ &
  $c0 \vee c2 \vee c4 \vee c6 \vee c8$ &
  $100.00$ &
  $100.00$ \\
 &
  $c1 \vee c3 \vee c5 \vee c7 \vee c9$ &
  $100.00$ &
  $ \neg c1 \wedge  \neg c3 \wedge  \neg c5 \wedge  \neg c7 \wedge  \neg c9$ &
  $100.00$ &
  $100.00$ \\ \hline
\end{tabular}%
}
\end{table}

% Please add the following required packages to your document preamble:
% \usepackage{multirow}
% \usepackage{graphicx}
\begin{table}[]
\centering
\caption{MNIST (hidden) explanations}
\label{tab:my-table}
\resizebox{\textwidth}{!}{%
\begin{tabular}{c|p{10cm}|l|p{10cm}|ll}
\hline
\multirow{2}{*}{\textbf{Method}} &
  \multicolumn{2}{c}{\textbf{Positive explanation}} &
  \multicolumn{2}{c}{\textbf{Negative explanation}} &
  \multicolumn{1}{c}{\multirow{2}{*}{\textbf{Model's accuracy}}} \\
 &
  \textbf{Formula} &
  \textbf{Accuracy (\%)} &
  \textbf{Formula} &
  \textbf{Accuracy (\%)} &
  \multicolumn{1}{c}{} \\ \hline
\multirow{10}{*}{Pruning} &
  $ \neg h1 \wedge  \neg h3 \wedge  \neg h6 \wedge  \neg h9$ &
  $99.28$ &
  $h1 \vee h3 \vee h6 \vee h9$ &
  $99.28$ &
  $99.28$ \\
 &
  $ \neg h1 \wedge  \neg h3 \wedge  \neg h6 \wedge  \neg h9$ &
  $99.28$ &
  $h1 \vee h3 \vee h6 \vee h9$ &
  $99.28$ &
  $99.28$ \\
 &
  $ \neg h1 \wedge  \neg h3 \wedge  \neg h6 \wedge  \neg h9$ &
  $99.28$ &
  $h1 \vee h3 \vee h6 \vee h9$ &
  $99.28$ &
  $99.28$ \\
 &
  $ \neg h1 \wedge  \neg h3 \wedge  \neg h6 \wedge  \neg h9$ &
  $99.28$ &
  $h1 \vee h3 \vee h6 \vee h9$ &
  $99.28$ &
  $99.28$ \\
 &
  $ \neg h1 \wedge  \neg h3 \wedge  \neg h6 \wedge  \neg h9$ &
  $99.28$ &
  $h1 \vee h3 \vee h6 \vee h9$ &
  $99.28$ &
  $99.28$ \\
 &
  $ \neg h1 \wedge  \neg h3 \wedge  \neg h6 \wedge  \neg h9$ &
  $99.28$ &
  $h1 \vee h3 \vee h6 \vee h9$ &
  $99.28$ &
  $99.28$ \\
 &
  $ \neg h1 \wedge  \neg h3 \wedge  \neg h6 \wedge  \neg h9$ &
  $99.28$ &
  $h1 \vee h3 \vee h6 \vee h9$ &
  $99.28$ &
  $99.28$ \\
 &
  $ \neg h1 \wedge  \neg h3 \wedge  \neg h6 \wedge  \neg h9$ &
  $99.28$ &
  $h1 \vee h3 \vee h6 \vee h9$ &
  $99.28$ &
  $99.28$ \\
 &
  $ \neg h1 \wedge  \neg h3 \wedge  \neg h6 \wedge  \neg h9$ &
  $99.28$ &
  $h1 \vee h3 \vee h6 \vee h9$ &
  $99.28$ &
  $99.28$ \\
 &
  $ \neg h1 \wedge  \neg h3 \wedge  \neg h6 \wedge  \neg h9$ &
  $99.28$ &
  $h1 \vee h3 \vee h6 \vee h9$ &
  $99.28$ &
  $99.28$ \\ \hline
\multirow{10}{*}{$\psi$ net} &
  $(h0 \vee h2 \vee  \neg h1)$ &
  $52.02$ &
  $( \neg h4 \wedge  \neg h5 \wedge (h6 \vee  \neg h7))$ &
  $56.63$ &
  $71.43$ \\
 &
  $((h2 \vee h5) \wedge (h2 \vee  \neg h1) \wedge (h5 \vee  \neg h3) \wedge ( \neg h1 \vee  \neg h3))$ &
  $28.47$ &
  $( \neg h4 \wedge  \neg h5 \wedge (h1 \vee h3))$ &
  $78.74$ &
  $78.74$ \\
 &
  $( \neg h1 \wedge (h2 \vee  \neg h9) \wedge (h0 \vee h7 \vee  \neg h6))$ &
  $30.72$ &
  $( \neg h0 \wedge  \neg h2 \wedge  \neg h5 \wedge  \neg h7)$ &
  $84.57$ &
  $84.57$ \\
 &
  $((h2 \wedge h5) \vee (h2 \wedge  \neg h3) \vee (h2 \wedge  \neg h9) \vee (h5 \wedge  \neg h3) \vee (h7 \wedge  \neg h6) \vee ( \neg h3 \wedge  \neg h9))$ &
  $40.02$ &
  $(h1 \vee h3 \vee h6 \vee h9)$ &
  $99.28$ &
  $99.28$ \\
 &
  $( \neg h1 \wedge  \neg h6 \wedge (h2 \vee h7))$ &
  $72.44$ &
  $(h1 \vee h9 \vee (h3 \wedge  \neg h2 \wedge  \neg h5))$ &
  $92.42$ &
  $92.42$ \\
 &
  $(h2 \wedge  \neg h6 \wedge  \neg h9)$ &
  $65.07$ &
  $(h9 \wedge  \neg h5 \wedge  \neg h7)$ &
  $64.42$ &
  $75.13$ \\
 &
  $(h0 \vee h2 \vee h5)$ &
  $77.20$ &
  $(h6 \vee (h3 \wedge  \neg h2 \wedge  \neg h4))$ &
  $64.81$ &
  $71.44$ \\
 &
  $(h2 \wedge  \neg h3)$ &
  $65.07$ &
  $(h3 \vee h6)$ &
  $64.81$ &
  $64.81$ \\
 &
  $((h2 \vee  \neg h9) \wedge (h4 \vee  \neg h6) \wedge (h5 \vee  \neg h1))$ &
  $40.92$ &
  $((h9 \vee  \neg h0) \wedge (h9 \vee  \neg h5) \wedge (h3 \vee h6 \vee h9) \wedge ( \neg h0 \vee  \neg h7) \wedge ( \neg h5 \vee  \neg h7) \wedge (h3 \vee h6 \vee  \neg h7))$ &
  $56.63$ &
  $78.49$ \\
 &
  $( \neg h1 \wedge  \neg h3 \wedge (h2 \vee  \neg h9))$ &
  $48.61$ &
  $( \neg h4)$ &
  $55.63$ &
  $75.14$ \\ \hline
\multirow{10}{*}{Decision tree} &
  $(h1  \leq  0.50 \wedge h9  \leq  0.50 \wedge h3  \leq  0.50 \wedge h6  \leq  0.50 \wedge h8  \leq  0.50 \wedge h2  \leq  0.50 \wedge h7  \leq  0.50) \vee (h1  \leq  0.50 \wedge h9  \leq  0.50 \wedge h3  \leq  0.50 \wedge h6  \leq  0.50 \wedge h8  \leq  0.50 \wedge h2  \leq  0.50 \wedge h7 > 0.50) \vee (h1  \leq  0.50 \wedge h9  \leq  0.50 \wedge h3  \leq  0.50 \wedge h6  \leq  0.50 \wedge h8  \leq  0.50 \wedge h2 > 0.50) \vee (h1  \leq  0.50 \wedge h9  \leq  0.50 \wedge h3  \leq  0.50 \wedge h6  \leq  0.50 \wedge h8 > 0.50)$ &
  $99.28$ &
  $(h1  \leq  0.50 \wedge h9  \leq  0.50 \wedge h3  \leq  0.50 \wedge h6 > 0.50) \vee (h1  \leq  0.50 \wedge h9  \leq  0.50 \wedge h3 > 0.50) \vee (h1  \leq  0.50 \wedge h9 > 0.50) \vee (h1 > 0.50)$ &
  $99.28$ &
  $99.28$ \\
 &
  $(h1  \leq  0.50 \wedge h9  \leq  0.50 \wedge h3  \leq  0.50 \wedge h6  \leq  0.50 \wedge h8  \leq  0.50 \wedge h2  \leq  0.50 \wedge h7  \leq  0.50) \vee (h1  \leq  0.50 \wedge h9  \leq  0.50 \wedge h3  \leq  0.50 \wedge h6  \leq  0.50 \wedge h8  \leq  0.50 \wedge h2  \leq  0.50 \wedge h7 > 0.50) \vee (h1  \leq  0.50 \wedge h9  \leq  0.50 \wedge h3  \leq  0.50 \wedge h6  \leq  0.50 \wedge h8  \leq  0.50 \wedge h2 > 0.50) \vee (h1  \leq  0.50 \wedge h9  \leq  0.50 \wedge h3  \leq  0.50 \wedge h6  \leq  0.50 \wedge h8 > 0.50)$ &
  $99.28$ &
  $(h1  \leq  0.50 \wedge h9  \leq  0.50 \wedge h3  \leq  0.50 \wedge h6 > 0.50) \vee (h1  \leq  0.50 \wedge h9  \leq  0.50 \wedge h3 > 0.50) \vee (h1  \leq  0.50 \wedge h9 > 0.50) \vee (h1 > 0.50)$ &
  $99.28$ &
  $99.28$ \\
 &
  $(h1  \leq  0.50 \wedge h9  \leq  0.50 \wedge h3  \leq  0.50 \wedge h6  \leq  0.50 \wedge h8  \leq  0.50 \wedge h2  \leq  0.50 \wedge h7  \leq  0.50) \vee (h1  \leq  0.50 \wedge h9  \leq  0.50 \wedge h3  \leq  0.50 \wedge h6  \leq  0.50 \wedge h8  \leq  0.50 \wedge h2  \leq  0.50 \wedge h7 > 0.50) \vee (h1  \leq  0.50 \wedge h9  \leq  0.50 \wedge h3  \leq  0.50 \wedge h6  \leq  0.50 \wedge h8  \leq  0.50 \wedge h2 > 0.50) \vee (h1  \leq  0.50 \wedge h9  \leq  0.50 \wedge h3  \leq  0.50 \wedge h6  \leq  0.50 \wedge h8 > 0.50)$ &
  $99.28$ &
  $(h1  \leq  0.50 \wedge h9  \leq  0.50 \wedge h3  \leq  0.50 \wedge h6 > 0.50) \vee (h1  \leq  0.50 \wedge h9  \leq  0.50 \wedge h3 > 0.50) \vee (h1  \leq  0.50 \wedge h9 > 0.50) \vee (h1 > 0.50)$ &
  $99.28$ &
  $99.28$ \\
 &
  $(h1  \leq  0.50 \wedge h9  \leq  0.50 \wedge h3  \leq  0.50 \wedge h6  \leq  0.50 \wedge h8  \leq  0.50 \wedge h2  \leq  0.50 \wedge h7  \leq  0.50) \vee (h1  \leq  0.50 \wedge h9  \leq  0.50 \wedge h3  \leq  0.50 \wedge h6  \leq  0.50 \wedge h8  \leq  0.50 \wedge h2  \leq  0.50 \wedge h7 > 0.50) \vee (h1  \leq  0.50 \wedge h9  \leq  0.50 \wedge h3  \leq  0.50 \wedge h6  \leq  0.50 \wedge h8  \leq  0.50 \wedge h2 > 0.50) \vee (h1  \leq  0.50 \wedge h9  \leq  0.50 \wedge h3  \leq  0.50 \wedge h6  \leq  0.50 \wedge h8 > 0.50)$ &
  $99.28$ &
  $(h1  \leq  0.50 \wedge h9  \leq  0.50 \wedge h3  \leq  0.50 \wedge h6 > 0.50) \vee (h1  \leq  0.50 \wedge h9  \leq  0.50 \wedge h3 > 0.50) \vee (h1  \leq  0.50 \wedge h9 > 0.50) \vee (h1 > 0.50)$ &
  $99.28$ &
  $99.28$ \\
 &
  $(h1  \leq  0.50 \wedge h9  \leq  0.50 \wedge h3  \leq  0.50 \wedge h6  \leq  0.50 \wedge h8  \leq  0.50 \wedge h2  \leq  0.50 \wedge h7  \leq  0.50) \vee (h1  \leq  0.50 \wedge h9  \leq  0.50 \wedge h3  \leq  0.50 \wedge h6  \leq  0.50 \wedge h8  \leq  0.50 \wedge h2  \leq  0.50 \wedge h7 > 0.50) \vee (h1  \leq  0.50 \wedge h9  \leq  0.50 \wedge h3  \leq  0.50 \wedge h6  \leq  0.50 \wedge h8  \leq  0.50 \wedge h2 > 0.50) \vee (h1  \leq  0.50 \wedge h9  \leq  0.50 \wedge h3  \leq  0.50 \wedge h6  \leq  0.50 \wedge h8 > 0.50)$ &
  $99.28$ &
  $(h1  \leq  0.50 \wedge h9  \leq  0.50 \wedge h3  \leq  0.50 \wedge h6 > 0.50) \vee (h1  \leq  0.50 \wedge h9  \leq  0.50 \wedge h3 > 0.50) \vee (h1  \leq  0.50 \wedge h9 > 0.50) \vee (h1 > 0.50)$ &
  $99.28$ &
  $99.28$ \\
 &
  $(h1  \leq  0.50 \wedge h9  \leq  0.50 \wedge h3  \leq  0.50 \wedge h6  \leq  0.50 \wedge h8  \leq  0.50 \wedge h2  \leq  0.50 \wedge h7  \leq  0.50) \vee (h1  \leq  0.50 \wedge h9  \leq  0.50 \wedge h3  \leq  0.50 \wedge h6  \leq  0.50 \wedge h8  \leq  0.50 \wedge h2  \leq  0.50 \wedge h7 > 0.50) \vee (h1  \leq  0.50 \wedge h9  \leq  0.50 \wedge h3  \leq  0.50 \wedge h6  \leq  0.50 \wedge h8  \leq  0.50 \wedge h2 > 0.50) \vee (h1  \leq  0.50 \wedge h9  \leq  0.50 \wedge h3  \leq  0.50 \wedge h6  \leq  0.50 \wedge h8 > 0.50)$ &
  $99.28$ &
  $(h1  \leq  0.50 \wedge h9  \leq  0.50 \wedge h3  \leq  0.50 \wedge h6 > 0.50) \vee (h1  \leq  0.50 \wedge h9  \leq  0.50 \wedge h3 > 0.50) \vee (h1  \leq  0.50 \wedge h9 > 0.50) \vee (h1 > 0.50)$ &
  $99.28$ &
  $99.28$ \\
 &
  $(h1  \leq  0.50 \wedge h9  \leq  0.50 \wedge h3  \leq  0.50 \wedge h6  \leq  0.50 \wedge h8  \leq  0.50 \wedge h2  \leq  0.50 \wedge h7  \leq  0.50) \vee (h1  \leq  0.50 \wedge h9  \leq  0.50 \wedge h3  \leq  0.50 \wedge h6  \leq  0.50 \wedge h8  \leq  0.50 \wedge h2  \leq  0.50 \wedge h7 > 0.50) \vee (h1  \leq  0.50 \wedge h9  \leq  0.50 \wedge h3  \leq  0.50 \wedge h6  \leq  0.50 \wedge h8  \leq  0.50 \wedge h2 > 0.50) \vee (h1  \leq  0.50 \wedge h9  \leq  0.50 \wedge h3  \leq  0.50 \wedge h6  \leq  0.50 \wedge h8 > 0.50)$ &
  $99.28$ &
  $(h1  \leq  0.50 \wedge h9  \leq  0.50 \wedge h3  \leq  0.50 \wedge h6 > 0.50) \vee (h1  \leq  0.50 \wedge h9  \leq  0.50 \wedge h3 > 0.50) \vee (h1  \leq  0.50 \wedge h9 > 0.50) \vee (h1 > 0.50)$ &
  $99.28$ &
  $99.28$ \\
 &
  $(h1  \leq  0.50 \wedge h9  \leq  0.50 \wedge h3  \leq  0.50 \wedge h6  \leq  0.50 \wedge h8  \leq  0.50 \wedge h2  \leq  0.50 \wedge h7  \leq  0.50) \vee (h1  \leq  0.50 \wedge h9  \leq  0.50 \wedge h3  \leq  0.50 \wedge h6  \leq  0.50 \wedge h8  \leq  0.50 \wedge h2  \leq  0.50 \wedge h7 > 0.50) \vee (h1  \leq  0.50 \wedge h9  \leq  0.50 \wedge h3  \leq  0.50 \wedge h6  \leq  0.50 \wedge h8  \leq  0.50 \wedge h2 > 0.50) \vee (h1  \leq  0.50 \wedge h9  \leq  0.50 \wedge h3  \leq  0.50 \wedge h6  \leq  0.50 \wedge h8 > 0.50)$ &
  $99.28$ &
  $(h1  \leq  0.50 \wedge h9  \leq  0.50 \wedge h3  \leq  0.50 \wedge h6 > 0.50) \vee (h1  \leq  0.50 \wedge h9  \leq  0.50 \wedge h3 > 0.50) \vee (h1  \leq  0.50 \wedge h9 > 0.50) \vee (h1 > 0.50)$ &
  $99.28$ &
  $99.28$ \\
 &
  $(h1  \leq  0.50 \wedge h9  \leq  0.50 \wedge h3  \leq  0.50 \wedge h6  \leq  0.50 \wedge h8  \leq  0.50 \wedge h2  \leq  0.50 \wedge h7  \leq  0.50) \vee (h1  \leq  0.50 \wedge h9  \leq  0.50 \wedge h3  \leq  0.50 \wedge h6  \leq  0.50 \wedge h8  \leq  0.50 \wedge h2  \leq  0.50 \wedge h7 > 0.50) \vee (h1  \leq  0.50 \wedge h9  \leq  0.50 \wedge h3  \leq  0.50 \wedge h6  \leq  0.50 \wedge h8  \leq  0.50 \wedge h2 > 0.50) \vee (h1  \leq  0.50 \wedge h9  \leq  0.50 \wedge h3  \leq  0.50 \wedge h6  \leq  0.50 \wedge h8 > 0.50)$ &
  $99.28$ &
  $(h1  \leq  0.50 \wedge h9  \leq  0.50 \wedge h3  \leq  0.50 \wedge h6 > 0.50) \vee (h1  \leq  0.50 \wedge h9  \leq  0.50 \wedge h3 > 0.50) \vee (h1  \leq  0.50 \wedge h9 > 0.50) \vee (h1 > 0.50)$ &
  $99.28$ &
  $99.28$ \\
 &
  $(h1  \leq  0.50 \wedge h9  \leq  0.50 \wedge h3  \leq  0.50 \wedge h6  \leq  0.50 \wedge h8  \leq  0.50 \wedge h2  \leq  0.50 \wedge h7  \leq  0.50) \vee (h1  \leq  0.50 \wedge h9  \leq  0.50 \wedge h3  \leq  0.50 \wedge h6  \leq  0.50 \wedge h8  \leq  0.50 \wedge h2  \leq  0.50 \wedge h7 > 0.50) \vee (h1  \leq  0.50 \wedge h9  \leq  0.50 \wedge h3  \leq  0.50 \wedge h6  \leq  0.50 \wedge h8  \leq  0.50 \wedge h2 > 0.50) \vee (h1  \leq  0.50 \wedge h9  \leq  0.50 \wedge h3  \leq  0.50 \wedge h6  \leq  0.50 \wedge h8 > 0.50)$ &
  $99.28$ &
  $(h1  \leq  0.50 \wedge h9  \leq  0.50 \wedge h3  \leq  0.50 \wedge h6 > 0.50) \vee (h1  \leq  0.50 \wedge h9  \leq  0.50 \wedge h3 > 0.50) \vee (h1  \leq  0.50 \wedge h9 > 0.50) \vee (h1 > 0.50)$ &
  $99.28$ &
  $99.28$ \\ \hline
\multirow{10}{*}{ReLU} &
  $ \neg h1 \wedge  \neg h3 \wedge  \neg h6 \wedge  \neg h9$ &
  $99.28$ &
  $h1 \vee h3 \vee h6 \vee ( \neg h0 \wedge  \neg h2 \wedge  \neg h4 \wedge  \neg h7 \wedge  \neg h8)$ &
  $90.85$ &
  $99.28$ \\
 &
  $h2 \vee  \neg h6$ &
  $41.79$ &
  $h1 \vee h3 \vee h6 \vee h9$ &
  $99.28$ &
  $99.28$ \\
 &
  $h2 \vee h7 \vee h8 \vee ( \neg h1 \wedge  \neg h3 \wedge  \neg h6 \wedge  \neg h9)$ &
  $67.76$ &
  $h1 \vee h3 \vee h6 \vee h9$ &
  $99.28$ &
  $99.28$ \\
 &
  $ \neg h1 \wedge  \neg h3 \wedge  \neg h6 \wedge  \neg h9$ &
  $99.28$ &
  $h1 \vee h3 \vee h6 \vee h9$ &
  $99.28$ &
  $99.28$ \\
 &
  $( \neg h3 \wedge  \neg h7) \vee ( \neg h1 \wedge  \neg h3 \wedge  \neg h6 \wedge  \neg h9)$ &
  $15.30$ &
  $h1 \vee h3 \vee h6 \vee h9$ &
  $99.28$ &
  $99.28$ \\
 &
  $ \neg h1 \wedge  \neg h3 \wedge  \neg h6 \wedge  \neg h9$ &
  $99.28$ &
  $h1 \vee h3 \vee h6 \vee h9$ &
  $99.28$ &
  $99.28$ \\
 &
  $h2 \vee ( \neg h1 \wedge  \neg h3 \wedge  \neg h6 \wedge  \neg h9)$ &
  $83.47$ &
  $h1 \vee h3 \vee h6 \vee h9$ &
  $99.28$ &
  $99.28$ \\
 &
  $ \neg h1 \wedge  \neg h3 \wedge  \neg h6 \wedge  \neg h9$ &
  $99.28$ &
  $h1 \vee h3 \vee h6 \vee h9$ &
  $99.28$ &
  $99.28$ \\
 &
  $( \neg h0 \wedge  \neg h1 \wedge  \neg h2) \vee ( \neg h1 \wedge  \neg h3 \wedge  \neg h6 \wedge  \neg h9)$ &
  $41.02$ &
  $h1 \vee h3 \vee h6 \vee h9$ &
  $99.28$ &
  $99.28$ \\
 &
  $ \neg h1 \wedge  \neg h3 \wedge  \neg h6 \wedge  \neg h9$ &
  $99.28$ &
  $h1 \vee h3 \vee h6 \vee h9$ &
  $99.28$ &
  $99.28$ \\ \hline
\end{tabular}%
}
\end{table}

% Please add the following required packages to your document preamble:
% \usepackage{multirow}
% \usepackage{graphicx}
\begin{table}[]
\centering
\caption{Cell differentiation explanations (* the explanation is too complex)}
\label{tab:exp_formula_celldiff}
\resizebox{\textwidth}{!}{%
\begin{tabular}{c|p{8cm}|l|p{8cm}|lll}
\hline
\multirow{2}{*}{\textbf{Method}} &
  \multicolumn{2}{c}{\textbf{Positive explanation}} &
  \multicolumn{2}{c}{\textbf{Negative explanation}} &
  \multicolumn{1}{c}{\multirow{2}{*}{\textbf{Model's accuracy (\%)}}} \\
 &
  \multicolumn{1}{c}{\textbf{Formula}} &
  \multicolumn{1}{c}{\textbf{Accuracy (\%)}} &
  \multicolumn{1}{c}{\textbf{Formula}} &
  \multicolumn{1}{c}{\textbf{Accuracy (\%)}} &
  \multicolumn{1}{c}{} \\ \hline
\multirow{10}{*}{\textbf{Pruning}} &
  $pcxa \wedge nr2c2 \wedge kat6b \wedge  \neg CD37 \wedge  \neg si:ch211-103n10.5 \wedge  \neg im:7151449 \wedge  \neg dnajc28 \wedge  \neg oraov1 \wedge  \neg igic1s1 \wedge  \neg clmn \wedge  \neg prune2$ &
  $90.91$ &
  $prune2 \wedge nr2c2 \wedge kat6b \wedge  \neg CD37 \wedge  \neg si:ch211-103n10.5 \wedge  \neg im:7151449 \wedge  \neg dnajc28 \wedge  \neg oraov1 \wedge  \neg igic1s1 \wedge  \neg pcxa \wedge  \neg clmn$ &
  $27.97$ &
  $93.71$ \\
 &
  $anxa3b \wedge dpysl5b \wedge pcxa \wedge nr2c2 \wedge kat6b \wedge  \neg Unnamed: 168 \wedge  \neg im:7151449 \wedge  \neg oraov1 \wedge  \neg eif4g2b \wedge  \neg clmn \wedge  \neg rgs11$ &
  $89.51$ &
  $nr2c2 \wedge  \neg pcxa \wedge  \neg clmn$ &
  $45.45$ &
  $94.41$ \\
 &
  $si:ch211-132g1.1 \wedge nr2c2 \wedge  \neg CD37 \wedge  \neg si:ch211-103n10.5 \wedge  \neg im:7151449 \wedge  \neg oraov1 \wedge  \neg Unnamed: 419 \wedge  \neg hif1al2 \wedge  \neg eif4g2b \wedge  \neg zdhhc5a \wedge  \neg clmn \wedge  \neg nanos1 \wedge  \neg adora2aa$ &
  $89.44$ &
  $eif4g2b \wedge  \neg si:ch211-132g1.1$ &
  $33.80$ &
  $92.96$ \\
 &
  $dpysl5b \wedge pcxa \wedge nr2c2 \wedge  \neg CD37 \wedge  \neg si:ch211-103n10.5 \wedge  \neg si:dkey-183p4.10 \wedge  \neg lect2l \wedge  \neg im:7151449 \wedge  \neg smim14 \wedge  \neg oraov1 \wedge  \neg igic1s1 \wedge  \neg otud4.4 \wedge  \neg eif2ak1 \wedge  \neg anxa11a \wedge  \neg TMC8 \wedge  \neg zgc:158427 \wedge  \neg HHEX \wedge  \neg clmn \wedge  \neg oxsr1a \wedge  \neg lpar1$ &
  $90.14$ &
  $smim14 \wedge otud4.4 \wedge  \neg TMC8 \wedge  \neg HHEX \wedge  \neg oxsr1a \wedge  \neg lpar1$ &
  $40.85$ &
  $95.07$ \\
 &
  $nr2c2 \wedge  \neg CD37 \wedge  \neg si:ch211-103n10.5 \wedge  \neg im:7151449 \wedge  \neg oraov1 \wedge  \neg igic1s1 \wedge  \neg eif4g2b \wedge  \neg zdhhc5a \wedge  \neg clmn$ &
  $75.35$ &
  $eif4g2b$ &
  $33.10$ &
  $91.55$ \\
 &
  $SLC16A3 \wedge pcxa \wedge nr2c2 \wedge kat6b \wedge  \neg CD37 \wedge  \neg Unnamed: 168 \wedge  \neg im:7151449 \wedge  \neg si:ch73-359m17.5 \wedge  \neg si:dkeyp-44a8.2 \wedge  \neg otud4.4 \wedge  \neg eif2ak1 \wedge  \neg anxa11a \wedge  \neg CABIN1 \wedge  \neg SBNO2 \wedge  \neg mgrn1b \wedge  \neg clmn$ &
  $85.21$ &
  $mgrn1b \wedge  \neg pcxa$ &
  $39.44$ &
  $90.14$ \\
 &
  $ap5z1 \wedge pcxa \wedge  \neg CD37 \wedge  \neg si:ch211-103n10.5 \wedge  \neg si:dkey-183p4.10 \wedge  \neg si:ch73-359m17.5 \wedge  \neg si:dkeyp-44a8.2 \wedge  \neg igic1s1 \wedge  \neg hinfp \wedge  \neg zgc:154055 \wedge  \neg tbc1d25 \wedge  \neg eif2ak1 \wedge  \neg anxa11a \wedge  \neg nemp2 \wedge  \neg atxn3 \wedge  \neg eif4g2b \wedge  \neg got2a \wedge  \neg si:dkey-9i23.5 \wedge  \neg zdhhc5a \wedge  \neg clmn \wedge  \neg nanos1$ &
  $85.92$ &
  $ \neg zgc:154055 \wedge  \neg pcxa$ &
  $47.18$ &
  $92.25$ \\
 &
  $ap5z1 \wedge pcxa \wedge  \neg eif4g2b \wedge  \neg mgrn1b \wedge  \neg oxsr1a \wedge  \neg kdelc2$ &
  $91.55$ &
  $kdelc2 \wedge  \neg pcxa \wedge  \neg clmn$ &
  $43.66$ &
  $95.07$ \\
 &
  $ \neg CD37 \wedge  \neg si:ch211-103n10.5 \wedge  \neg si:dkey-183p4.10 \wedge  \neg oraov1 \wedge  \neg Unnamed: 419 \wedge  \neg igic1s1 \wedge  \neg otud4.4 \wedge  \neg anxa11a \wedge  \neg eif4g2b \wedge  \neg asap2b \wedge  \neg timm17a \wedge  \neg clmn \wedge  \neg rgs11 \wedge  \neg ADM$ &
  $88.73$ &
  $otud4.4 \wedge eif4g2b \wedge  \neg CD37 \wedge  \neg si:ch211-103n10.5 \wedge  \neg si:dkey-183p4.10 \wedge  \neg oraov1 \wedge  \neg Unnamed: 419 \wedge  \neg igic1s1$ &
  $26.06$ &
  $92.96$ \\
 &
  $pcxa \wedge kat6b \wedge  \neg CD37 \wedge  \neg im:7151449 \wedge  \neg igic1s1 \wedge  \neg anxa11a \wedge  \neg eif4g2b \wedge  \neg clmn$ &
  $85.92$ &
  $ \neg CD37 \wedge  \neg im:7151449 \wedge  \neg igic1s1 \wedge  \neg pcxa \wedge  \neg clmn$ &
  $47.89$ &
  $90.85$ \\ \hline
\multirow{10}{*}{\textbf{$\psi$ net}} &
  $(False)$ &
  $0.00$ &
  $( \neg clmn \wedge (si:ch211-103n10.5 \vee oraov1))$ &
  $53.15$ &
  $83.92$ \\
 &
  $(im:7151449 \vee ( \neg si:ch211-103n10.5 \wedge  \neg anxa11a))$ &
  $32.17$ &
  $(si:ch211-103n10.5)$ &
  $30.07$ &
  $82.52$ \\
 &
  $(im:7151449 \wedge  \neg si:ch211-103n10.5)$ &
  $81.69$ &
  $(si:ch211-103n10.5 \vee  \neg im:7151449)$ &
  $81.69$ &
  $81.69$ \\
 &
  $(clmn)$ &
  $83.10$ &
  $(True)$ &
  $0.00$ &
  $83.10$ \\
 &
  $(im:7151449 \vee clmn \vee  \neg si:ch211-103n10.5)$ &
  $28.17$ &
  $(si:ch211-103n10.5)$ &
  $30.99$ &
  $83.10$ \\
 &
  $(False)$ &
  $0.00$ &
  $(si:ch211-103n10.5)$ &
  $29.58$ &
  $83.10$ \\
 &
  $(clmn \vee (im:7151449 \wedge  \neg si:ch211-103n10.5))$ &
  $84.51$ &
  $( \neg clmn)$ &
  $83.10$ &
  $81.69$ \\
 &
  $(clmn \vee (im:7151449 \wedge  \neg si:ch211-103n10.5))$ &
  $84.51$ &
  $(si:ch211-103n10.5)$ &
  $30.99$ &
  $84.51$ \\
 &
  $(pcxa \vee clmn)$ &
  $73.24$ &
  $( \neg clmn)$ &
  $83.80$ &
  $84.51$ \\
 &
  $(clmn)$ &
  $82.39$ &
  $( \neg clmn)$ &
  $82.39$ &
  $82.39$ \\ \hline
\multirow{10}{*}{\textbf{Decision tree}} &
  * &
  $88.81$ &
  * &
  $88.81$ &
  $88.81$ \\
 &
  * &
  $90.91$ &
  * &
  $90.91$ &
  $90.91$ \\
 &
  * &
  $91.55$ &
  * &
  $91.55$ &
  $91.55$ \\
 &
  * &
  $90.85$ &
  * &
  $90.85$ &
  $90.85$ \\
 &
  * &
  $94.37$ &
  * &
  $94.37$ &
  $94.37$ \\
 &
  * &
  $92.25$ &
  * &
  $92.25$ &
  $92.25$ \\
 &
  * &
  $94.37$ &
  * &
  $94.37$ &
  $94.37$ \\
 &
  * &
  $91.55$ &
  * &
  $91.55$ &
  $91.55$ \\
 &
  * &
  $91.55$ &
  * &
  $91.55$ &
  $91.55$ \\
 &
  * &
  $92.96$ &
  * &
  $92.96$ &
  $92.96$ \\ \hline
\multirow{10}{*}{\textbf{ReLU}} &
  $pcxa \wedge nr2c2 \wedge  \neg si:ch211-103n10.5 \wedge  \neg im:7151449 \wedge  \neg oraov1 \wedge  \neg clmn \wedge  \neg marcksl1b \wedge  \neg tm9sf3$ &
  $77.62$ &
  $otud4.4 \wedge  \neg pcxa \wedge  \neg clmn \wedge  \neg kdelc2$ &
  $25.17$ &
  $95.80$ \\
 &
  $pcxa \wedge  \neg si:ch211-103n10.5 \wedge  \neg kdelc2$ &
  $83.22$ &
  $pcxa \wedge  \neg si:ch211-103n10.5 \wedge  \neg kdelc2$ &
  $16.78$ &
  $94.41$ \\
 &
  $pcxa \wedge  \neg si:ch211-103n10.5 \wedge  \neg im:7151449 \wedge  \neg otud4.4 \wedge  \neg clmn$ &
  $82.39$ &
  $ \neg si:ch211-103n10.5 \wedge  \neg im:7151449 \wedge  \neg otud4.4 \wedge  \neg clmn$ &
  $54.23$ &
  $96.48$ \\
 &
  $si:ch211-132g1.1 \wedge pcxa \wedge  \neg CD37 \wedge  \neg si:ch211-103n10.5 \wedge  \neg otud4.4 \wedge  \neg eif2ak1 \wedge  \neg clmn \wedge  \neg marcksl1b \wedge  \neg kdelc2$ &
  $90.14$ &
  $eif2ak1 \wedge dpysl5b \wedge SLC16A3 \wedge asb12a \wedge kat6b \wedge kdelc2 \wedge  \neg CD37 \wedge  \neg si:ch211-103n10.5 \wedge  \neg anxa11a \wedge  \neg mgrn1b$ &
  $32.39$ &
  $97.18$ \\
 &
  $si:ch211-132g1.1 \wedge pcxa \wedge nr2c2 \wedge  \neg si:ch211-103n10.5 \wedge  \neg im:7151449 \wedge  \neg oraov1 \wedge  \neg otud4.4 \wedge  \neg anxa11a \wedge  \neg clmn \wedge  \neg marcksl1b \wedge  \neg kdelc2$ &
  $88.73$ &
  $otud4.4 \wedge  \neg si:ch211-103n10.5 \wedge  \neg im:7151449 \wedge  \neg oraov1 \wedge  \neg anxa11a \wedge  \neg clmn \wedge  \neg kdelc2$ &
  $40.14$ &
  $98.59$ \\
 &
  $si:ch211-132g1.1 \wedge pcxa \wedge nr2c2 \wedge  \neg si:ch211-137j23.8 \wedge  \neg CD37 \wedge  \neg si:ch211-103n10.5 \wedge  \neg im:7151449 \wedge  \neg oraov1 \wedge  \neg hinfp \wedge  \neg otud4.4 \wedge  \neg anxa11a \wedge  \neg atp2b4 \wedge  \neg clmn \wedge  \neg marcksl1b$ &
  $86.62$ &
  $oraov1 \wedge dpysl5b \wedge asb12a \wedge kat6b \wedge  \neg CD37 \wedge  \neg si:ch211-103n10.5 \wedge  \neg im:7151449 \wedge  \neg otud4.4 \wedge  \neg anxa11a \wedge  \neg clmn \wedge  \neg marcksl1b$ &
  $32.39$ &
  $93.66$ \\
 &
  $pcxa \wedge  \neg si:ch211-103n10.5 \wedge  \neg im:7151449 \wedge  \neg clmn \wedge  \neg kdelc2$ &
  $79.58$ &
  $ \neg si:ch211-103n10.5 \wedge  \neg im:7151449 \wedge  \neg clmn \wedge  \neg kdelc2$ &
  $38.73$ &
  $97.18$ \\
 &
  $si:ch211-132g1.1 \wedge pcxa \wedge nr2c2 \wedge kat6b \wedge  \neg si:ch211-103n10.5 \wedge  \neg im:7151449 \wedge  \neg zgc:113377 \wedge  \neg otud4.4 \wedge  \neg clmn \wedge  \neg marcksl1b \wedge  \neg oxsr1a \wedge  \neg kdelc2$ &
  $90.85$ &
  $dpysl5b \wedge SLC16A3 \wedge asb12a \wedge kat6b \wedge  \neg si:ch211-103n10.5$ &
  $65.49$ &
  $95.77$ \\
 &
  $si:ch211-132g1.1 \wedge pcxa \wedge nr2c2 \wedge  \neg si:ch211-103n10.5 \wedge  \neg znf1034 \wedge  \neg smim14 \wedge  \neg oraov1 \wedge  \neg Unnamed: 419 \wedge  \neg otud4.4 \wedge  \neg anxa11a \wedge  \neg clmn \wedge  \neg marcksl1b \wedge  \neg kdelc2$ &
  $88.73$ &
  $smim14 \wedge otud4.4 \wedge pcxa \wedge nr2c2 \wedge  \neg si:ch211-137j23.8 \wedge  \neg si:ch211-103n10.5 \wedge  \neg znf1034 \wedge  \neg oraov1 \wedge  \neg Unnamed: 419 \wedge  \neg anxa11a \wedge  \neg clmn \wedge  \neg marcksl1b \wedge  \neg kdelc2$ &
  $17.61$ &
  $94.37$ \\
 &
  $pcxa \wedge  \neg si:ch211-103n10.5 \wedge  \neg im:7151449 \wedge  \neg otud4.4 \wedge  \neg CABIN1 \wedge  \neg clmn \wedge  \neg kdelc2$ &
  $83.10$ &
  $asb12a \wedge kat6b \wedge kdelc2 \wedge  \neg CD37 \wedge  \neg si:ch211-103n10.5 \wedge  \neg otud4.4 \wedge  \neg anxa11a \wedge  \neg CABIN1 \wedge  \neg pcxa \wedge  \neg clmn$ &
  $32.39$ &
  $96.48$ \\ \hline
\end{tabular}%
}
\end{table}
