# Supplementary material for: Logic Explained Networks
Source: arXiv:2108.05149 source file (2021-08-11)
Supplement: Supplementary file 2 [file main_sm.tex]

% \usepackage{icml2021}

\usepackage[utf8]{inputenc} % allow utf-8 input
\usepackage[T1]{fontenc}    % use 8-bit T1 fonts
\usepackage[pagebackref=true,
    breaklinks=true,
    colorlinks,
    linkcolor=blue,
    citecolor=blue,
    filecolor=black,
    urlcolor=blue,
    bookmarks=false]{hyperref}
\usepackage{url}            % simple URL typesetting
\usepackage{booktabs}       % professional-quality tables
\usepackage{amsfonts}       % blackboard math symbols
\usepackage{nicefrac}       % compact symbols for 1/2, etc.
\usepackage{microtype}      % microtypography
\usepackage{lipsum}
\usepackage{graphicx}
\usepackage{amssymb}
\usepackage{multirow}
\usepackage{caption}
\usepackage{subcaption}

\setcounter{secnumdepth}{6}


\usepackage{tikz}
% \usetikzlibrary{decorations}
\usetikzlibrary{decorations.text}
\usetikzlibrary{arrows.meta,bending,decorations.markings}


\usepackage{listings}
\usepackage{xcolor}

\definecolor{codegreen}{rgb}{0,0.6,0}
\definecolor{codegray}{rgb}{0.5,0.5,0.5}
\definecolor{codepurple}{rgb}{0.58,0,0.82}
\definecolor{backcolour}{rgb}{0.95,0.95,0.92}

\lstdefinestyle{mystyle}{
    backgroundcolor=\color{backcolour},   
    commentstyle=\color{codegreen},
    keywordstyle=\color{magenta},
    numberstyle=\tiny\color{codegray},
    stringstyle=\color{codepurple},
    basicstyle=\ttfamily\footnotesize,
    breakatwhitespace=false,         
    breaklines=true,                 
    captionpos=b,                    
    keepspaces=true,                 
    numbers=left,                    
    numbersep=5pt,                  
    showspaces=false,                
    showstringspaces=false,
    showtabs=false,                  
    tabsize=2
}

\lstset{style=mystyle}

\usepackage{pifont}
\usepackage{amsmath}
\usepackage{amsthm}
\usepackage{mathtools}
\usepackage{float}
\usepackage{fontawesome}
\usepackage{makecell}

\def\UrlFont{\rmfamily}
\usepackage{fancyhdr}
\usepackage{mathrsfs} 
\usepackage{color}
\usepackage{hyperref}
\usepackage{longtable}
\hypersetup{colorlinks=true}
% \usepackage[linesnumbered, ruled]{algorithm2e}


\newtheorem{definition}{Definition}[]
\newtheorem{theorem}{Theorem}[section]
\newtheorem{corollary}{Corollary}[theorem]
\newtheorem{lemma}[theorem]{Lemma}
\newtheorem{example}{Example}


\newcommand{\cmark}{\ding{51}}%
\newcommand{\xmark}{\ding{55}}%

\graphicspath{ {./images/} }


\def\[#1\]{$$#1$$}

\def\frac#1#2{{#1\over#2}}
\def\eps{\varepsilon}

\def\bbR{{\bf R}}
\def\X{{\bf X}}
\def\meno{\medskip\noindent}

\newcommand{\fg}[1]{\textcolor{red}{F: #1}}
\newcommand{\gc}[1]{\textcolor{red}{G: #1}}
\newcommand{\sm}[1]{\textcolor{blue}{#1}}


% Please add the following required packages to your document preamble:
% \usepackage{graphicx}
\setlength{\tabcolsep}{10pt}
\renewcommand{\arraystretch}{1.5}


\title{\sm{Logic} Explained Networks}

\author{Gabriele Ciravegna\thanks{Equal contribution}\hspace{1.2mm}$^{1,2}$\hspace{1.2mm}\href{https://orcid.org/0000-0002-6799-1043}{\includegraphics[scale=0.06]{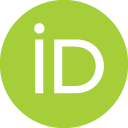}}, 
Pietro Barbiero$^{*3}$\hspace{1mm}\href{https://orcid.org/0000-0003-3155-2564}{\includegraphics[scale=0.06]{orcid.png}}, 
Francesco Giannini$^{*2}$, \\
\textbf{
Marco Gori$^{2,4}$\hspace{1mm}\href{https://orcid.org/0000-0001-6337-5430}{\includegraphics[scale=0.06]{orcid.png}}, 
Pietro Li\'o$^{3}$, 
Marco Maggini$^{2}$, 
Stefano Melacci$^{2}$\hspace{1mm}\href{https://orcid.org/0000-0002-0415-0888}{\includegraphics[scale=0.06]{orcid.png}}
}\\
$^{1}$Universita' di Firenze (Italy), $^{2}$Universita' di Siena (Italy), \\ $^{3}$University of Cambridge (UK), \sm{$^{4}$Universitè Côte d’Azur (France)}\\
\texttt{gabriele.ciravegna@unifi.it, pb737@cam.ac.uk, fgiannini@diism.unisi.it}\\
\texttt{\sm{marco.gori@unisi.it, pl219@cam.ac.uk, marco.maggini@unisi.it, mela@diism.unisi.it}}
}

\begin{document}
\maketitle
\begin{abstract}
\sm{The large and still increasing popularity of deep learning clashes with a major limit of neural network architectures, that consists in their lack of capability in providing human-understandable motivations of their decisions.}
%Despite the increasing popularity of deep \sm{networks in real-world application}, in real wold domains the employment of deep neural networks is still limited and strongly criticized due to their lack of interpretability. 
\sm{In situations in which the machine is expected to support the decision of human experts, providing a comprehensible explanation is feature of crucial importance.}
%providing a comprehensible explanation for a certain classification task can be crucial in decision support contexts. 
\sm{The language used to communicate the explanations must be formal enough to be implementable in a machine and friendly enough to be understandable by a wide audience.}
%To this aim, rule-based explanations expressed in a high-level language are particularly relevant. 
In this paper, we \sm{propose} a general approach to Explainable Artificial Intelligence \sm{in the case of neural architectures}, showing how a mindful design of the networks leads to interpretable deep learning models called \sm{Logic} Explained Networks (LENs). 
\sm{LENs} only require \sm{their inputs} to be semantically meaningful and human understandable predicates, \sm{and they provide explanations in terms of simple First-Order Logic formulas involving such predicates.} LENs are general enough to cover a large number of scenarios. Amongst them, we consider the case in which \sm{LENs are directly used as special classifiers} with the capability of being explainable, or when they act as additional networks with the role of creating the conditions for \sm{making a black-box classifier explainable by FOL.} 
Explanations can be either \sm{local (single-example level) or global (problem level)}, and,
despite supervised learning problems are mostly emphasized, 
%and are given as first-order logic formulas expressed in terms of input concepts. 
we also show that LENs can learn to provide explanations in unsupervised learning settings.
%to provide explanations of the predictions made either by a black-box model or by the LEN itself. 
We describe and \sm{evaluate three different use-cases of the LEN framework}, based on multiple out-of-the-box LEN models. Experimental results on several datasets and tasks \sm{show} that LENs not only \sm{yield better classifications than established white-box models}, such as decision trees and Bayesian rule lists, but \sm{they} also provide \sm{more compact} and meaningful explanations.
\end{abstract}


\begin{figure}[h]
    \centering
    \includegraphics[width=1\textwidth]{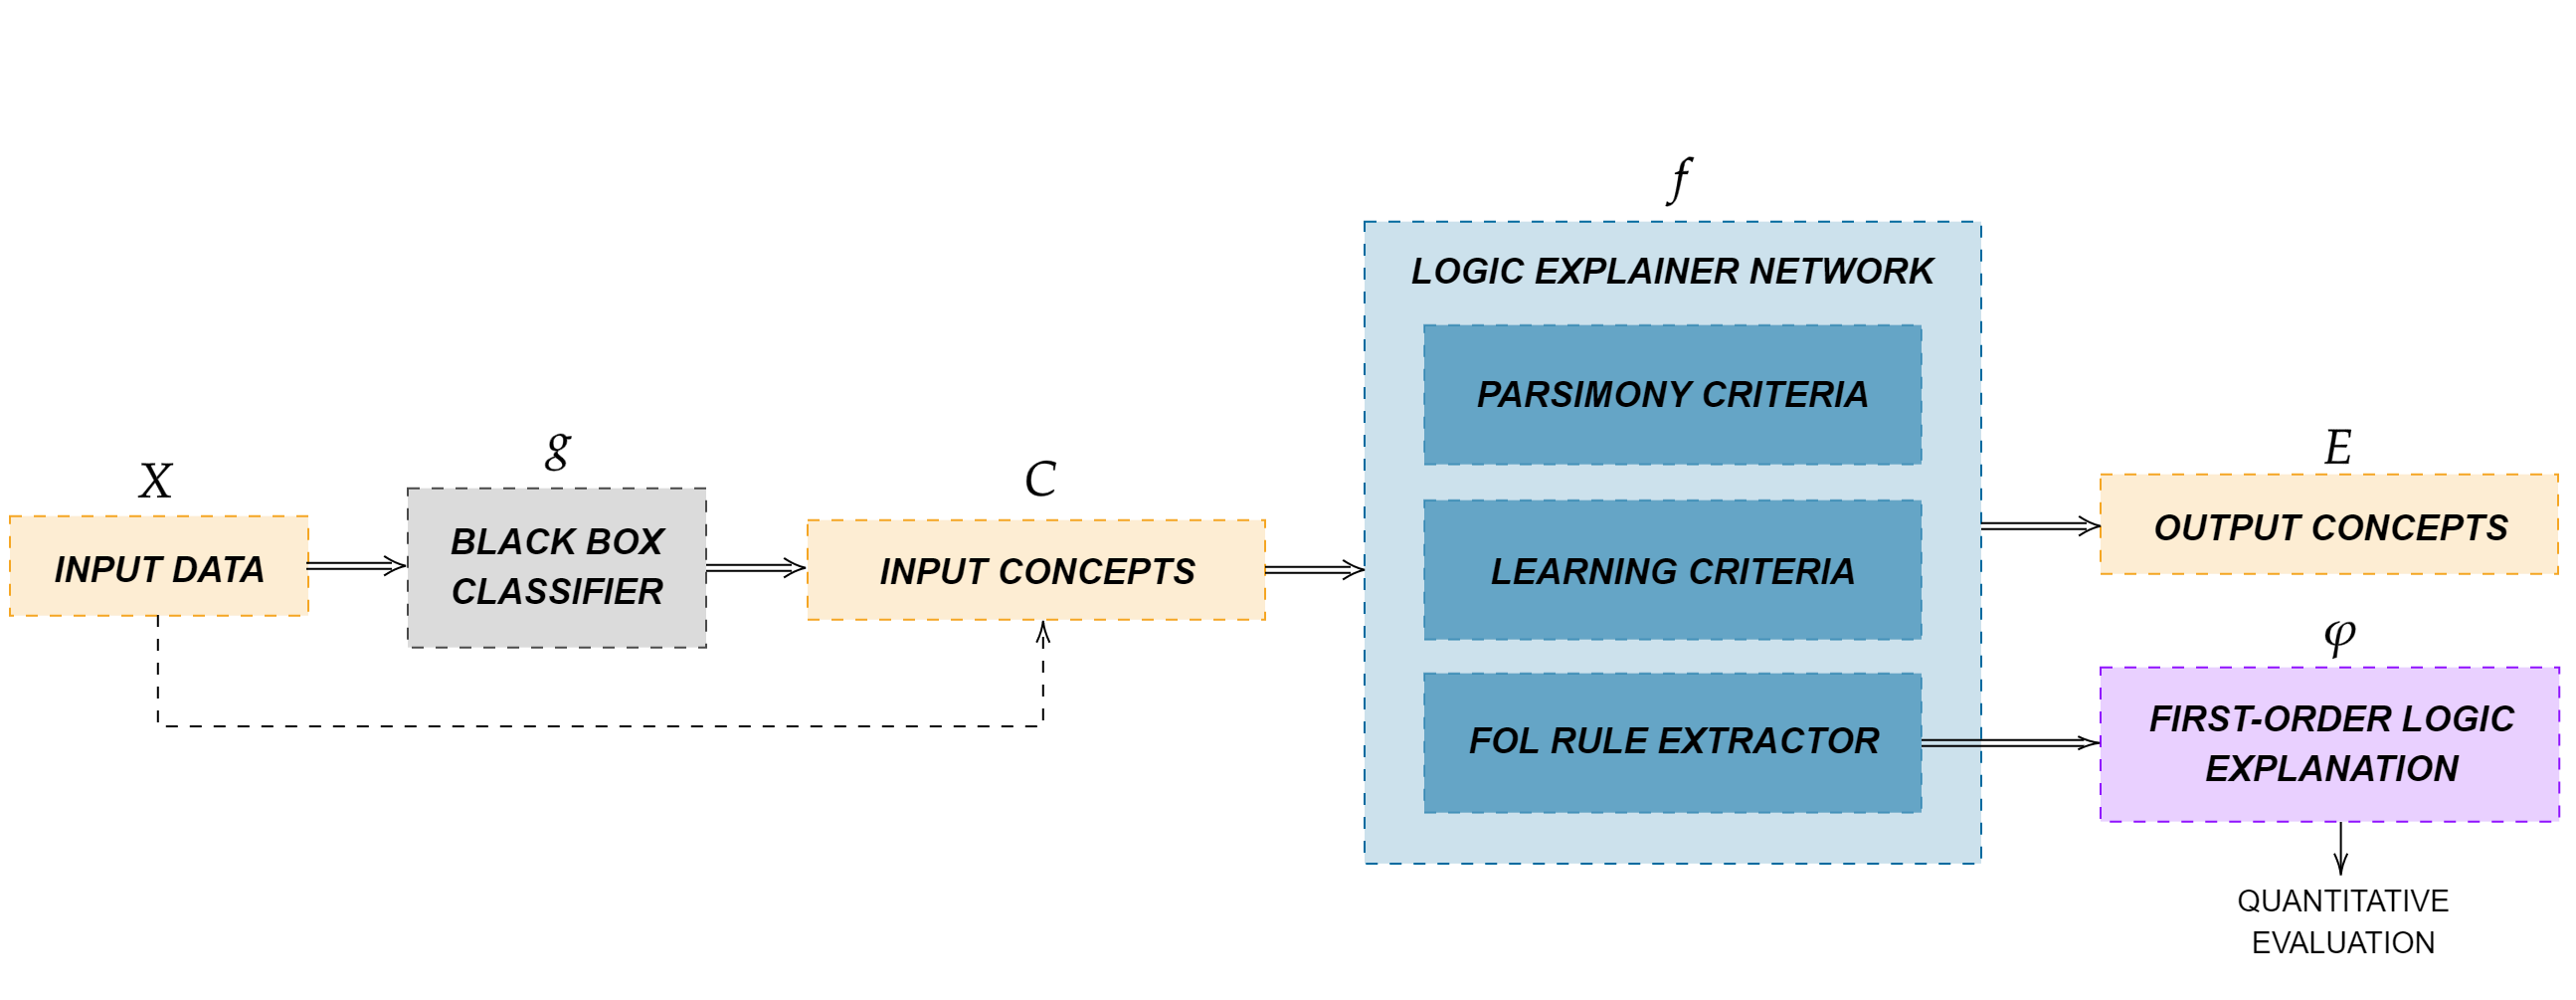}
\caption{\sm{Logic Explained Networks (LENs) are neural networks capable of making predictions and providing First-Order Logic explanations. In detail, A LEN (blue box -- function $f$) provides FOL explanations (purple box -- function $\varphi$) of a set of output concepts (rightmost yellow-box -- output concepts belong to set $E$) in function of the LEN inputs, that might be other concepts (mid yellow box -- input concepts belong to $C$) computed by a neural network (gray box -- function $g$) and/or concepts provided within the available data (leftmost yellow box -- data belong to $X$), following the dotted connection). } %Colors are used in all figures to identify different parts of the framework: yellow boxes contain input data and concepts, output predictions and labels; grey boxes represent the black box classifier $g$ that can either provide final classification or extract low-level concepts; the blue box represents the LEN $f$; t
\sm{There are several different ways of instantiating this generic model into real-world problems, that are described in Section~\ref{sec:basics}. 
Within the blue box, the key components of LENs are listed, that are the main subject of Section~\ref{sec:methods}: } Learning Criteria (Section~\ref{sec:learncrit}), FOL Rule Extractor (Section~\ref{sec:logic_rule_extr}), and the Parsimony Criteria (Section~\ref{sec:parsimony}).
}
    \label{fig:framework}
\end{figure}

\begin{figure}[h]
    \centering

     \includegraphics[width=0.9\textwidth]{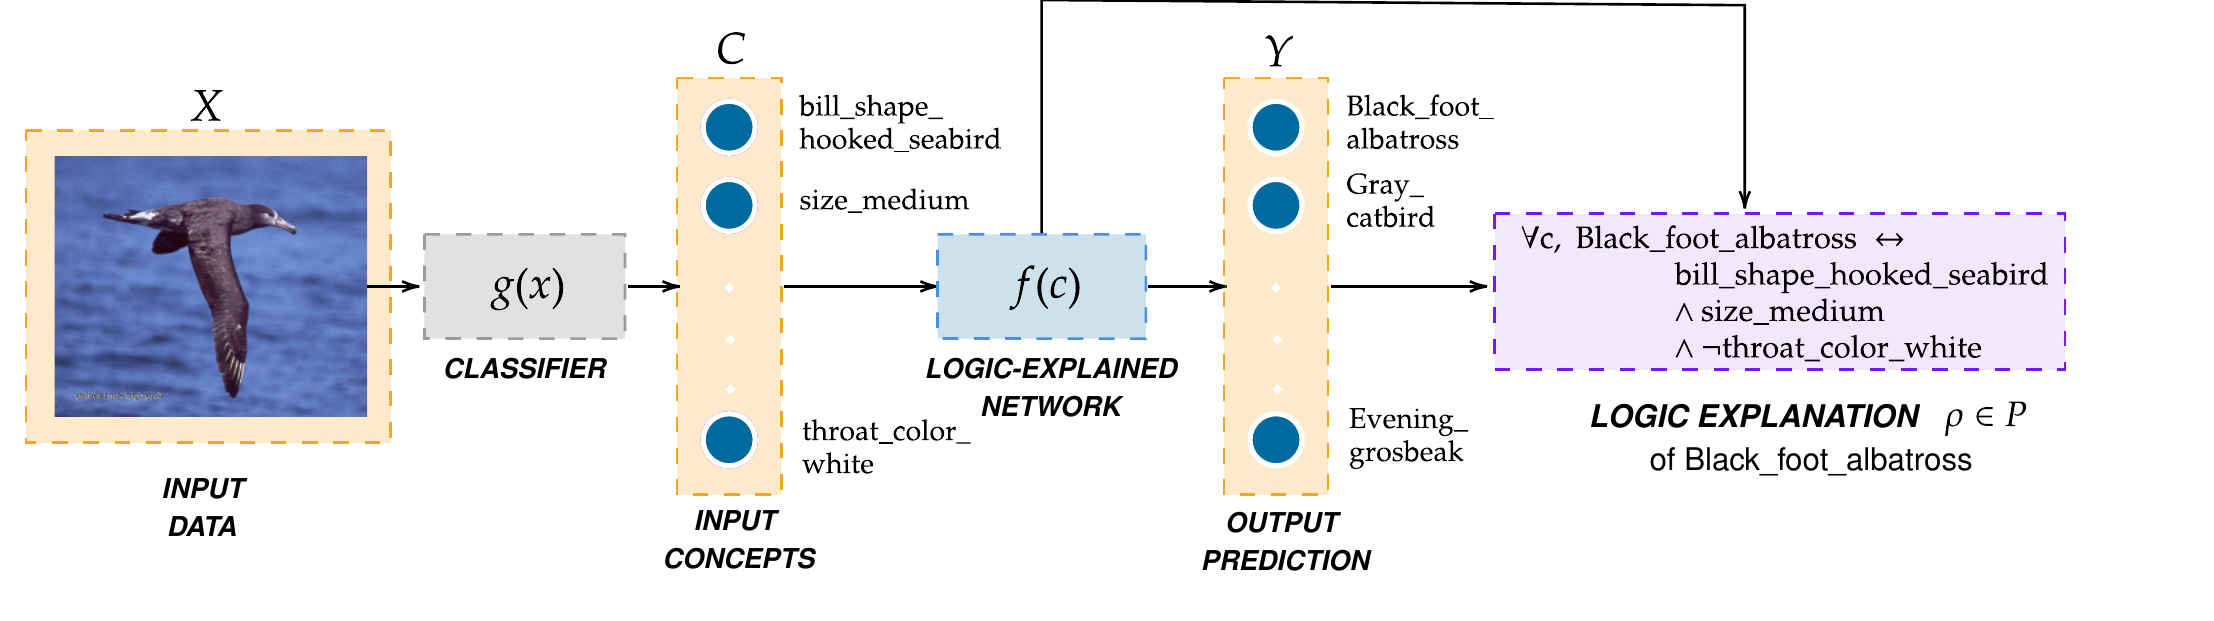}
         \caption{\sm{An example of a possible instance of the generic model of Fig.~\ref{fig:framework}, inspired by the CUB 200-2011 fine-grained classification dataset. Classes are divided into a two-level hierarchy.} {\color{red}[Add a citation to the dataset.]} A LEN is placed on top of a convolutional neural network $g(\cdot)$ in order to \textit{(i)} classify the species of the bird in input and \textit{(ii)} provide an explanation on why it belongs to this class. {\color{red}[Add at least another output concept (no need to show its explanation). Avoid being to strictly close to the CUB dataset, otherwise the example is not clear. In other words, make black-footed-albatross the name of the output concept (instead of 'bird') and also add another one. Rename the input concepts with the names that are in the purple box. If they are too long, you can shorten them by renaming them in a more simple manner (hooked-bill, solid-wing, medium-size, white-throat, black-bill). Moreover, user the lower-case $x$ instead of $X$.]}}
         \label{fig:len}

\end{figure}


\section{Introduction}
The lack of transparency in the decision process of some machine learning models, such as neural networks, \sm{limits} their application in many safety-critical domains \cite{chander2018working}. Employing black-box\footnote{\sm{In the context of this paper, a black-box classifier is any classifier that cannot provide human understandable explanations about its decisions}} models may be unacceptable in contexts such as industry, medicine or courts, where the potential economical or ethical repercussions are calling for lawmakers to discourage from a reckless application of non-interpretable models \cite{gdpr2017,law10code,goddard2017eu,gunning2017explainable}. As a consequence, research in Explainable Artificial Intelligence (XAI) has become strategic and has been massively encouraged, leading to the development of a variety of techniques that aim at explaining black-box models \cite{das2020opportunities,brundage2020toward} or at developing effective interpretable models \cite{carvalho2019machine,rudin2019stop}. 
% Some of the latter case, like decision rules, provide one of the best forms of explanations as they were originally developed for decision support systems \cite{sprague1980framework}.

The notions of \emph{interpretability} and \emph{explainability} were historically used as synonyms, however nowadays the distinction between interpretable models and models providing explanations has become more \sm{evident}, as recently discussed by different authors \cite{gilpin2018explaining,lipton2018mythos,marcinkevivcs2020interpretability}. 
{\color{red}[Say something on the definitions of interpretability and explainability, connected to what follows (we need to define what we mean with these terms).]}
In some contexts, the use of a black-box model may be unnecessary or even not preferable \cite{rudin2019stop}. For instance, a proof of concept, a prototype, or the solution to a simple classification problem can be easily based on standard out-of-the-box AI solutions which are interpretable by design.
However, interpretable models may generally miss to capture complex relationships among data. Hence, in order to achieve state-of-the-art performance in more challenging problems, it may be necessary to exploit black-box models that, in turn, may require an additional explanatory model to gain the trust of the user. 

In the literature, there is a wide consensus on the necessity of having an explanation for machine learning models that are employed in safety-critical domains, while there is not even agreement on what an \emph{explanation} actually is, nor if it could be formally defined \cite{doshi2017towards,lipton2018mythos}.
An explanation should serve cognitive-behavioral purposes such as engendering trust, aiding bias identification, or taking actions/decisions \cite{srinivasanexplanation}. An explanation may help humans \sm{understand} the black box, may allow for a deeper human-machine interaction \cite{koh2020concept}, and may engender trust on fully automated tasks. All of this is possible as long as the explanations are useful from a human perspective.
% and take into account how humans think and make decisions
In a nutshell, an explanation is an answer to a ``why'' question %\cite{miller2019explanation}. 
%But what is that characterize a good explanation? 
and what makes an explanation good or bad depends on ``the degree to which a human can understand the cause of a decision'' \cite{miller2019explanation}. The goodness of an explanation is intimately connected to how humans collect evidences and eventually make decisions. 
In Herbert Simon's words we may say that a good explanation is \textit{satisficing} \cite{simon1956rational}, i.e. \textit{it either gives an optimal description of a simplified version of the black box (e.g. a surrogate model) or a satisfactory description for the black box itself}
% \footnote{"Decision makers can satisfice either by finding optimum solutions for a simplified world, or by finding satisfactory solutions for a more realistic world".}
\cite{simon1979rational}. However, the notion itself of explanation generally depends on both the domain of the application and who it is aimed at \cite{carvalho2019machine}.
% This is the reason why, different criteria and taxonomies 
% such as the \textit{scope}, the \textit{usage} and the \textit{methodology} have been identified as key-properties to define a XAI technique \cite{das2020opportunities}. 


The need for high-quality evidences is one of the main reasons why concept-based explanations are receiving ever-growing consideration. \sm{Explanations are} given in terms of human-understandable symbols (the \textit{concepts}) rather than raw features such as pixels or characters \cite{kim2018tcav,ghorbani2019towards,koh2020concept}. As a consequence, they seem more suitable to serve many strategic human purposes such as decision making tasks. For instance, a concept-based explanation may describe a high-level category through its attributes as in ``a \textit{human} has \textit{hands} and a \textit{head}''.
% However, many concept-based explanations still look ambiguous, it is not obvious how to \textit{quantitatively} assess their generality, and may not be suitable for effective decision making at all.
% How much effort requires analyzing a pairwise dependence plot \cite{friedman2008predictive} or a ranking of SHAP values \cite{NIPS2017_7062} or a decision tree with depth 10 \cite{breiman1984classification} for domain experts? How much for laypeople?
% If you are looking for a quick and comprehensible answer these methodologies will not suit your needs.
While collecting high-quality evidences for an explanation is a common feature of concept-based techniques, there are very few approaches formulating hypothesis and even less providing synthetic descriptions whose validity can be quantitatively assessed \cite{das2020opportunities}.
A possible solution is to rely on a formal language that is
% synthetic but also 
very expressive and closely related to natural language and reasoning, such as First-Order Logic (FOL). A FOL explanation can be considered a special kind of \sm{a} concept-based explanation, where the description is given in terms of logical predicates, connectives and quantifiers, such as ``$\forall x:\ \textit{is\_human}(x) \rightarrow \textit{has\_hands}(x) \wedge \textit{has\_head}(x)$''. However, FOL formulas generally express much more complex relationships among the concepts %that are 
involved in a certain explanation. Compared to other concept-based techniques, logic-based explanations provide many key advantages, \sm{that we briefly described in what follows}.
% \begin{itemize}
% CLARITY
An explanation reported in FOL is a rigorous and unambiguous statement (\textsc{clarity}). This formal clarity may serve cognitive-behavioral purposes such as engendering trust, aiding bias identification, or taking actions/decisions. For instance, \sm{dropping quantifiers and variables for simplicity}, the formula ``\textit{snow} $\wedge$ \textit{tree} $\leftrightarrow$ \textit{wolf}'' may easily outline the presence of a bias in the collection of training data.
% MODULARITY
Different logic-based explanations can be combined to describe groups of observations or global phenomena (\textsc{modularity}). %Different observations of the same phenomenon may have completely different %logic-based 
%explanations according to their characteristics. 
For instance, for an image showing only the face of a person, \sm{an} explanation could be ``(\textit{nose} $\wedge$ \textit{lips}) $\rightarrow$ \textit{human}'', while for another image showing a person from behind a valid explanation could be ``(\textit{feet} $\wedge$ \textit{hair} $\wedge$ \textit{ears})  $\rightarrow$ \textit{human}''. The two local explanations can be combined \sm{into} ``(\textit{nose} $\wedge$ \textit{lips}) $\vee$ (\textit{feet} $\wedge$ \textit{hair} $\wedge$ \textit{ears}) $\rightarrow$ \textit{human}''.
% MEASURABILITY
The quality of logic-based explanations can be quantitatively measured
    % on independent data sets 
to check their correctness and completeness (\textsc{measurability}). For instance, once the explanation ``(\textit{nose} $\wedge$ \textit{lips}) $\vee$ (\textit{feet} $\wedge$ \textit{hair} $\wedge$ \textit{ears})'' is extracted for the class \textit{human}, this logic formula can be applied on a test set to check its generality in terms of quantitative metrics like accuracy, fidelity and consistency.
% SIMPLIFIABILITY
\sm{Finally,} FOL-based explanations can be rewritten in 
    different equivalent forms such as in \emph{Disjunctive Normal Form} (DNF) and \emph{Conjunctive Normal Form} (CNF)  (\textsc{simplifiability}). Further, techniques such as the Quine–McCluskey algorithm can be used to compact and simplify logic explanations \cite{mccoll1878calculus,quine1952problem,mccluskey1956minimization}. For instance, the explanation ``(\textit{person} $\wedge$ \textit{nose}) $\vee$ ($\neg$\textit{person} $\wedge$ \textit{nose})'' can be easily simplified in ``\textit{nose}''.
% \end{itemize}


This paper presents a unified framework for XAI where a neural network, the \emph{\sm{Logic} Explained Network} (LEN), is trained to \textit{solve-and-explain} a categorical learning problem \sm{integrating elements from deep learning and logic}. 
\sm{Differently from vanilla neural architectures}, LENs can be \sm{directly} interpreted \sm{by means of} a set of \sm{FOL} formulas. \sm{In order to implement such property, LENs require their inputs to represent the activation scores of human-understandable concepts. Then, specifically designed learning objectives allow LENs to make predictions in a way that is well suited for providing FOL-based explanations that involve the input concepts. In order to reach this goal, LENs exploit parsimony criteria aimed at keeping their structure simple.}
% learn a set of explanations of its classification results, or for the class-assignments of another classifier. 
%(eventually another neural network). 
\sm{There are several different computational pipelines in which a LEN can be configured, depending on the properties  of the considered problem and on other potential experimental constraints. For example, LENs can be used to directly classify data in an explainable manner, or to explain another black-box neural classifier. Moreover, according to the user expectations}, different kinds of logic rules may be provided. 
\sm{Due to this intrinsic versatility of LENs, what we propose can also be taught as a generic framework that encompasses a large variety of use cases.}

%This versatility makes the proposed framework 
%and in particular LENs 
%applicable to a wide range of learning tasks \sm{and in different use cases.} % by providing logic-based explanations in different use cases. % and according to different user preferences. 
\sm{Fig.~\ref{fig:framework} depicts a generic view on LENs, in which the main components are reported. A LEN (blue box -- function $f$) provides FOL explanations (purple box) of a set of output concepts (rightmost yellow-box) in function of the LEN inputs. Inputs might be other concepts (mid yellow box) computed by a neural network classifier (gray box -- function $g$) and/or concepts provided within the available data (leftmost yellow box). %The output concepts are the ones that are the main subject of the explanations (e.g., they could be the classes of a classification problem). Explanations involve the inputs of the LEN. 
This generic structure can be instantiated in multiple ways, depending on the final goal of the user and on the properties of the considered problem. In order to provide the reader with an initial example/use-case (different configurations are explored in the paper), we consider an image classification problem with concepts organized into a two level hierarchy. In Fig.~\ref{fig:len} we report an instance of Fig.~\ref{fig:framework} in which a CNN-based neural classifier gets an input image $X$, predicting the activations of a number of low-level concepts (organized in a vertical manner). The LEN $f$ processes such concepts, and it predicts the activation of higher-level output concepts. The LEN can provide a FOL description of each (high-level) output concept with respect to the (low-level) input ones. Another possible instance of the proposed framework consists in using the LEN to directly classify and explain some input data (that is basically the case in which the input concepts are immediately available in the data themselves, and not the output of another neural model), thus the LEN itself becomes an explainable machine. Moreover, LENs can be paired with a black-box classifier operating on the same input data, and forced to mimic as much as possible the behaviour of the black-box, basically implementing an additional  explanation-oriented module. At a first glance, since the internal structure of LENs is subject to a number of constraints, LENs might not be as powerful as a black-box classifier. However, the versatility of LENs allows the user to customize his approach to the considered classification problem in order to find a satisfactory compromise between interpretability and accuracy.}

\sm{We investigate three different use-cases that are inspired by the aforementioned instances, comparing different ways of implementing the LEN models. While most of the emphasis of this paper is on supervised classification, we also show how LEN can be exploited in fully unsupervised settings.}
Additional human priors could be eventually incorporated into the learning process \cite{ciravegna2020constraint}, in the architecture \cite{koh2020concept}, \sm{and, following \cite{ciravegna2020constraint,ciravegna2020human}, what we propose can be trivially extended to semi-supervised learning (out of the scope of this paper).}


%Furthermore, LENs can also be integrated with existing black-box classifiers to extract low-level concepts or to explain their classification results.




%The overall problem configuration of how a Logically Explained Network can be integrated with an existing classifier is shown in Fig. \ref{fig:framework} and further described in Sec. \ref{sec:use_cases}. A configuration example is reported in Fig. \ref{fig:len}.




%Out-of-the-box neural networks based on this framework span a wide range of flavors, from fully interpretable models to black-boxes providing different interpretability-VS-accuracy trade-off.  
%high-quality explanations and state-of-the-art classification performance.

%Further, human priors expressed by FOL formulas can be naturally incorporated with LENs both in the learning process \cite{ciravegna2020constraint} and in the architecture \cite{koh2020concept}. 

Our work contributes to the XAI research field in the following ways.
\begin{itemize}
    \item \sm{It provides} a unifying framework for solving and explaining categorical learning problems with neural networks. We designed the LEN framework inspired by our previous experiences \cite{ciravegna2020human,ciravegna2020constraint}.
    \item \sm{It allows users to decide how to interconnect LENs in the classification task under investigation,} and to express a set of preferences to get one or more customized explanations. We provide and experimentally evaluate three out-of-the-box preset models.
    % \item Supporting a wide range of logic-based explanations from \textit{local explanations} and \textit{node-level explanations}, explaining the prediction for an individual sample or a hidden neuron, to \textit{cluster explanations} up to \textit{class-level explanations} and \textit{global explanations}.
    \item \sm{It offers} a wide range of logic-based explanations at different level of granularity, such as \textit{example}, \textit{local} and \textit{global} explanations, aiming at explaining a single sample, a subset of the available data or the whole dataset, respectively.
    \item \sm{It reports} experimental results confirming how LENs generalize better in terms of model accuracy than established white-box models such as decision trees on complex Boolean tasks (as observed in \cite{tavares2020understanding}).    
    \item \sm{It advertises our public} implementation of LENs through a Python package\footnote{\url{https://pypi.org/project/deep-logic/}} with an extensive documentation on out-of-the-box LENs, implementing different trade-offs between intepretability, explainability and accuracy. {\color{red}[This goes back to my previous comment on better defining these terms.]}
\end{itemize}

% \paragraph{Reading path} 
The paper is organized as follows. Related works are described in Section \ref{sec:related}. Section \ref{sec:basics} gives a formal definition of a LEN and it describes its underlying assumptions, key paradigms and design principles. The methods used to extract logic formulas and to effectively train LENs are described in Section \ref{sec:methods}. Three out-of-the-box LENs, presented in Section \ref{sec:outofthebox}, are compared on a wide range of benchmarks in terms of classification performance and quality of the explanations, in Section \ref{sec:experiments}. 
% A coding example showing how to use LENs with the associated python library is shown in Section \ref{sec:tool}. 
Finally, Section \ref{sec:conclusion} outlines the social and economical impact of this work as well as future research directions.


\section{Related work}
\label{sec:related}


In the last few years, the demand for human-comprehensible models has significantly increased in safety-critical and data-sensible contexts. This popularity is justified by the emerging need for unveiling the decision process of pitch-black models like deep neural networks. To this aim, the scientific community has developed an important variety of XAI techniques, with different properties and goals. Several taxonomies have been proposed to categorize the XAI models, with partial overlapping and some ambiguities on the referred terminology. Without pretending to be exhaustive, in the following we only focus on some key-properties that are relevant to compare LENs with other existing approaches. In particular, we will \sm{describe} related works \sm{considering the type of} \textsc{result} \sm{they provide} (feature-scoring vs. rule-based), 
\sm{their specific} \sm{\textsc{role}} (interpretable models vs. explanation methods), 
and the \textsc{scope} of the provided explanations (local vs. global). A brief summary of a few XAI works in terms of these features is reported in Tab.~\ref{tab:related_work} -- for more details on existing taxonomies we refer, e.g., to the following surveys \cite{adadi2018peeking,carvalho2019machine,marcinkevivcs2020interpretability,molnar2020interpretable}.

%\textsc{Results of Explanation Methods. }
XAI models can be differentiated according to the \textsc{result} of the produced explanation. 
Most of the methods in literature usually focus on scoring or providing summary statistics of features. However, \textit{feature-scoring} methods
%
can be of scarce utility in decision support cases, whereas a comprehensible language may bring light on the black-box behaviour by identifying concept-based correlations.
% do not consider how concepts are interconnected, therefore, these explanations may not live up to the expectations. 
On the other hand, \emph{rule-based} explanations are generally more comprehensible, since they usually rely on a formal language, such as \sm{FOL}. Further, the learned rules can be directly applied to perform the learning task in place of the explained model.
%\textsc{Explanation Usage. }
\sm{Existing approaches has different \textsc{roles} in the XAI landscape, acting as intrinsically \emph{interpretable models} or as \emph{explanation methods}. }
\sm{As a matter of fact,} the interpretability of a model can be achieved either by constraining the model to be interpretable per se (\emph{interpretable models}) or by applying some methods to get an explanation of an existing model (\emph{explanation methods}). Interpretable models are by definition {model specific}, while explanation methods can rely on a single model or be, as more commonly happens, {model agnostic}. In principle, interpretable models are the best suited to be employed as decision support systems. However, their decision function often is not smooth which makes them quite sensible to data distribution shifts and impairs their generalization ability on unseen observations \cite{tavares2020understanding,molnar2020interpretable}. 
On the other hand, explanation methods can be applied to get approximated interpretation of state-of-the-art models. These methods are generally {``post hoc''}, since the explanations are produced when the training procedure is concluded. 
%\textsc{Scope of Interpretability. }
A fundamental feature to distinguish among explainable methods \sm{is the \textsc{scope} of the provided explanations. \textit{Local} explanations are valid for a single given sample, while \textit{global} explanations {hold} on the whole input space}. However, several models consider local explanations together with aggregating heuristics to get a global explanation.

% {\bf Methodology. }
% The algorithms employed by most XAI models can be roughly categorized into two main categories. \textit{Backpropagation}-based techniques analyze the gradients of the activation up to the input features, in order to identify the most relevant ones for the classification task. \textit{Perturbation}-based techniques, instead, observe how the machine output changes when altering a given input data. The aim of these methods is to understand which %are the most discriminative 
% features (when altered) may drive the model to take different decisions. 
% Nonetheless, not all algorithms belong to these two categories. In particular, \textit{Model-intrinsic} explanation methods significantly differ according to the training algorithms.

\begin{table}[t]
\centering
\setlength{\tabcolsep}{8pt} % Default value: 6pt
\renewcommand{\arraystretch}{1.3} % Default value: 1
\resizebox{\textwidth}{!}{
\begin{tabular}{l|cc|cc|cc}
                                    & \multicolumn{2}{c|}{\sm{\textbf{Result Type}}} & \multicolumn{2}{c|}{\textbf{Scope}} & \multicolumn{2}{c}{\sm{\textbf{Role}}} \\
                        & feature-scoring & rule-based & local & global & interpretable model & explanation method \\ 
\hline
LIME &\faCheckCircle & & \faCheckCircle            & & & \faCheckCircle  \\
SHAP &\faCheckCircle & & \faCheckCircle & & & \faCheckCircle  \\
% DeConv \cite{zeiler2014visualizing}                     &\faCheckCircle&& \faCheckCircle            &            &              & \faCheckCircle           & \faCheckCircle         &               &                  \\
Activation Maximization & \faCheckCircle & & \faCheckCircle  &  &  & \faCheckCircle  \\
Saliency Maps &\faCheckCircle&& \faCheckCircle &      &              & \faCheckCircle \\
% Grad-CAM \cite{selvaraju2017grad}                       &\faCheckCircle&& \faCheckCircle            &            &              & \faCheckCircle           &              & \faCheckCircle          &                  \\
SP-LIME &\faCheckCircle&& & \faCheckCircle &              & \faCheckCircle  \\
Class Model Visualization &\faCheckCircle&&              & \faCheckCircle          &              & \faCheckCircle                 \\
% TCAV \cite{kim2018tcav}                                 &\faCheckCircle&&              & \faCheckCircle          &              & \faCheckCircle           &              & \faCheckCircle          &                  \\
LORE &&\faCheckCircle& \faCheckCircle & &  & \faCheckCircle \\
Anchors &&\faCheckCircle& \faCheckCircle & &  & \faCheckCircle  \\
DeepRED   &&\faCheckCircle& \faCheckCircle & \faCheckCircle &  & \faCheckCircle \\
GAM  &\faCheckCircle&&              & \faCheckCircle          & \faCheckCircle            &   \\
Decision Trees       &&\faCheckCircle& \faCheckCircle & \faCheckCircle          & \faCheckCircle            &               \\
BRL                   &&\faCheckCircle& \faCheckCircle & \faCheckCircle          & \faCheckCircle            &               \\
\hline
\textbf{LENs}                                           &&\faCheckCircle& \textbf{\faCheckCircle}    & \textbf{\faCheckCircle}  & \textbf{\faCheckCircle}  & \textbf{\faCheckCircle} \\
\end{tabular}
}
\vspace{0.3cm}
\caption{Summary of related work. \sm{The first column lists a number of approaches in the context of XAI. The other columns are about different properties. See the paper text for more details and for a description of all the approaches. }}
\label{tab:related_work}
\end{table}

Some of the most famous XAI techniques share the characteristic of being feature-scoring, local, post hoc methods.
Sometimes indeed, the easiest way to solve the explanation problem is simply to treat the model as a black-box and, sample-by-sample, determine which are the most important features for a prediction. 
Prominent examples of algorithms falling in this area %are Local Interpretable Model-agnostic Explanations (LIME) \cite{ribeiro2016should}, SHapley Additive exPlanations (SHAP) \cite{lundberg2017unified} and DeConvolution Neural Network (DeConv) \cite{zeiler2014visualizing}, which
accomplish this task by perturbing the input data. 
Local Interpretable Model-agnostic Explanations (LIME) \cite{ribeiro2016should} trains a white-box model (e.g., a logistic regression) to mimic the predictions of a given model in the neighbourhood of the sample to explain. By analyzing the weights of the white-box model it identifies the most important \sm{group} of pixels (superpixel).
Differently, SHapley Additive exPlanations (SHAP) \cite{lundberg2017unified} computes the Shapley value of each feature by removing each of them \sm{in an iterative manner}. %provides for local explanations by computing each input feature contributions in a certain prediction. In the Kernel SHAP version, the Shapley values of each feature are calculated by iteratively removing features in a similar way to what is done in LIME.
% Deconvolutional Network were initially introduce in \cite{zeiler2011adaptive} for unsupervised learning.
% Firstly introduced in \cite{zeiler2011adaptive}, DeConvolution Neural Network (DeConv) are used in \cite{zeiler2014visualizing} to %visualize the activation of a convolutional layer. In particular, they 
%visually determine pixel importance for a certain prediction by analyzing how the classification output changes when part of the input image is masked. 
Other important techniques %such as Activation Maximization \cite{erhan2010understanding}, Saliency Maps \cite{simonyan2013deep} and Gradient Class Activation Mapping (Grad-CAM) \cite{selvaraju2017grad} 
provide the same type of explanations through gradient analysis. %Differently from the previous one, however, they determine feature importance  %in the context of Convolutional Neural Network (CNN). 
Authors of Activation Maximization \cite{erhan2010understanding} firstly introduced this idea as an optimization problem. They explain the behaviour of a hidden/output unit by slightly modifying a given input data such that it maximizes its activation. An easier way to identify features causing a certain output has been found with Saliency Maps \cite{simonyan2013deep}, which project the classification loss until the input image. 
% A further improvement has been introduced with Gradient Class Activation Mapping (Grad-CAM) \cite{selvaraju2017grad} which allows to identify both class-specific image area and counterfactual explanations.
%They achieved this by modifying global average pooling with class activation mapping which allows to identify important image area with a single forward pass.
%
Other post hoc methods have been devised to extract global feature-scoring explanations, often starting from local explanations. %like LIME for Global Explanations \cite{ribeiro2016should} based on perturbation and Class Model Visualization \cite{simonyan2013deep} or Testing with Class Activation Vectors \cite{kim2018interpretability} based on Backpropagation. 
A submodular-pick algorithm extends the LIME module (SP-LIME) in %LIME for Global Explanations 
\cite{ribeiro2016should} to provide global explanations. SP-LIME first finds superpixels of all input samples with the standard LIME module. Successively, it finds the minimum number of common superpixels that covers most of the images.
Starting from the idea of Activation Maximization, Class Model Visualization \cite{simonyan2013deep} finds the input sample that maximizes a certain class probability score in the whole input space. %Differently from Activation Maximization, here the input sample is not searched in the neighbourhood of a given sample, but in the whole input space. 
Differently, LENs take a quite different perspective with respect to these methods, \sm{still inheriting several of their properties (see Tab.~\ref{tab:related_work})}. A LEN aims at providing human comprehensible decision support in terms of a set of FOL rules.


Explanation methods, indeed, can also supply FOL explanations. 
LOcal Rule-based Explanations of black-box decision systems (LORE) \cite{guidotti2018local} extracts FOL explanations via tree induction. \sm{The authors of \cite{guidotti2018local}} focus on local rules extracted through input perturbation. For each sample to explain, a simple decision tree is trained to mimic the behaviour of the black-box model in the neighbourhood of the sample. Both standard and counterfactual explanations can then be extracted  following the branches of the tree. 
Again based on LIME, Anchors \cite{ribeiro2018anchors}  also provides local rules of black-box model prediction via input perturbation. In this case, rules are not extracted from a decision tree but are generated by solving a Multi-Armed-Bandit beam search problem. 
Extending the CRED algorithm \cite{sato2001rule}, DeepRED  \cite{zilke2016deepred} employs a decomposition strategy to globally explain neural networks. Starting from the output nodes, each node in a layer is explained in terms of the activations of the previous ones through a decision tree. In the end, all rules for each class are merged in a single global rule in terms of input nodes only. For a single example a single local rule can be extracted following the firing path. 
The approach proposed in this paper is in some sense similar to the DeepRED algorithm. Indeed, \sm{as it will become clear in the following sections}, LENs can explain the behaviour of a neural network both end-to-end and layer by layer. However, LENs can be used to explain any black-box model as far as its input and output are interpretable (Section~\ref{sec:basics}). \sm{Furthermore}, LENs support different forms of FOL rules, with different scopes and goals.

Interpretable models are generally capable of providing both local and global explanations. These explanations may be based again on feature-scoring as in Generalized Additive Models (GAM) or on FOL rules as in Decision Tree \cite{breiman1984classification} and Bayesian Rule Lists (BRL) \cite{letham2015interpretable}. Meant to overcome the non-linearity assumptions of Linear regression, GAM learns to predict the given class for each feature via decision tree. In \cite{caruana2015intelligible}, authors proposed GA$^2$M where attribute interaction is allowed at a pair level. Recently a further extension employing neural network as non-linear function has been proposed in \cite{agarwal2020neural}, which, however, lose interpretability at feature-level.
Decision trees are a greedy learning algorithm which iteratively divides input data into smaller subsets until they only contain elements belonging to the same class. Different pruning algorithms have been also proposed to simplify the resulting structure and therefore the explanations \cite{quinlan1987simplifying}. Each path of a decision tree may be seen as a decision rule\sm{, i.e.,} an \textit{IF-THEN} statement. 
The set of rules may be generated in different ways, either with sequential covering as in \cite{cohen1995fast} or by selecting the best rules from a pre-mined set via Bayesian statistics as in BRL. 
%
\sm{Interestingly, LENs} can be \sm{directly} used to solve a learning task, being almost interpretable per se. 
Employing an interpretable by-design neural network as classifier has the advantage that the extracted explanations will perfectly match the classifier predictions. 
In addition, relying on a neural network, LEN generalization performance can be much better than standard interpretable-by-design methods, that generally have a very limited representation capacity.

Summing up, the proposed approach can be used both as interpretable model and explanation method. \sm{Indeed, the flexibility of LENs allows the user to find an appropriate trade-off between interpretability and accuracy that is well suited for the task at hand.} 
The explanation type of LENs is in terms of FOL rules and different explanation styles, corresponding to different \sm{types} of logic formulas. Such explanations are extracted with different scopes, from local rules valid on a single sample to global rules \sm{that hold} for an entire class.





\section{\sm{Logic} Explained Networks}
\label{sec:basics}
%%%%%%%%%%%%%%%%%%%%%%%%%%%%%%%%%%%%%%%%%%%%%%%%%%%%%%%%%%%%%%%%%O
%%%%%%%%%%%%%%%%%%%%%%%%%%%%%%%%%%%%%%%%%%%%%%%
% NOTATION REMINDER
%\fg{mettere in tabella es alla fine del 2.1?}
% {\color{red}
% \textbf{Notation}
% X = input space (non-interpretable)\\
% Y = symbolic output space (interpretable)\\
% C = symbolic "concept" space (interpretable)\\
% E = symbolic "rule" space (interpretable)\\

% n = \# samples\\
% d = \# features of X\\
% q = \# categories of Y\\
% k = \# categories of C\\
% r = \# categories of E\\
% }
%%%%%%%%%%%%%%%%%%%%%%%%%%%%%%%%%%%%%%%%%%%%%%%
% DISCORSINO intro su cosa è il nostro modello, cosa fa, a cosa si appoggia.. caratteristiche generali


% Differently from several existing XAI models, 
We consider a general framework in which a special kind of neural network, \sm{referred to as Logic Explained Network (LEN), is used to make predictions and provide explanations about them, or it is used to}  explain the behaviour of another classifier, \sm{being} it another neural network or \sm{another generic} black-box model. \sm{Moreover, a LEN might also be used to explain relationships among some given data.}
%LENs can be defined according to different criteria and exploited in different use cases. 
\sm{In this section we will formally introduce LENs and the notation used throughout the paper. Then, instead of immediately diving into the internals of LENs (Section~\ref{sec:methods}), we will focus on
the different ways in which LENs can be set up. In particular, we consider how LENs can be instantiated in the framework of Fig.~\ref{fig:len}, discussing a variety of computational pipelines (Section~\ref{sec:use_cases}), and on the type of explanations that we can ask the LEN to generate (Section~\ref{sec:explanation_styles}).} %Fig.~\ref{fig:scheme1} provides an overview of the main topics covered in this section.

\iffalse
\begin{figure}[h]
    \centering
    % \includegraphics[width=0.7\textwidth]{figs/scheme1.png}
    \includegraphics[width=0.6\textwidth]{figs/lens_1.pdf}
    % \input{tikz/framework}
    \caption{\sm{Basics of LENs (Section~\ref{sec:basics}). In order to setup a LEN-based model, first, the way the LENs communicate with a black-box classifier or directly with the data must be defined (what we refer to as computational \textsc{pipeline} Section~\ref{sec:use_cases}). The type of expected explanations has a direct consequence in the objective that drives the learning of the LENs parameters (\textsc{learning and explanations}, Section \ref{sec:explanation_styles}). {\color{red}[Remove the word 'explainer' from the 3 points in Pipeline.
    Remove the word 'explanations' from the white box on the right.]} } 
    }
    \label{fig:scheme1}
\end{figure}
\fi

%There are different ways of letting LENs communicate with a black-box classifier

%and for which
%the main aspects on what LENs can be used for and which kind of explanation we may get with 
%learning problems it applies (see Fig. \ref{fig:scheme1}).

%Let us consider a standard classification problem where a classifier f defines the membership values of

\sm{A LEN is a function $f$, implemented with a neural network, that map data falling within a $k$-dimensional Boolean hypercube onto data that fall within another $r$-dimensional Boolean hypercube. Each dimension is about the activation strength of what we refer to as \textit{concept}, with the strict requirement of having a human-understandable description of each \textit{input} dimension/concept. 
Formally, LEN is a mapping $f: C \rightarrow E$, \sm{where $C = [0,1]^{k}$ is the \textit{input concept space}, and $E = [0,1]^{r}$} is the so called \textit{output concept space}. Explanations are given in terms of the input concepts, while the $r$ output concept activations are about the truth degrees of $r$ FOL rules. Whenever a LEN has been trained, the $i$-th output concept can be directly translated into a FOL rule $\varphi_i$ such as the one shown in Fig.~\ref{fig:len}. Rules can be then aggregated to different extents, altering their granularity level from a local to a more global coverage of the available data.
}

\sm{In order to provide a concrete meaning to the LEN model, we have to define the source of the input concept activations and how to learn the criteria that allow LENs to predict the output concepts/rules. Amongst a variety of possible configurations that are instance of Fig.~\ref{fig:framework}, we will focus on a finite set of computational pipelines in which the input and output concept spaces are defined with respect to real-world use-cases. In some of them, LENs communicate with a black-box classifier, with the goal of providing explanations of its predictions, or with the goal of exploiting its predictions to model the LEN input concept activations.
In all the cases, for each input sample, LENs provide $r$ FOL explanations that might be directly associated to $r$ categories of a classification problem or they could be interpreted as $r$ generic different explanations of the input data. In the former case, LENs are trained in a supervised manner, while in the latter case they are trained in an unsupervised setting.}

\sm{Before going into further details, we introduce the entities and the notation that will be used throughout the paper.
\begin{itemize}
\item We consider a scenario in which we have the use of a collection $\mathcal{X}$ of $n$ data samples belonging to $X\subseteq\mathbb{R}^d$ to train LENs. 
\item The notation $\mathcal{C}$ indicates a discrete set of $n$ elements belonging to the space $C$ of the input concepts. The data in $\mathcal{C}$ are directly associated to the data in $\mathcal{X}$, i.e., for each element in $\mathcal{X}$ there is a corresponding element in $\mathcal{C}$.
\item \sm{We use the notation $q$ to indicate the total number of classes in a classification problem. Each data sample can be associated with one or more classes. No strict conditions are posed on the potential mutual exclusivity of the different classes, thus we consider the most generic setting that spans from multi-label to single-label classification. Moreover, classes could also be organized in a structured manner, such as in hierarchy. Classes are encoded with binary targets belonging to $\bar{Y} = \{0,1\}^{q}$. We will use the notation $\bar{Y}_{(a:b)}$ to indicate a projection of $\bar{Y}$ limited to the dimensions going from index $a$ to index $b$ -- included. The function $\bar{y}(\cdot)$ returns the binary target vector associated to the data sample passed as its argument, while $\bar{y}_i(\cdot)$ returns the binary label restricted to the $i$-th class.} %The classification problem might also be structured in a hierarchical manner. In this case, at each level $\ell$ of the hierarchy we have $q^{(\ell)}$ classes, $\ell \in [1,h]$.
%\sm{In the case of hierarchically organized classes, the higher-level classes are predicted in function of the ones activated at the lower levels, $g^{(\ell)}: Y^{(\ell-1)} \rightarrow Y^{(\ell)}$, $\ell \in [1,h]$, where $Y^{(0)} = X$.}
\item The function $g$ is about a generic black-box neural classifier,
%\footnote{With "black box classifier" we mean that there are no assumptions on the classifier structure. The classifier architecture could be totally unknown to the logically explained network, that only requires a $[0,1]$-valued I/O.} 
 where $g: X \rightarrow Y^{(u)}$ defines the membership \sm{scores} of \sm{$x$} to $u$ categories, i.e.,  $g(x)=(g_1(x),\ldots,g_u(x))\in Y^{(u)}$, $Y^{(u)} = [0,1]^{u}$, $u\leq q$, with $g_i(x)=1$ (resp. $g_i(x)=0$) \sm{when} $x$ belongs (does not belong) to class $i$. \sm{The $u$ categories could be exactly the ones of the considered classification problem ($u = q$) or a subset of them ($u < q$). No special conditions are enforced in the definition of $g$.}
 \item The notation $\bar{f}$ is about a Boolean instance of function $f$, in which each output of $f$ is projected to either $0$ or $1$.\footnote{When not directly specified, we will assume $0.5$ to be used as threshold value to compute the projection.} In order to refer to a single output of the vector function $f$ (or $\bar{f}$), the subscript will be used, e.g., $f_i$ (or $\bar{f}_i$). Similarly, for a vector $c \in \mathcal{C}$ with activation scores of concepts, $c_i$ is the $i$-th score, while $\bar{c}_i$ is the Boolean instance of it.
 \item The $j$-th dimension of space $C$ includes a human-readable label. FOL rules generated by LENs will exploit such labels to give understandable name to predicates. In order to simplify the notation, whenever we provide the FOL rule associated to a sample $c \in \mathcal{C}$, we will use the already introduced symbol $\bar{c}_i$ also to refer to the label of the $i$-th dimension. Similarly, in FOL rules, $\bar{f}_i$ will refer to the understandable name of the $i$-th output concept (when available).
\end{itemize}}
The listed elements will play a precise role in different portions of the LEN framework.




\iffalse
such that:
\begin{itemize}
    \item Any input $c\in C$ consists in a $[0,1]$-valued feature or concept vector, i.e. $C \subseteq [0,1]^k$. $C$ is also said the \emph{concept space}. Concepts need to be semantically meaningful since they will be exploited to provide explanations. Many times $X=C$ if $X$ is already semantically meaningful; otherwise a mapping is required.
    \item $f$ can be any neural model, but it is required that $E\subseteq[0,1]^r$ where, for any $c\in C$, $i=1,\ldots,r$, $f_i(c)=1$   means that the $i$-th explanation holds for $c$, viceversa if $f_i(c)=0$. $f_i$ is sometimes called the $i$-th output of the LEN $f$. We refer to $E$ as the \emph{explanation space}. In standard supervised problems $E=Y$, however, LENs can also be employed in other contexts.
    % \item there is no pair $c^i,c^j\in C$, such that $\bar{f}(c^i) \neq \bar{f}(c^j)$ and $\bar{c}^i=\bar{c}^j$, where the overline notation denotes the boolean discretization (thresholded at $0.5$) of values from $[0,1]$ to $\{0,1\}$ values.
\end{itemize}



In a broad sense, a \sm{LEN} for the classifier $g$ can be simply thought of as any neural model $f$ aiming at explaining the decision processes taken by $g$. 

The explanations will generally hold on different input sub-portions. In terms of FOL formulas, this means that the extracted rules will be satisfied on different subsets of the concept space. For instance, we may consider example-level explanations, i.e. explanations focusing on individual class assignments. Example-level explanations can be aggregated into clusters up to overall class-level explanations. However, we may also be interested in frequent co-occurrences or global principles among different classes.




% One of the main advantage of the proposed framework is its versatility, indeed a LEN can be defined according to different user-preferences by serving different purposes. 
%In particular, the layout of a XAI pipeline based on LENs follows the definition of a few aspects concerning the classification problem under investigation and the properties of the required explanations. Setting these points allows the correct definition of a LEN in a learning problem. For clear, this is also schematized in Fig. \ref{fig:scheme1}.
LENs can be integrated in different learning problems with different classifier architectures. How the integration will take place depends on the nature of the input data and the presence of one or more concept bottlenecks among the classes under investigation. LENs can provide different kind of explanations both in supervised and unsupervised learning settings, according to user needs. 
%In particular, we may be interested in individual explanation, i.e. the explanation of the decision taken by the classifier on a specific sample. However, we may also look for more general explanations, such as explaining the decisions taken for a whole class predictions, or even looking for more abstract relations among the classes. 
Indeed, by now, we referred to LENs as neural networks aiming to accomplish a classification task. 
%(either to explain the behaviour of a black box or to solve the classification problem itself). 
However, LENs can also be used in unsupervised learning task. 
In the latter case, the output of the LEN denotes the cluster-assignment.
\fi


\begin{figure}[t]
    \centering
    %\includegraphics[width=0.55\textwidth]{figs/E2E.pdf}
    $\vcenter{\hbox{\includegraphics[width=.40\textwidth]{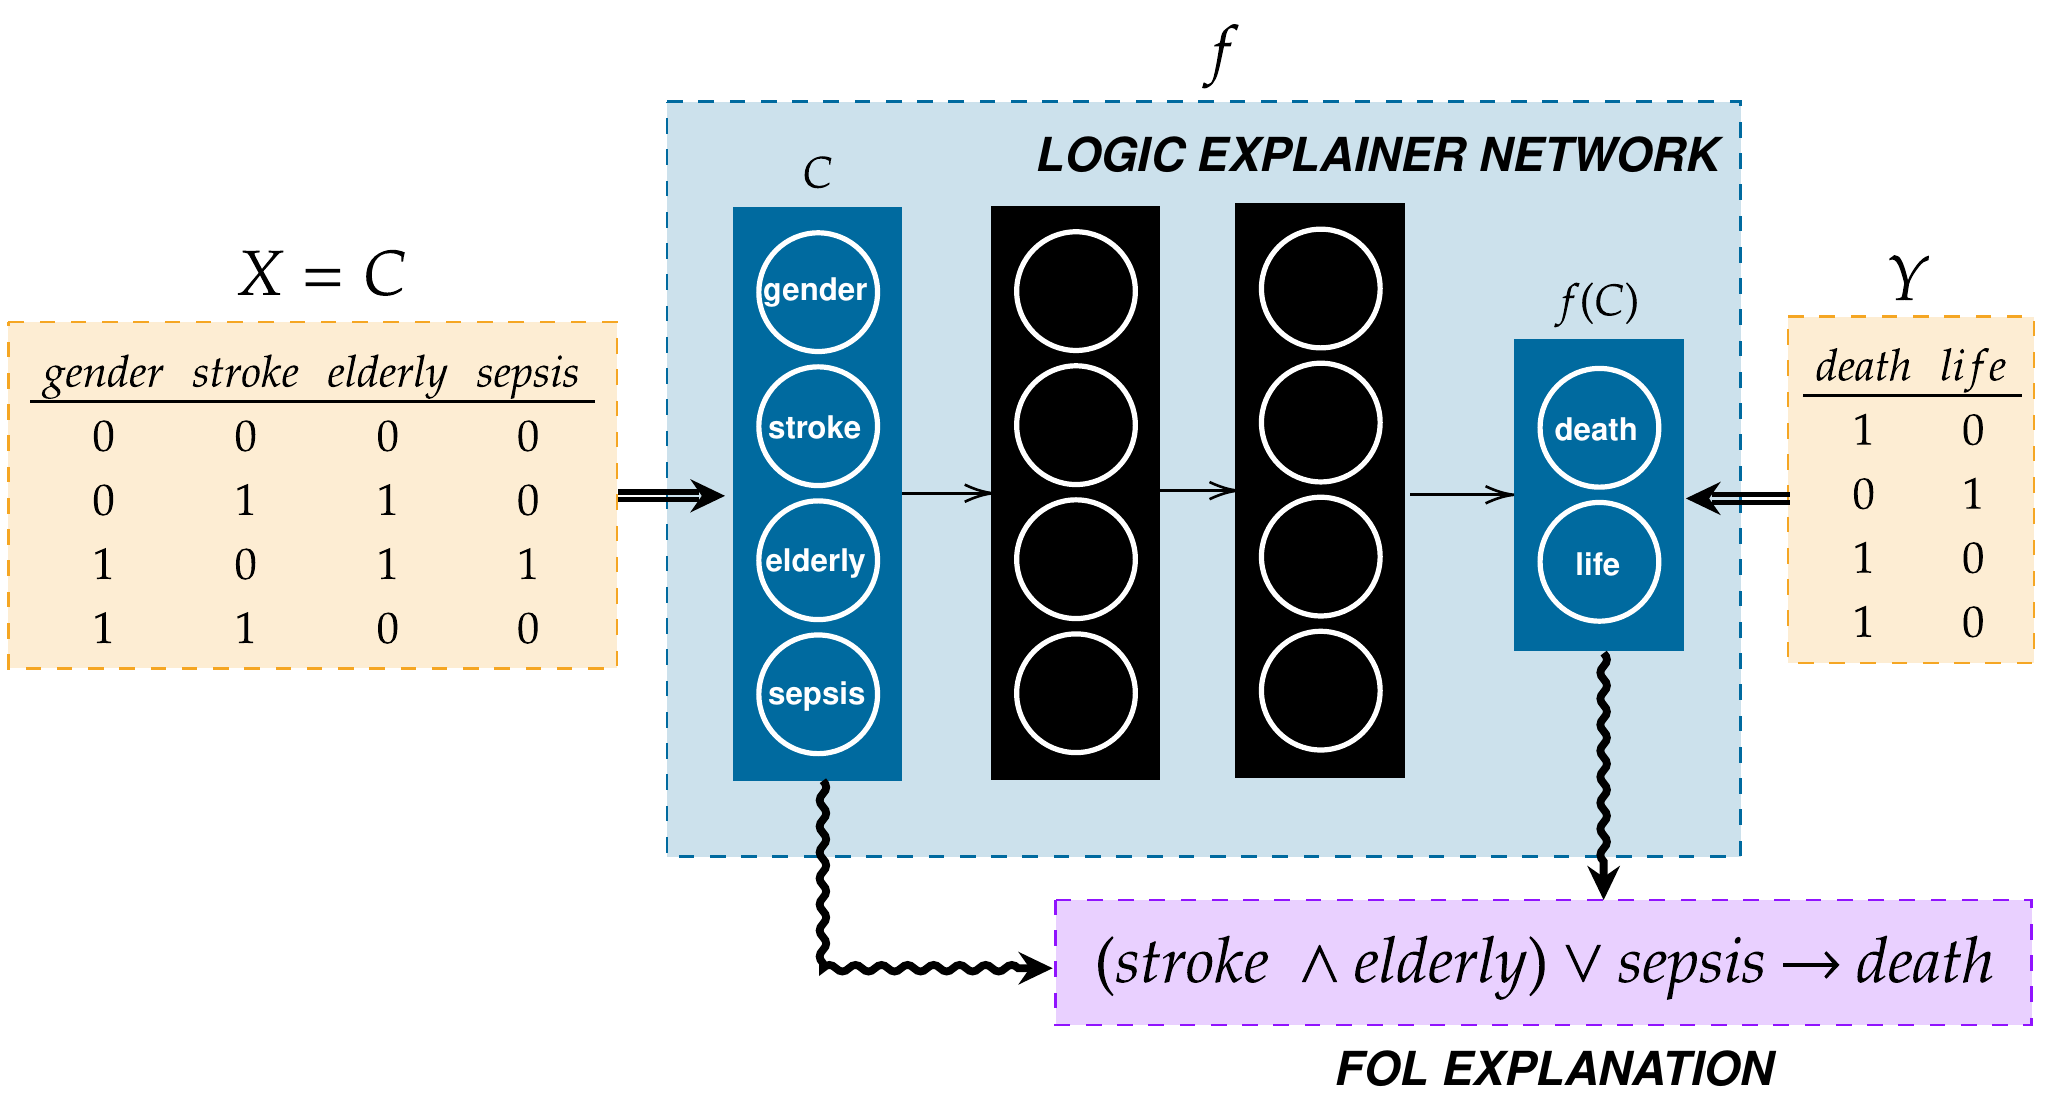}}}$ \quad %\\ \bigskip
    $\vcenter{\hbox{\includegraphics[width=.56\textwidth]{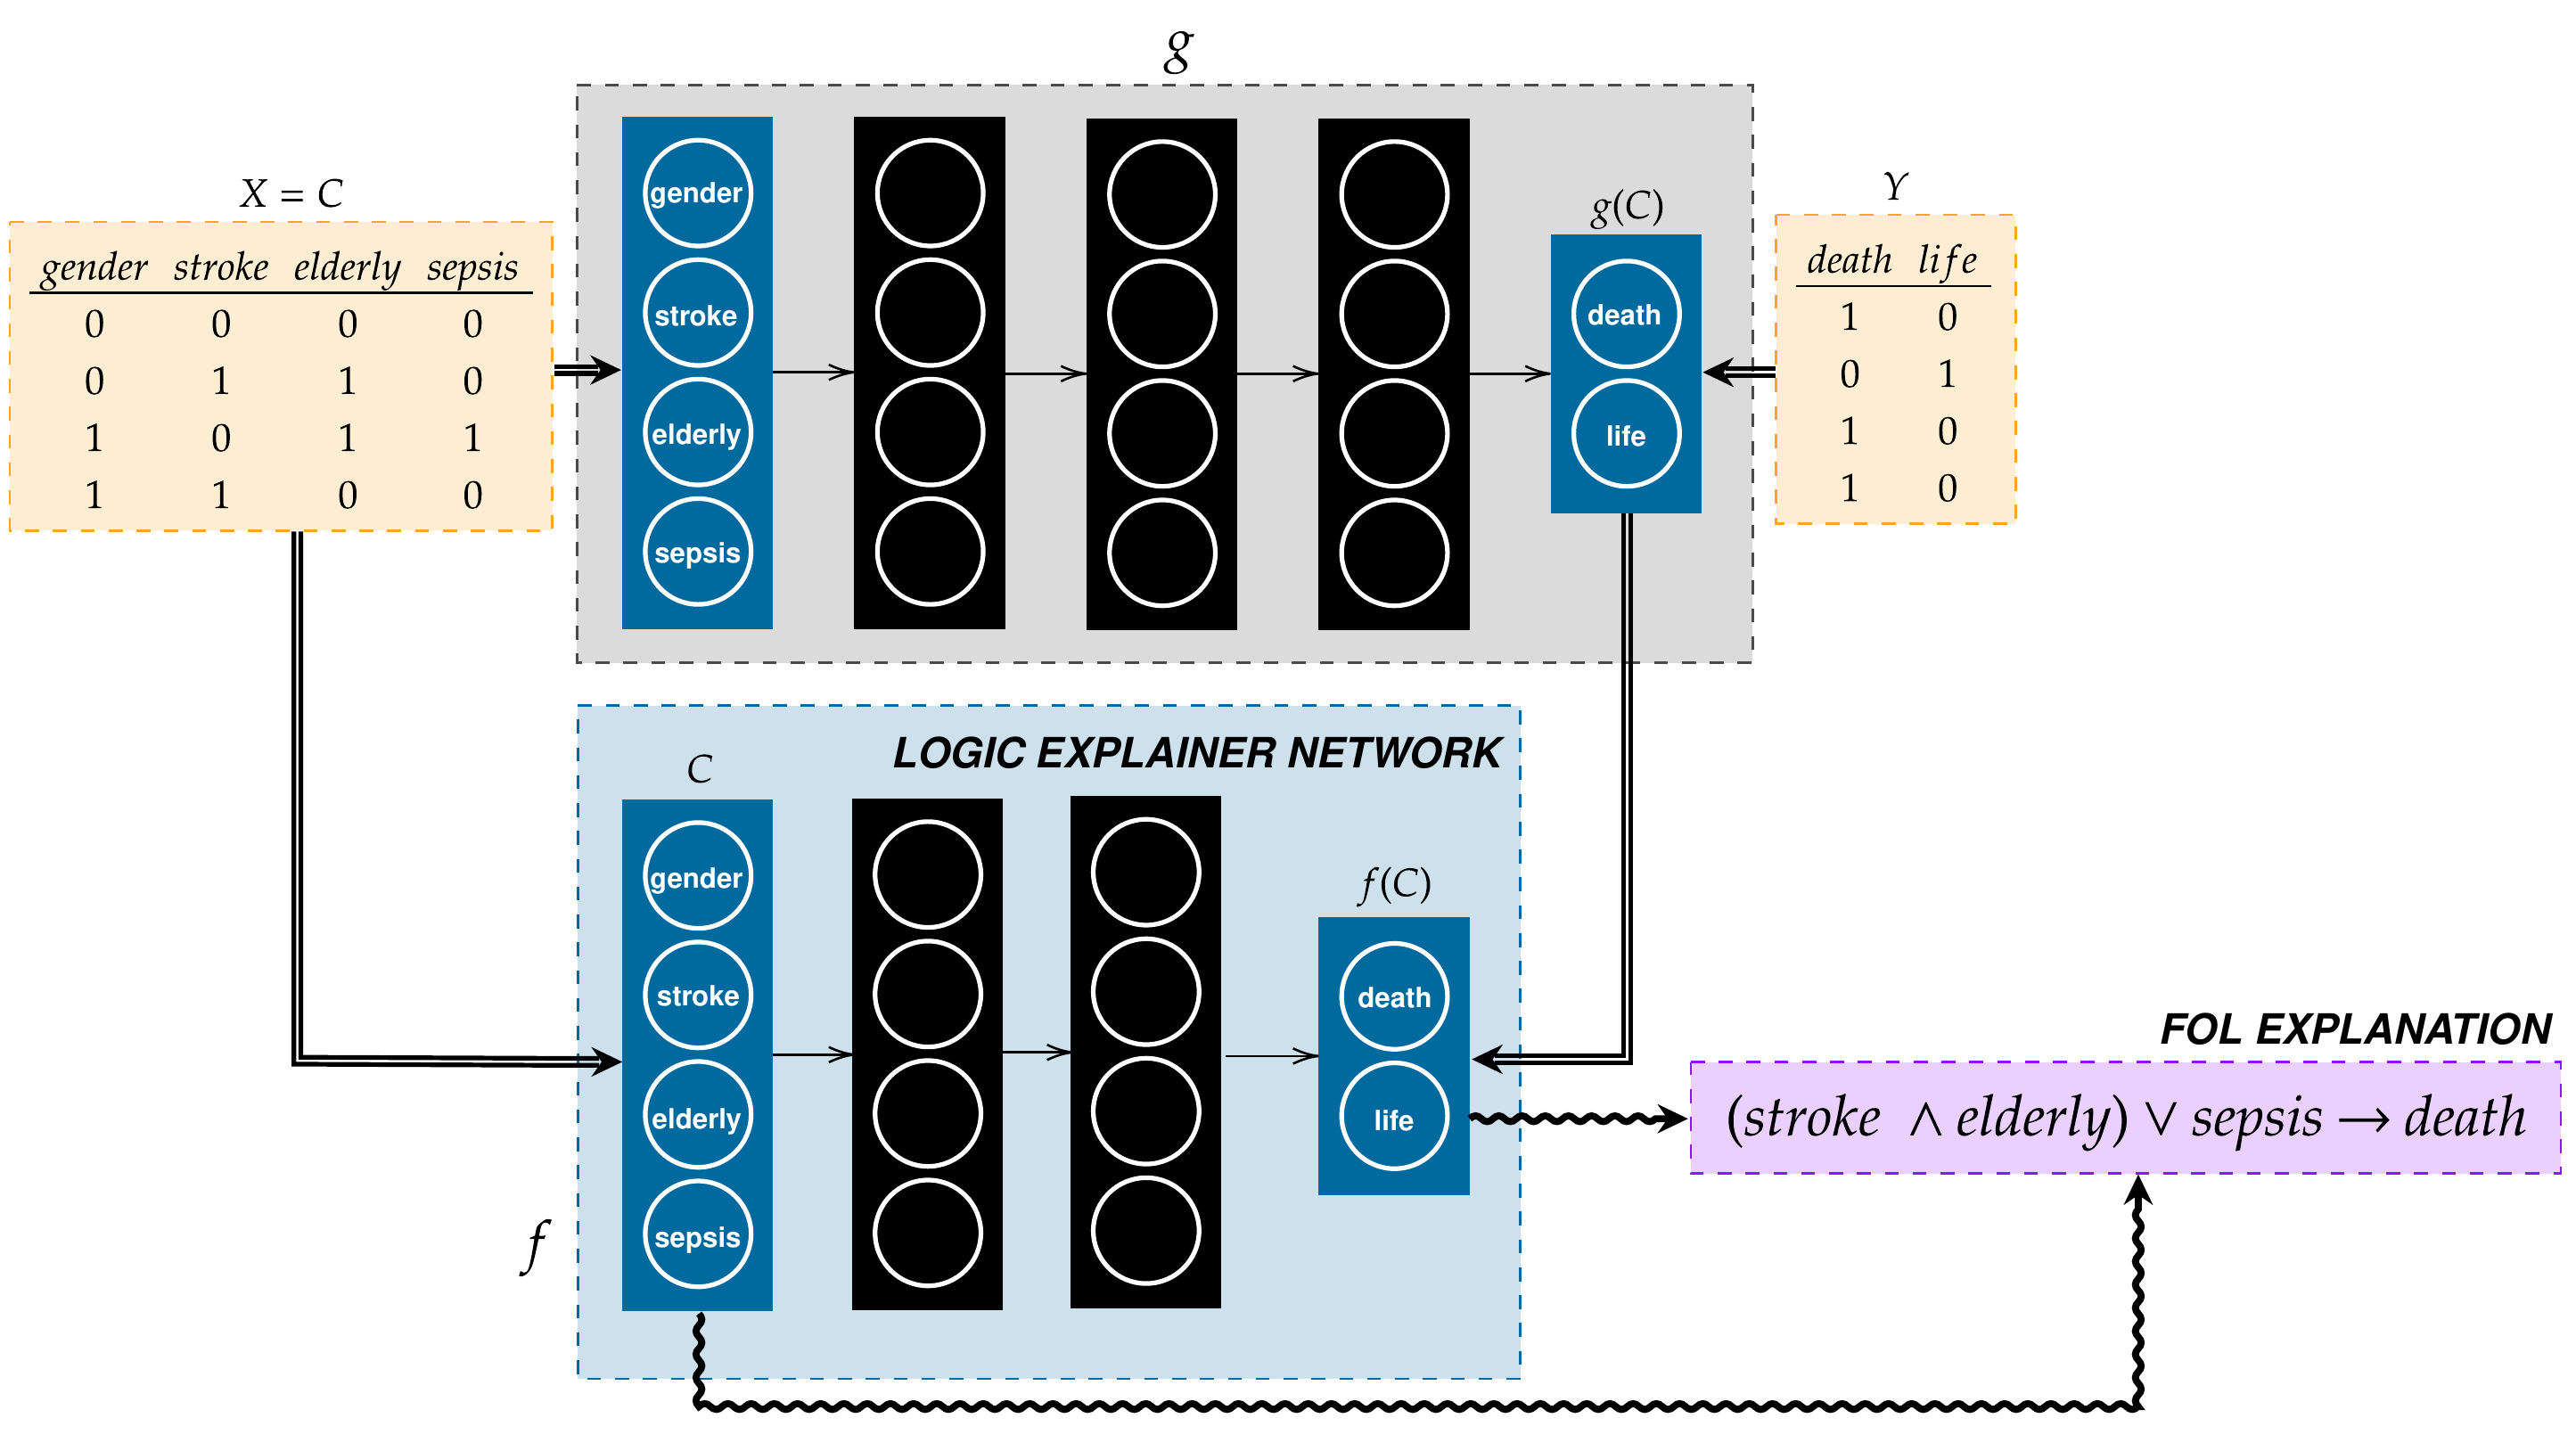}}}$    
    \caption{\sm{End-to-end (E2E) LENs} directly work on input data that are interpretable per se and treated as concepts ($C=X$), \sm{while the output concepts are the activation scores of the classes of the dataset ($r = q$)}. \sm{This is a real-world example from the} MIMIC II dataset \sm{(see the experimental section)}, where patient features are used to classify if \sm{the patient} will survive 28 days after hospital recovery. Left: the LEN solves the classification problem and provides explanation, also referred to as \textit{interpretable classification}. Right: the LEN \textit{provides explanations} of a black-box classifier. {\color{red}[Replace $X=C$ with $X$ (twice). Replace $C$ with $C=X$ (twice). Add $E=[0,1]^{q}$ in place of $f(C)$ (left only). Add $E=Y^{(q)}$ in place of $f(C)$ (right only). Replace $g(C)$ with $Y^{(q)}$. Replace $Y$ (twice) with $\bar{Y}$.]}}
    \label{fig:E2EExplainer}
\end{figure}

\subsection{Computational Pipelines} 
\label{sec:use_cases}
% In general, we can state that the above assumptions about the input data and the classifier are not always valid. However, in the following we will see how we can apply the LEN framework in different use cases where these conditions hold.
%Roughly speaking, a logically explained network $f$ is simply a function mapping $[0,1]$-values to $[0,1]$-values.
%, with the aim of providing itself the final classifications or to provide explanations for a classifier $g$. 
%This very general definition allows the application of LENs to different contexts that can be made consistent with real-unit I/O. 
%The most straightforward way of designing a computational pipeline involving LENs is to let the black-box classifier $g$ predict the activation scores of the $q$ classes and provide them to the LEN. In this way, we have $C = Y$, i.e., the LEN outpt concept space collides with $Y$. This is indeed feasible since $Y$ is bounded by a Boolean hypercube. %However, if the available data are already encoded in a symbolic manner in which the $d$ input features are actually  scores in $[0,1]$ (or in $\{0,1\}$ in the most extreme case) that can be considered the activation scores of $d$ concepts, then we can set $C = X$, and directly provide the data to the LEN. 
%The output space of the LEN can be designed in multiple ways, depending on what is the final goal of the whole system. For example, it could collide with $Y$, i.e., the output space of the black-box $g$, $E=Y$, or it could be a totally new concept space.}

\sm{Among a large set of feasible input/output configurations of the LEN block, here we consider three different computational pipelines that are about three concrete scenarios/use-cases where LENs may be applied, that consist in what we refer to as \textsc{end-to-end}, \textsc{concept bottleneck}, and \textsc{cascading} pipelines.}

%directly working on structured data; in a concept bottleneck-scenario where low-level concepts are first extracted from unstructured data (e.g. images); as a cascade of LENs providing explanations at different level of granularity.

%{\color{magenta}******* TBC ******}

% \paragraph{End-to-end explainer}
\textsc{End-to-end. } The most immediate instance of the LEN framework is the one in which the \sm{LEN block} aims at \sm{directly} explain, \sm{and eventually solve,} a \sm{supervised} categorical learning problem. \sm{In this case, we have $C = X$, and $r = q$, as shown in Fig.~\ref{fig:E2EExplainer}. In order to make the first equality valid with respect to the LEN requirements, the $d$ input features of the data in $X$ must be scores in $[0,1]$ (or in $\{0,1\}$ in the most extreme case), so that they can be considered as activations of $d$ human-interpretable concepts. }
%, i.e., $X=C \xrightarrow[]{f} E$. 
%An E2E LEN assumes that the features of the input space are meaningful individually, i.e. they correspond to human-interpretable concepts. 
%Structured datasets usually fall into this category. 
\sm{Of course, in order to create these conditions in different types of datasets, generic} continuous features can be either discretized into different bins or booleanized by comparing them to a reference ground truth (e.g., for gene expression data, the gene signature obtained from control groups can be used as a reference).
An E2E LEN can perform a fully \textit{interpretable classification} task, having the double role of main classifier and explanation provider (Fig.~\ref{fig:E2EExplainer}, left), or they can work in parallel with another neural black-box classifier $g$, thus {providing explanations} of the predictions of $g$ (Fig.~\ref{fig:E2EExplainer}, right) \sm{with $E = Y^{(q)}$} -- what we refer to as \textit{explaining a black-box}.
%used to explain the predictions of any black box model $g:X\rightarrow Y$, 
%as shown in Fig. \ref{fig:E2EExplainer}.
This first solution is preferred when it is of fundamental importance to have a white-box classifier, while we can accept some drawbacks in terms of classification performances, due to the constrained nature of the LENs.
The second solution is instead useful in those context where the classification performance plays a key role, and we may accept approximate explanations of the decision taken. 

\begin{figure}[t]
\centering
    %\includegraphics[width=0.55\textwidth]{figs/E2E.pdf}
    $\vcenter{\hbox{\includegraphics[width=.48\textwidth]{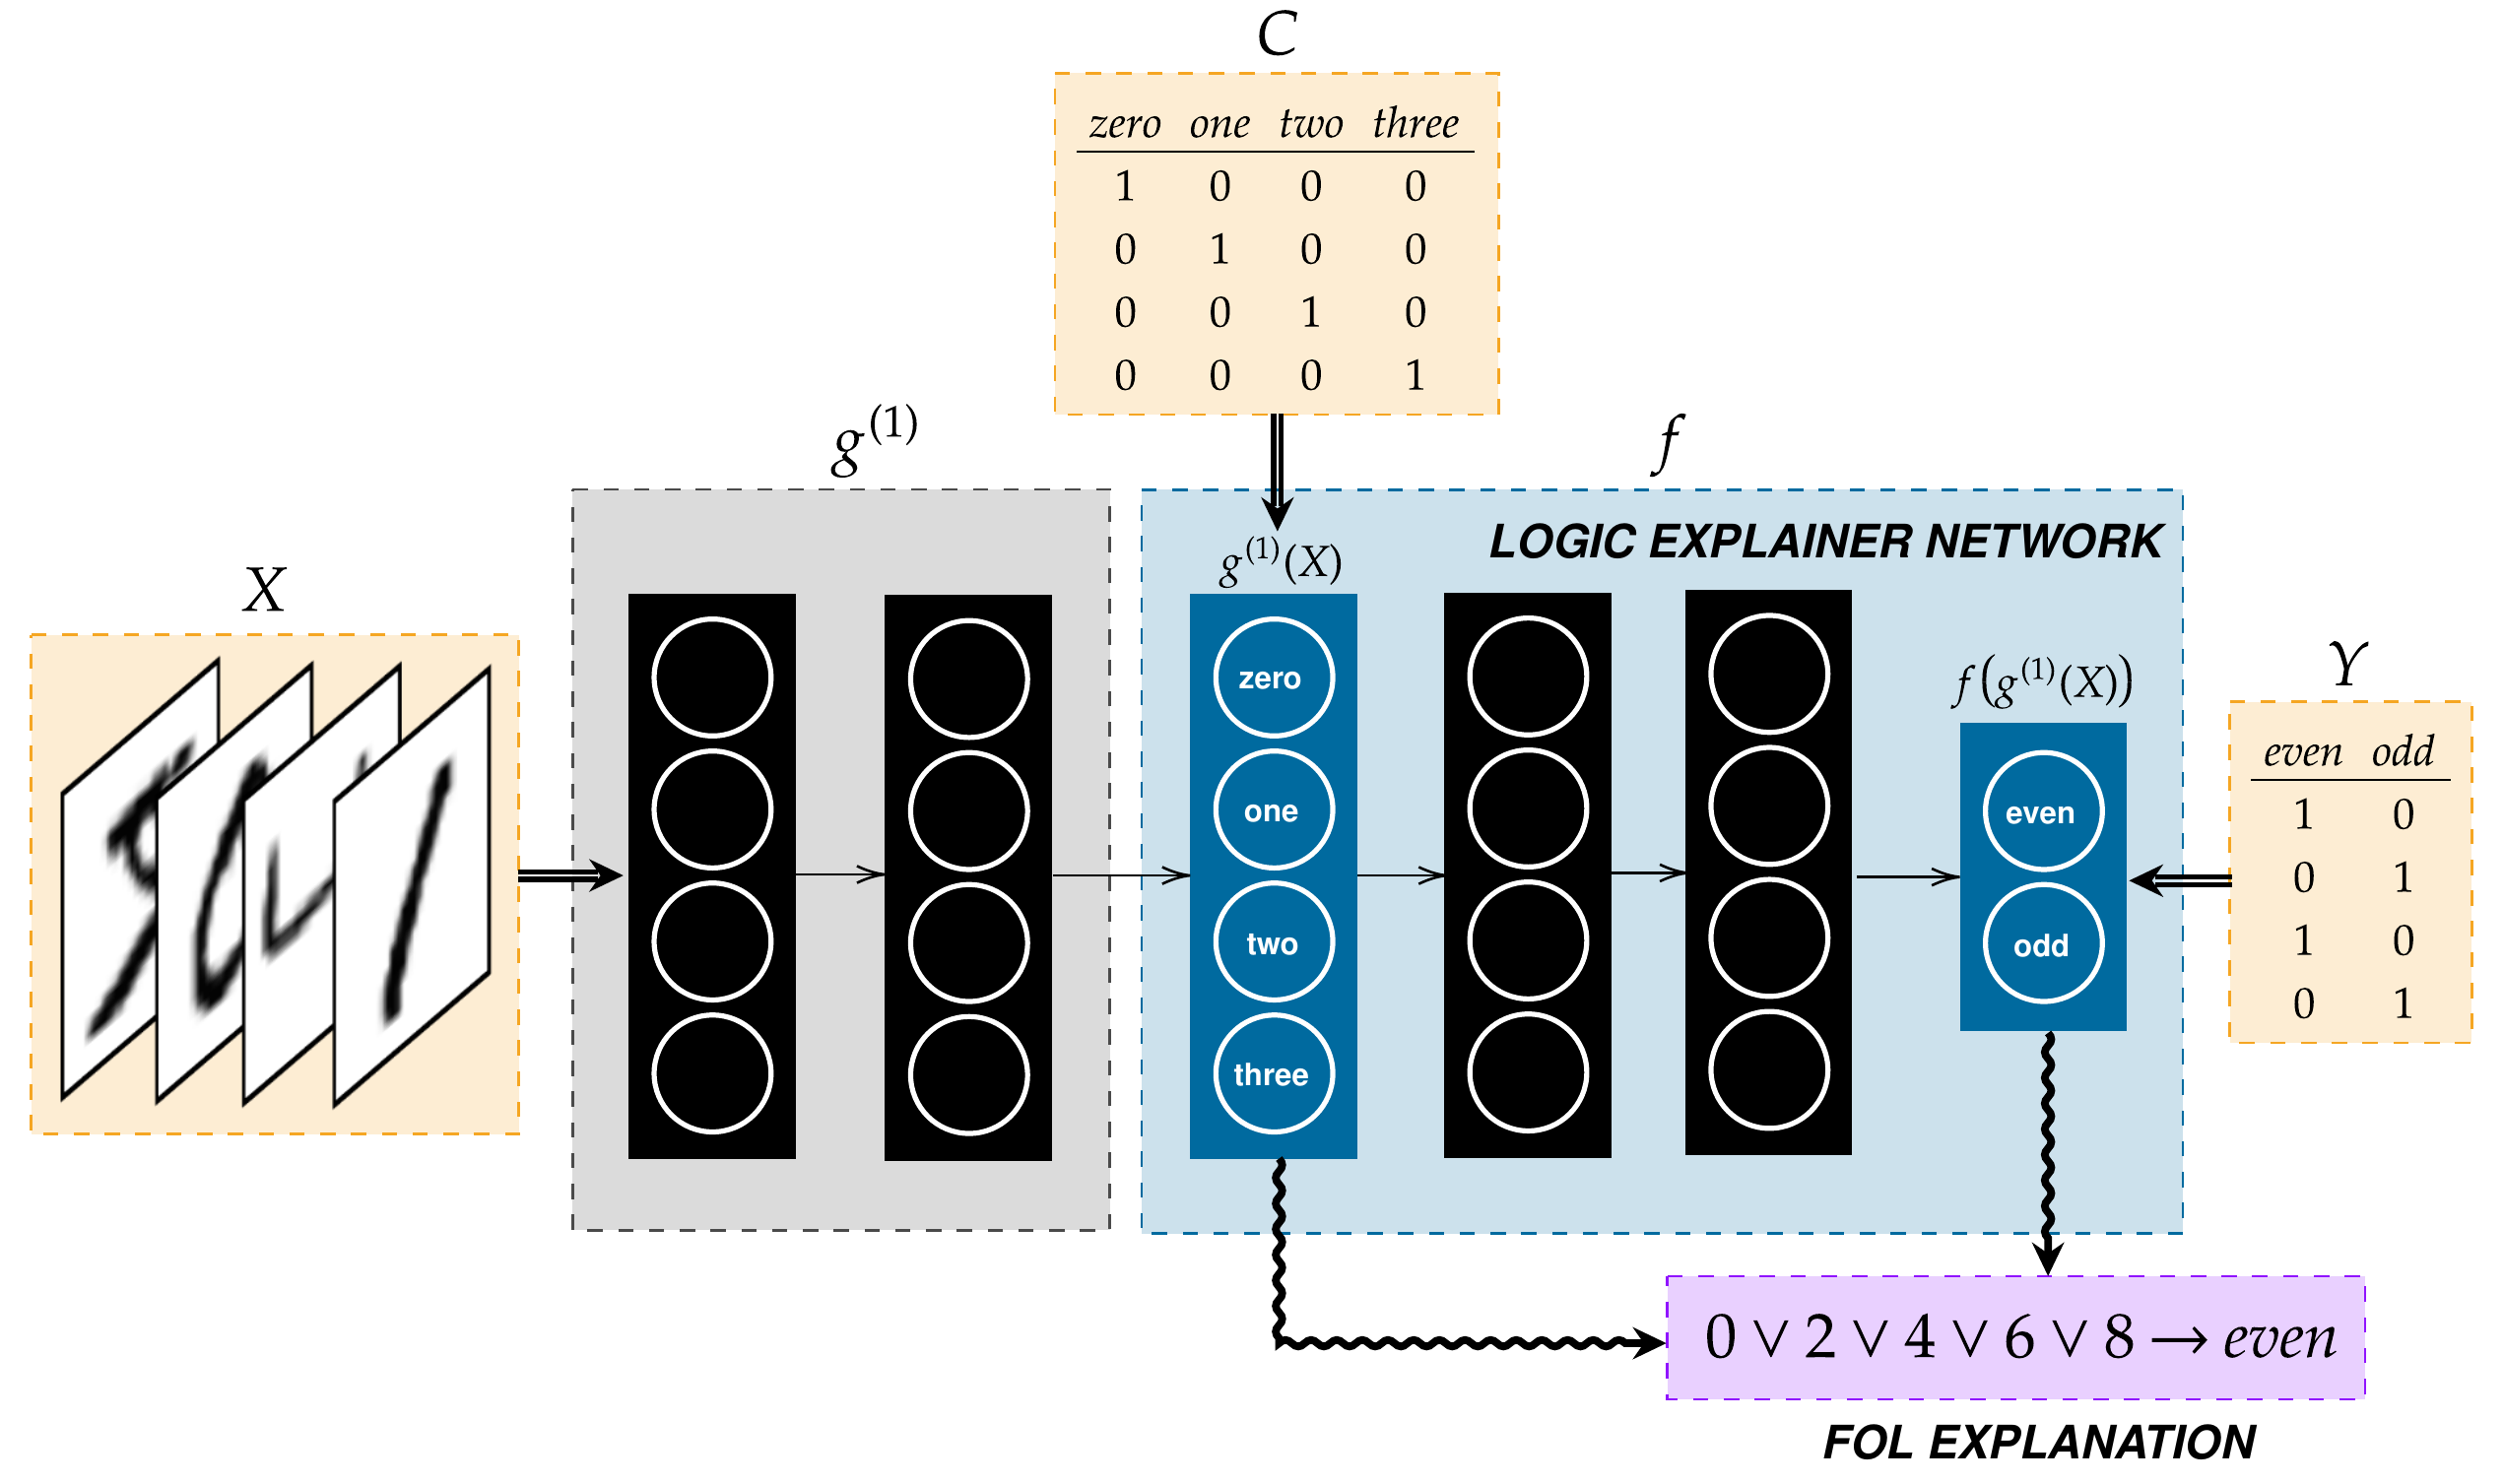}}}$ \quad %\\ \bigskip
    $\vcenter{\hbox{\includegraphics[width=.48\textwidth]{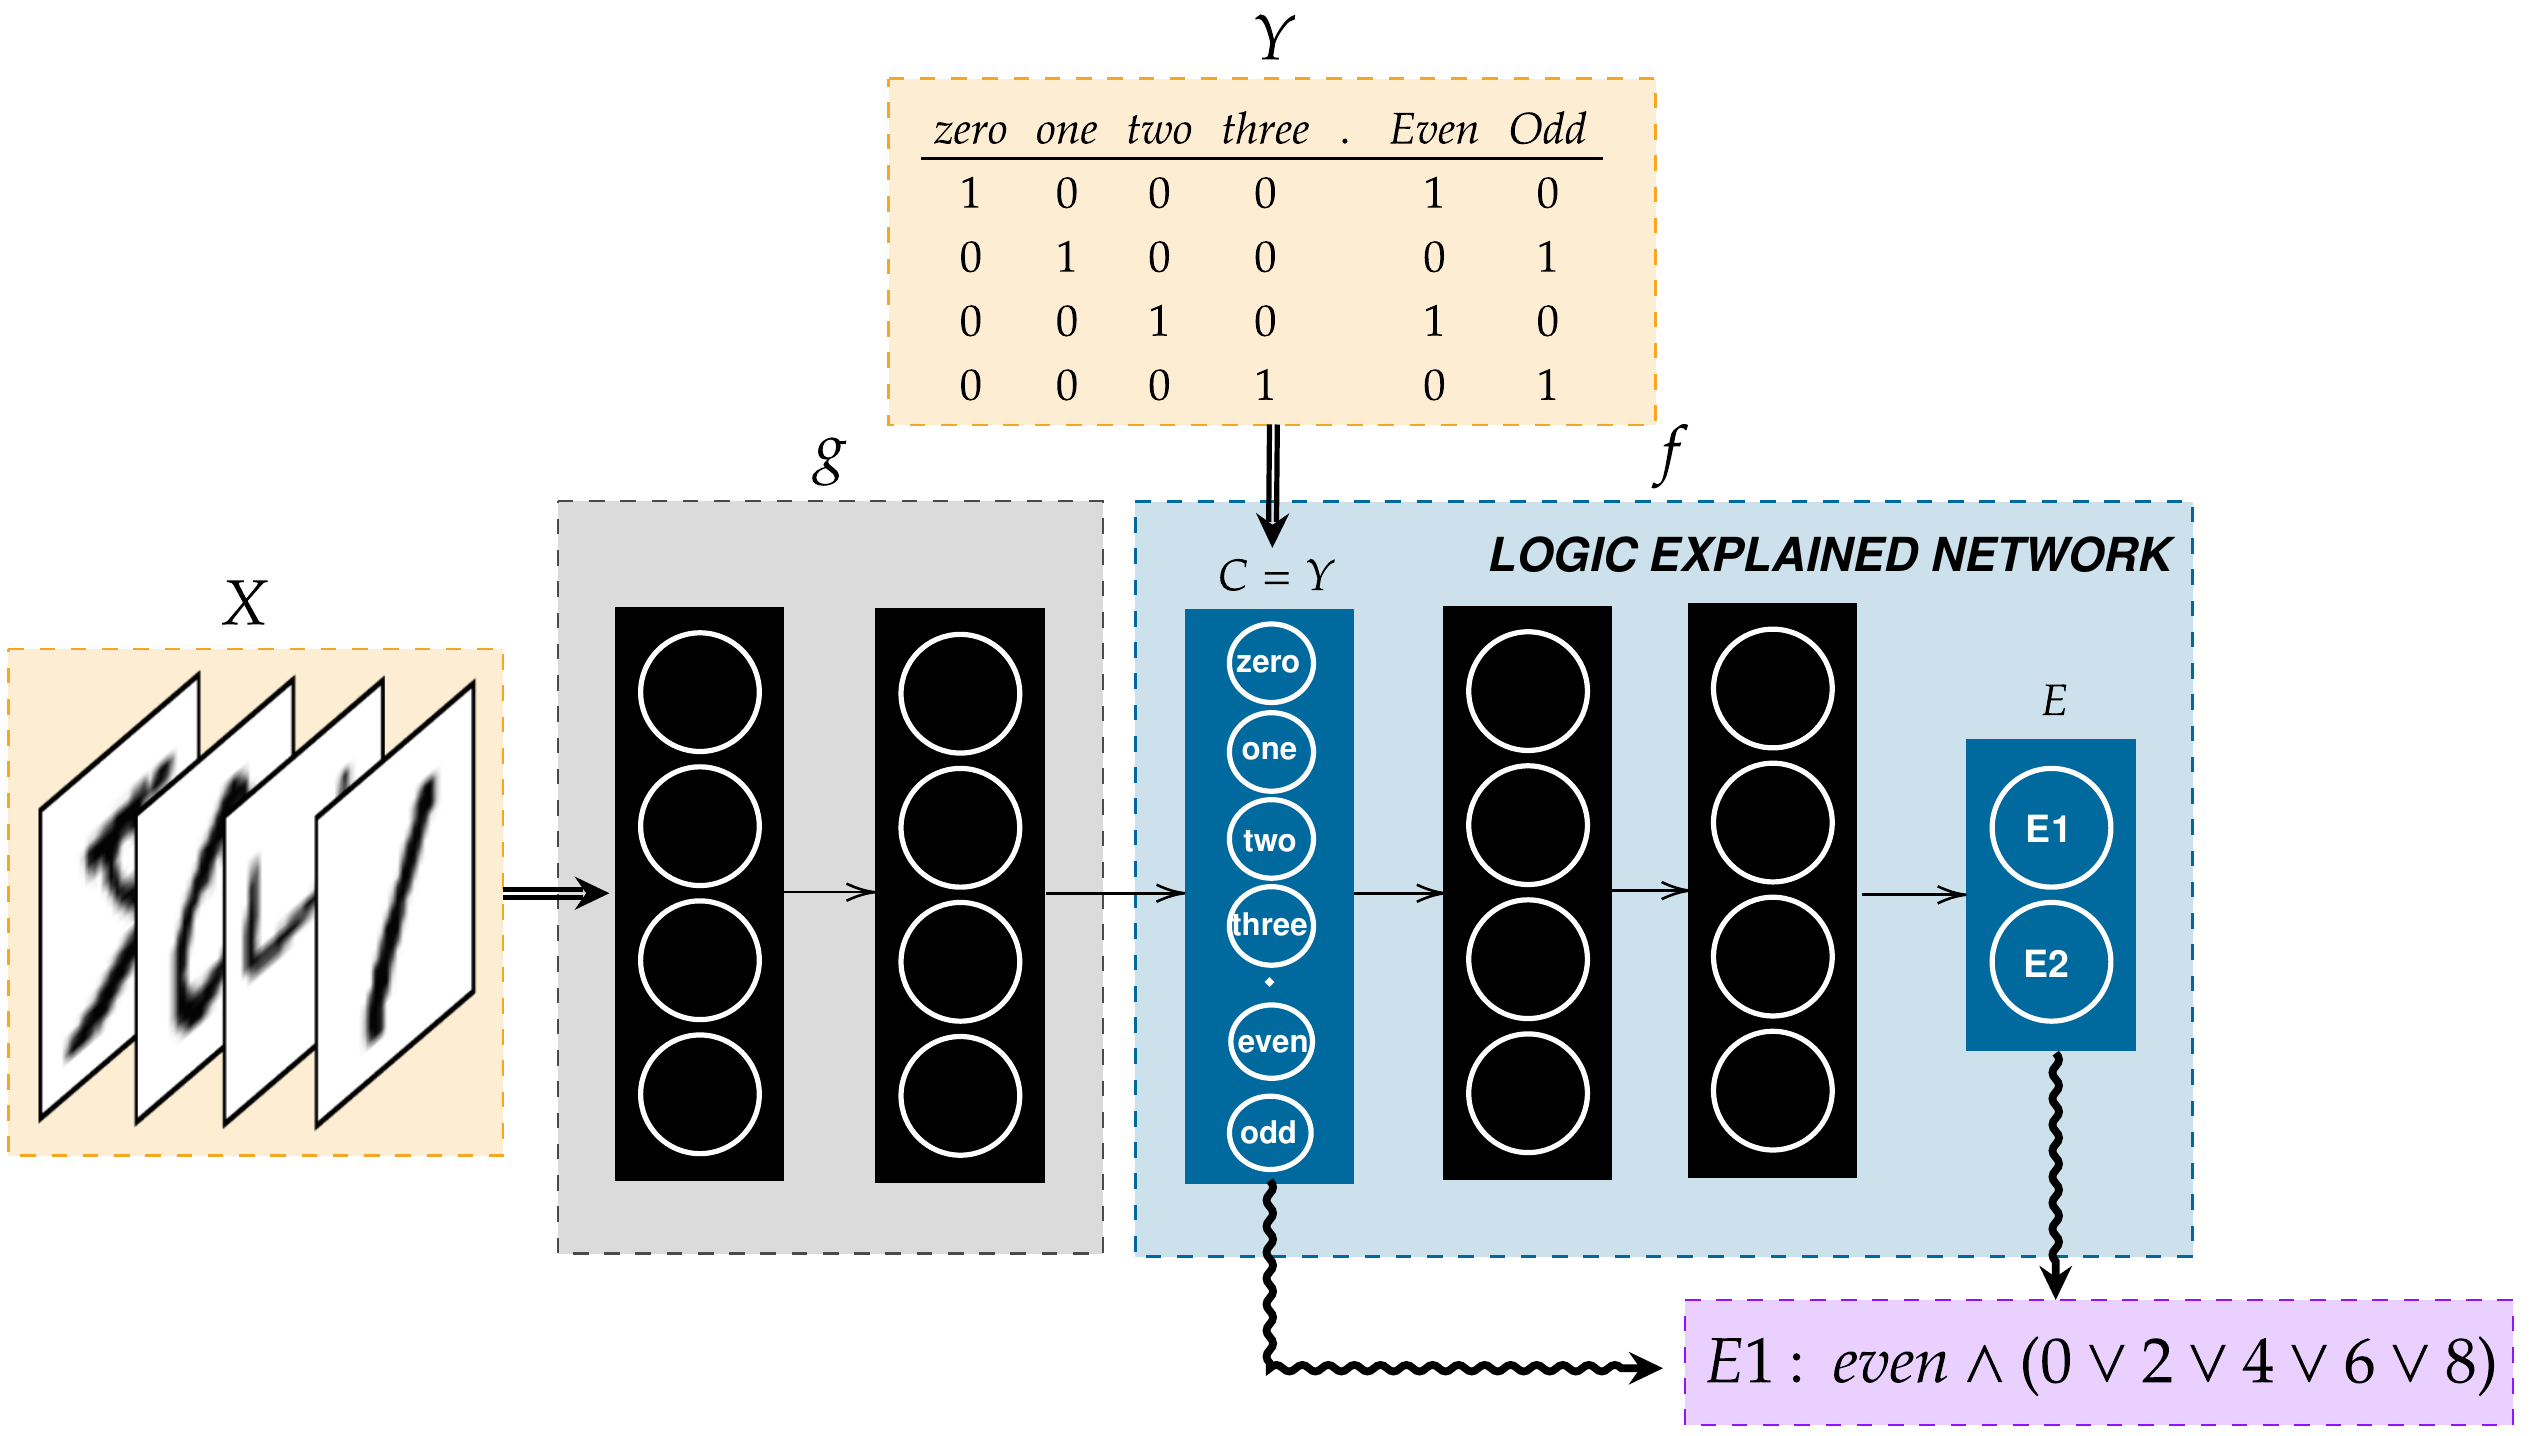}}}$       
    \caption{\sm{Concept-bottleneck (CB) LEN}. Left: the LEN is placed on top of a black box model $g$ which maps the input data into a first set of interpretable concepts. An MNIST-based experiments is shown \sm{(see the experimental section)}. Handwritten digits are first classified by $g$. A LEN is \sm{then} employed to classify and explain whether the digit is even or odd -- \textit{interpretable classification}. {\color{red}[Replace $g^{(1)}(X)$ on top of the blue column of concepts with $C=Y^{(z)}$. Replace $f(g^{(1)})(X)$ with $E=[0,1]^{(q-z)}$. Remove the superscript $(1)$ everywhere here. Replace the $Y$ on the right with $\bar{Y}_{(z+1:q)}$. Replace $C$ on top with $\bar{Y}_{(1:z)}$.]} Right: \sm{MNIST digits are classified as belonging to one of the 10 classes and whether they are even of odd by a black-box $g$ \sm{(see the experimental section)}.  %in a Concept-bottleneck pipeline 
     A LEN groups these predictions in an unsupervised manner, and analyzes the relations within each cluster -- \textit{interpretable clustering}.} Supervision labels are not provided for the LEN output. {\color{red}[Replace $g(X)$ on top of the blue column of concepts with $C=Y^{(z)}$. Replace  $f(g(X))$ with $E=[0,1]^{r}$. Fix FOL Explanation of Cluster 2 (not 1).]}}
    \label{fig:CMBExplainer} 
\end{figure}

% \paragraph{Concept-bottleneck explainer}
\textsc{Concept-bottleneck. } 
A Concept-Bottleneck (CB) LEN is a computational pipeline in which the LEN $f$ aims at explaining, and eventually solving, a categorical learning problem \sm{in which the data in $X$ are not readily exploitable as LEN inputs, and a black-box model $g$ computes the activations of an initial set of $z$ concepts out of the available data. The LEN solves the problem of predicting $r$ new concepts from the activations of the $z$ ones, as shown in Fig.~\ref{fig:CMBExplainer} (left/right). Differently from the E2E case, there is always a neural network $g$ processing the data, and the outcome of such processing is the input of the LEN. Formally, we have $g: X \rightarrow Y^{(z)}$, while $f: (C=Y^{(z)}) \rightarrow E$.} 
This two-level scenario can be implemented in a way that is coherent with the already discussed example of Fig.~\ref{fig:len}, that is what we also show in Fig.~\ref{fig:CMBExplainer} (left). In this case, each example is labeled with $q$ binary targets divided into two disjoint sets, where the black-box network predicts the first $z < q$ ones, and the LEN predicts the remaining $r = q-z$.
The LEN will be both responsible of predicting the higher level concepts and of explaining them in function of the lower level concepts yielded by the black-box model, thus still falling withing the context of \textit{interpretable classification}.
 We also consider the case in which the outcome of the LEN is not associated to any known classes, thus the LEN is trained in an unsupervised manner, as shown in  Fig.~\ref{fig:CMBExplainer} (right), thus implementing a form of \textit{interpretable clustering}. In both the cases, the black-box classifier $g$ is trained in a supervised manner.\footnote{The extraction process can be either implicit, through the analysis of the latent spaces learnt by the black-box \cite{kazhdan2020now}, or explicit by training a black-box to classify specific concepts \cite{koh2020concept}.}

%\sm{in which the features of the data in $X$ are not interpretable as activations of human-understandable concepts or they are too low-level to be directly involved into compact explanations} (e.g., all the pixels of an image \cite{koh2020concept}). In this case, we assume to have information to process the data in order to extract an initial set of concepts that will be provided to the LEN. 
%Then, given


%In this latter setting, a model $g$ can be used to extract high-level concepts $C$ from raw features in $X$, and then producing the final classification $Y$. In this case, we may assume $g=g^{(2)}\circ g^{(1)}$ with $X\xrightarrow[]{g^{(1)}}C\xrightarrow[]{g^{(2)}}Y$.
%Given the concepts extracted from $g$, a LEN $f$ may be exploited to produce a set of explanations $X \xrightarrow[]{g^{(1)}} C\xrightarrow[]{f}E$, 
% and eventually solve the classification task (if $E=Y$)
%classify and explain the categorical learning problem at a higher level of abstraction, i.e. $X \xrightarrow[]{g} C\xrightarrow[]{f}E$ %$C \xrightarrow[]{f} E$  
%as shown in Fig. \ref{fig:CMBExplainer} where $E=Y$.
% or even producing itself a solution by assuming $E=Y$.


\begin{figure}[t]
    \centering
    \includegraphics[width=0.58\textwidth]{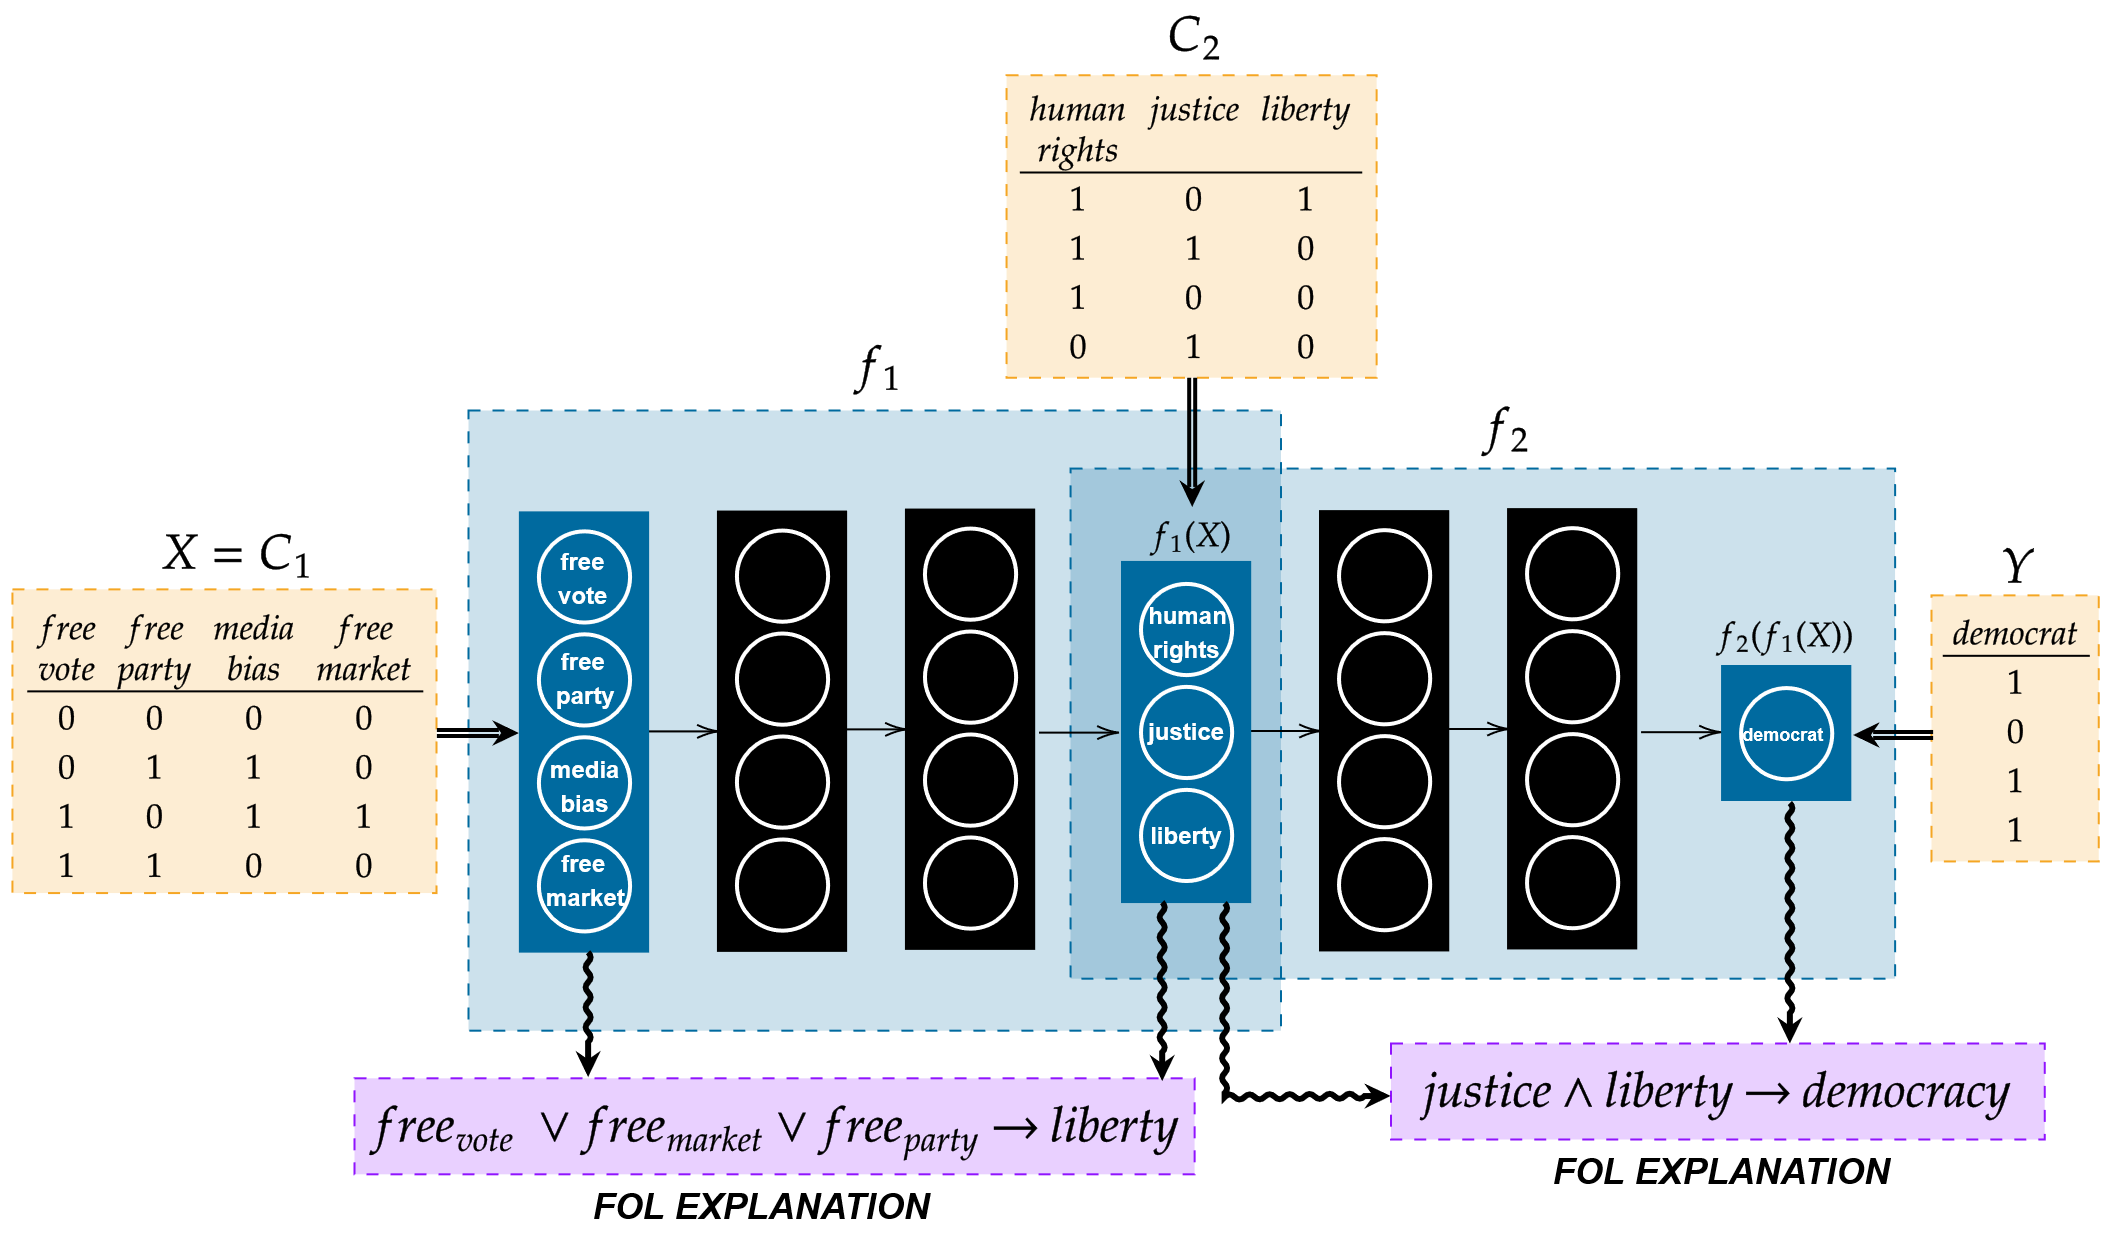}

      \caption{\sm{Cascading LENs}, \sm{an example taken from the V-Dem classification dataset (see the experimental section)}. The final classification on the status of the democracy is divided into two steps.
    %   $X=C^{(1)} \xrightarrow[]{f^{(1)}} C^{(2)}\xrightarrow[]{f^{(2)}} E$. 
    First, the input data/concepts $C_1$ are mapped into high-level concepts $C_2$. %$= f_1(X)$. 
    High-level concepts are then used to compute the final classification. %$= f_2(f_1(X))$. 
    Cascading LENs can provide explanations \sm{at different levels of granularity}, implementing multiple \textit{interpretable classifications}. {\color{red}[Replace $X=C_1$ with $X$. Add $C_1$ on top of the first column of blue concepts. Replace $f_1(X)$ with $E_1 = C_2$. Replace $f_2(f_1(X))$ with $E_2$. Replace $C_2$ on top with $\bar{Y}_{(1:z)}$. Replace $Y$ on the right with $\bar{Y}_{(z+1:q)}$.]}}
    \label{fig:CascadeExplainer} 
\end{figure}

% \paragraph{Cascading explainers}
\textsc{Cascading. }
Cascading LENs can be used to provide explanations by means of a hierarchy of concept layers. \sm{In particular, multiple LENs are used to map concepts into a higher-abstraction level (without the need of any black-box $g$), }%Each model is trained on a concept space to predict concepts at a higher level of abstraction which will feed the next LENs $C^{(i)} \xrightarrow[]{f^{(i)}} C^{(i+1)}$. 
%The final model solves and explains the more abstract classification task $C^{(m)} \xrightarrow[]{f^{(m)}} E$ 
as shown in Fig.~\ref{fig:CascadeExplainer}. \sm{Each LEN provides explanations of its outputs with respect to its inputs, thus cascading LENs handle multiple levels of granularity.} This structure provides a hierarchy of explanations and upholds human interventions at different levels of abstraction, providing a far deeper support for human-machine interactions. \sm{We indicate with $(C_1, E_1), (C_2, E_2), \ldots, (C_m, E_m)$ the input/output concept spaces of the $m$ cascading LENs, with $C_{j} = E_{j-1}$, $j > 1$. We will consider the case in which LENs are trained in a supervised manner, thus implementing multiple \textit{interpretable classifications}.}



\subsection{Learning \& Explanations}
\label{sec:explanation_styles}
%Different pipelines may be employed to solve different learning problems while (eventually) producing different explanations.
%In addition, 
\sm{Each LEN module can be trained in a supervised or an unsupervised fashion, according to the preference of the user with respect to the type of explanations generated by the LEN. %The user might be interested in finding explanations that hold whenever specific categories of the considered problem are predicted, }
% that hold on a certain portion of data 
%or \sm{in} letting the LEN \sm{autonomously discover a set of regularities among the input concepts.
In Section~\ref{sec:use_cases}, when describing the selected computational pipelines, we made a precise distinction among \textit{interpretable classification}, \textit{explaining a black-box}, and \textit{interpretable clustering}, that represent three different preferences that the user might have in the problem at hand. These preferences impose precise constraints in the selection of the learning criteria and on the form of the FOL rules that can be extracted by the LENs. In addition to this choice, the user can select the granularity level of the FOL rules, moving from \textit{local} to \textit{global} rules. The former are about single examples, while the latter covers the whole dataset. While all the formal details on the learning criteria and the rule types will be provided in  Section~\ref{sec:learncrit}, here we contextualize their role with respect to the properties of the previously described computational pipelines.} 

\sm{Whenever LENs are exploited to both solve the classification problem and provide explanations, i.e., in \textit{interpretable classification},  they become white-box classifiers. The examples of Fig.~\ref{fig:E2EExplainer} (left), Fig.~\ref{fig:CMBExplainer} (left), Fig.~\ref{fig:CascadeExplainer} are all about this case. Learning is driven by supervised criteria that exploit the available supervised data in order to create the conditions for extracting different types of FOL rules. Each output concept of the LEN is associated to a target category of the considered learning problem, and LENs can provide a FOL explanation of each prediction, e.g., explanation of the target class \textit{person} with respect to the input concepts/attributes \textit{head, hands, body}.}

\sm{In the case in which the user aim at \textit{explaining a black-box}, a LEN acts in parallel to a black-box classifier with the only goal of providing explanations, and it is forced to yield outputs that are as close as possible to the ones of the black-box, i.e., $f$ is forced to be close to $g$ on the available data samples. This is what is shown in  Fig.~\ref{fig:E2EExplainer} (right) and it does not require any supervisions, since learning is driven by a coherence criterion between the outputs of $g$ and those of $f$ when processing the same data.}

%
%For instance, in the selected computational pipelines of Section~\ref{sec:use_cases}, while most of the focus is on supervised learning, the Concept-bottleneck case is also about unsupervised learning of LENs (Fig.~\ref{fig:CMBExplainer} right).
%


%\sm{In the former case, each output concept of the LEN is associated to a target category of the considered learning problem, and LENs are developed by learning criteria that exploit the available supervisions (ection~\ref{sec:learncrit}). The rationale behind this approach it that LENs implicitly learn to predict each target class with respect to the input concepts, that are lower-level attributes. Then, LENs can provide a FOL explanation of such prediction, e.g., explanation of the target class \textit{person} with respect to the input concepts/attributes \textit{head, hands, body}. %We refer to this context as \textsc{targeted explanations}, and the learning process is driven by supervised criteria (Section~\ref{sec:learncrit}).
%\sm{Whenever the LEN belongs to a computational pipeline in which it is expected to both solve the classification problem and provide explanations, i.e., in \textit{interpretable classification}, then it becomes a white-box classifier. The examples of Fig.~\ref{fig:E2EExplainer} (left), Fig.~\ref{fig:CascadeExplainer} (left), Fig.~\ref{fig:CMBExplainer} are all about this case. 
%
%\sm{In the E2E case when $g$ is present or, more generally, whenever LENs act in parallel to a black-box classifier with the only goal of providing explanations, then LENs are forced to yield outputs that are as close as possible to the black-box, so $f$ is forced to be close to $g$. This is what is shown in  Fig.~\ref{fig:E2EExplainer} (right).
%
\sm{A user may be interested in discovering relations among different \sm{input} concepts without posing any preferences on any pre-defined class.
For example, the user might be interested in discovering  co-occurrences of certain input concept activations in not-defined-before subsets of the dataset, such as $soccer\_ball \wedge foot$ for some samples in a collection of miscellaneous images.
In the case of \textit{interpretable clustering}, each output concept of the LEN is associated to a symbol that is not defined in advance, as in Fig.~\ref{fig:CMBExplainer} (right), and the activation score can be tough as a cluster membership score.
LENs yield an explanation for each of these symbols, that is about discovering relations among the input concepts. In this context, no supervisions are exploited, and the learning criterion is designed in order to cluster the input concepts into $r$ groups.}

 %For instance, by analyzing the output of a multi-label classifier $C=g_1(X)$ in a CB pipeline, %with eventually several output classes, 
%it could be interesting to get an explanation of the holding relationships among different classification outputs. 
%\sm{For example, the user might be interested in discovering}  co-occurrences of certain input concept activations, like $soccer\_ball \wedge foot$ for a set of football images.

\sm{Independently on what has been described so far, the user might decide to automatically discover regularities that are about single examples, groups of data points, an entire class, or, more generally, the whole dataset, moving from \textit{local} to \textit{global} explanations.} %On the other hand, the user may also look for unbiased global explanations, like $zero\oplus one\oplus\ldots\oplus nine$, in a digit classification task. 
%In both the cases, learning is driven by unsupervised criteria.
%Each output concept activation of the LEN module can be tough as a cluster membership score. Thus, another view of \textsc{untargeted explanations} can be directly related to the notion of \textit{interpretable clustering}, where LEN can provide explanation of each cluster, as shown in Fig.~\ref{fig:concept_relations} for the case of MNIST digits.
%As another example, consider the case of gene expression analysis, where neural networks are usually employed to group similar patients according to their genes activations. LENs can be used not only to perform such grouping (E2E), but also understand why such groups have been formed and in particular which are the most relevant gene activations in each group. }


%\sm{In the following we provide further insights for \textsc{targeted} and \textsc{untargeted explanations}.}

%For this reason, we distinguish between the case in which LENs are trained in a supervised manner or with unsupervised criteria.

%A supervised task consists in learning and explaining a target \textit{class} with respect to a set of lower-level attributes, e.g. explanation of the class \textit{person} with respect to the attributes \textit{head, hands, body}. In this scenario LENs generate \textit{Supervised Explanations}.
%Alternatively, an unsupervised task consists in explaining hidden relations among \textit{concepts}, e.g. the classification outputs of another classifier or categorical attributes. In this scenario LENs yield \textit{Unsupervised Explanations}.
% Further, the explanation could have a global, local or even example-level validity. For instance, we may be interested in explaining a certain decision for a specific input, but also in universally valid regularities or simply most frequent co-occurrences among classes.
%In the following, we briefly discuss these two logical explanation styles %that are currently supported by the LENs framework
%which we respectively referred as \textit{Supervised Explanations} and \textit{Unsupervised Explanations}.
%In order to train a LEN to produce these %one or more of the following explanation styles, we can make use of ad hoc learning criteria, as successively discussed in Sec.\ref{sec:learncrit}


% \paragraph{Class-driven explanations}
%\textsc{Targeted explanations. }
% (local or global); \fg{richiederebbe spiegare, che mentre la LEN è vera esattamente dove la classe che spiega, la formula logica è soddisfatta dovunque.}
%Targeted explanations aim at providing a valid explanation for all the samples of a specific class. 
%This may be achieved by training a LEN to provide \textit{interpretable classification} or to \textit{explain a black-box model}.
%represent different kinds of causalities for a selected class with respect to the other ones, or a set of lower-level concepts. 
%Whenever the LEN belongs to a computational pipeline in which it is expected to both solve the classification problem and provide explanations (E2E when no black-box is considered, CB, Cascading), then it becomes a white-box classifier. 
%\sm{Learning of the LEN module is simply driven by a supervised objective function, in which $f$ is forced to be as close as possible to the corresponding $\bar{Y}$ on the available data. Whenever the LEN belongs to a computational pipeline in which it is expected to both solve the classification problem and provide explanations (E2E when no black-box is considered, CB, Cascading), then it becomes a white-box classifier. The examples of Fig.~\ref{fig:E2EExplainer} (left), Fig.~\ref{fig:CascadeExplainer}, Fig.~\ref{fig:CMBExplainer} are all about targeted explanations. In the E2E case when $g$ is present or, more generally, whenever LENs act in parallel to a black-box classifier with the only goal of providing explanations, then LENs are forced to yield outputs that are as close as possible to the black-box, so $f$ is forced to be close to $g$. This is what is shown in  Fig.~\ref{fig:E2EExplainer} (right)., and that we refer to as \textit{explaining a black-box}}

%One possibility is to use a LEN to directly accomplish a classification task. Indeed, it can provide an interpretable classification by training a LEN $f$ to satisfy $f_i\simeq Y_i$ for some $i\in\{1,\ldots,q\}$, i.e. to have $f_i(c)$ as close as possible to $Y_i(c)$ for any $c\in C$, where $Y_i(c)$ denotes the label of the $i$-th class on the input $c$, that the LEN is meant to both learn and explain. This solution is preferred when it is of fundamental importance to have a white-box classifier, while we can accept some drawbacks in terms of classification performances.
%However, we may also train a LEN $f$ to explain a black-box model $g$. Therefore, to satisfy $f_i\simeq g_i$ for some $i\in\{1,\ldots,d\}$, i.e. to have $f_i(c)$ as close as possible to $g_i(c)$ for any $c\in C$. This other solution is instead useful in those context where the classification performances play a key role and we may accept approximate explanations of the decision taken. 
%It is worth noticing that when explaining a black-box model $g$, a LEN may also take into account the classifier predictions on unlabeled data, e.g. in a semi-supervised learning setting. This allows the LEN to produce explanations covering a larger set of data, but also possibly inaccurate. 
%On the other hand, in the interpretable classification case the LEN learns explanations directly from (limited to) the labeled data. 
% \begin{itemize}
%     \item 
%     \textit{IF-Rules. } This kind of explanation provides a superset of a specific class assignment. For instance, an upper bound containing the class $flies$ can be defined according to the explanation "$flies\rightarrow bird\vee airplane$".
%     \item 
%     \textit{Only IF-Rules. } In this case an explanation is required to provide a subset of a specific class assignment. A lower bound contained in the class $flies$ may be obtained with the explanation "$has\_wings \ \wedge \ has\_engine\rightarrow flies$".
%     \item 
%     \textit{IFF-Rules. } An explanation  can completely characterize a certain class. For instance, the class $airplane$ can be defined according to the explanation "$airplane \leftrightarrow has\_wings\wedge has\_engine$".
% \end{itemize}
% We note that only with IFF-Rules explanations a LEN can be used for interpretable classification. Indeed, not any bird or plane can fly, so as a seagull can fly without having an engine. Hence, IF and Only IF-Rules are not suitable to correctly predict a specific class behaviour.
\iffalse
\begin{figure}[t]
    \centering
    \includegraphics[width=.48\textwidth]{figs/E2E.pdf} \quad %\\ \bigskip
    \includegraphics[width=.48\textwidth]{figs/e2e_explaining.pdf}
    \caption{LENs Supervised Explanations: interpretable classification, where the LEN directly provides the final classification (left), or explaining a black-box model $g$ (right).
    % Classification style: Explaining an existing classifier. Differently from the previous examples, here a LEN is used to explain the predictions made by an existing classifier $g(x)$ on the MIMIC classification task.} 
    }
    \label{fig:explainablevsexplanation}
\end{figure}
\fi

% \paragraph{Relations among concepts}
%\textsc{\sm{Untargeted} explanations. }
%  (local or global): MI, Conversion to CNF
%A user may be interested in discovering relations among different \sm{input} concepts without posing any preferences on any specific class. %For instance, by analyzing the output of a multi-label classifier $C=g_1(X)$ in a CB pipeline, %with eventually several output classes, 
%it could be interesting to get an explanation of the holding relationships among different classification outputs. 
%\sm{For example, the user might be interested in discovering}  co-occurrences of certain input concept activations, like $soccer\_ball \wedge foot$ for a set of football images.
%\sm{Differently from the case of \textsc{targeted explanations}, the user might decide to automatically discover regularities that are not about the whole dataset, but that may hold only for a portion of the available data. On the other hand, the user may also look for unbiased global explanations, like $zero\oplus one\oplus\ldots\oplus nine$, in a digit classification task. In both the cases, learning is driven by unsupervised criteria.
%Each output concept activation of the LEN module can be tough as a cluster membership score. Thus, another view of \textsc{untargeted explanations} can be directly related to the notion of \textit{interpretable clustering}, where LEN can provide explanation of each cluster, as shown in Fig.~\ref{fig:concept_relations} for the case of MNIST digits.
%As another example, consider the case of gene expression analysis, where neural networks are usually employed to group similar patients according to their genes activations. LENs can be used not only to perform such grouping (E2E), but also understand why such groups have been formed and in particular which are the most relevant gene activations in each group. }

\iffalse
\begin{figure}[t]
    \centering
    \includegraphics[width=0.58\textwidth]{figs/concept_relations.pdf}
    \caption{\sm{Automatic explanations. MNIST digits are classified as belonging to one of the 10 classes and whether they are even of odd by a black-box $g$.  %in a Concept-bottleneck pipeline 
     A LEN groups these predictions in an unsupervised manner, and analyzes the relations within each cluster.} Supervision labels are not provided for the LEN output. {\color{red}[Remove $g(X)$ and $f(g(X))$. FOL Explanation of Cluster 2 (not 1).]}}
    \label{fig:concept_relations}
\end{figure}
\fi

% \paragraph{Explanation Ranges}
% \textsc{Explanation Ranges. }
% As already mentioned, the explanations may hold on different input sub-portions. In terms of FOL formulas, this means that the extracted rules will be satisfied on different subsets of the concept space. For instance, we may consider example-level explanations, i.e. explanations focusing on individual class assignments. Example-level explanations can be aggregated into clusters up to overall class-level explanations. However, we may also be interested in frequent co-occurrencies or global principles among different classes.
%\fg{aggiungere qualche esempio?}



\section{Methods}
% \section{Formulas, Criteria and Pruning}
\label{sec:methods}
\sm{This section presents the fundamental methods that are used to implement the ideas of LENs. We start with the formal definition of the learning objectives (Section~\ref{sec:learncrit}), followed by the procedure that is used to extract FOL rules out of LENs for an individual observation  or in an aggregated manner (Section~\ref{sec:logic_rule_extr}). Finally, we discuss how to constraint LENs to avoid developing complex logic formulas by means of precise parsimony criteria (Section~\ref{sec:parsimony}).}


%This section presents the fundamental methods that are exploited to extract and ensure the style of a certain logic-based explanation for LENs (see Fig. \ref{fig:scheme2}).
%First we illustrate how different loss functions can be optimized to achieve customizable classification and explanation styles. Then, we discuss how first-order logic rules can be extracted from LENs for an individual observation and how explanations can be aggregated to be representative of a cluster of samples. Finally, we provide an overview of some parsimony criteria which can be used to avoid overly complex logic formulas and, in turn, useless explanations.

\begin{figure}[ht]
    \centering
    % \includegraphics[width=0.7\textwidth]{figs/scheme2.png}
    \includegraphics[width=0.85\textwidth]{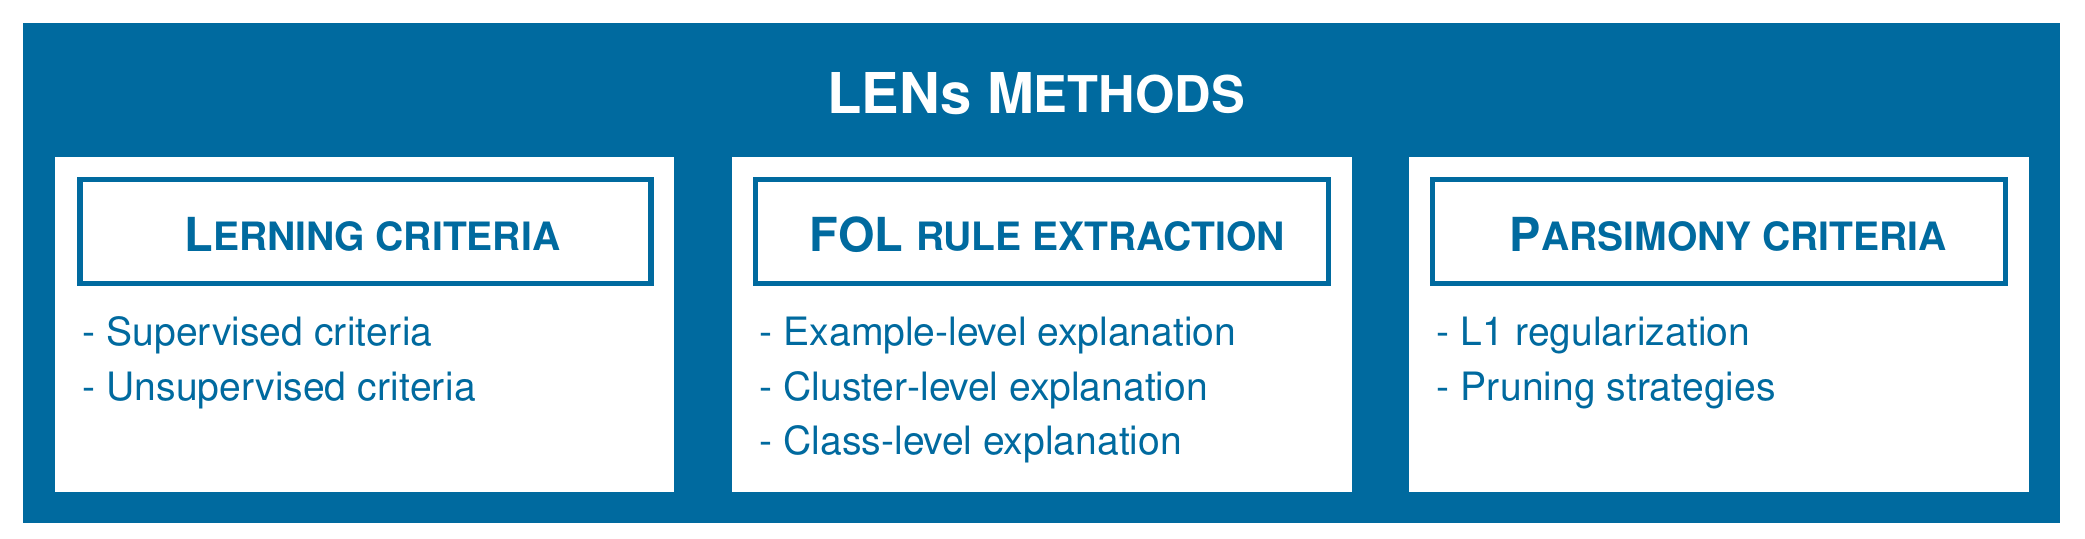}
    % \input{tikz/methods}
    \caption{\sm{Inside the LEN block (Section~\ref{sec:methods}). We distinguish among three categories of methods that implement the principles behind LENs:} learning criteria (Section~\ref{sec:learncrit}), FOL rule extraction (Section~\ref{sec:logic_rule_extr}), and parsimony criteria (Section~\ref{sec:parsimony}). {\color{red}[Swap cluster-level and class-level explanations. Rename example-level explanations with 'Example-level (local)'. Rename 'Class-level explanations' with 'Class-level (global). Do the same for 'cluster-level expl.']}}
    \label{fig:scheme2}
\end{figure}




\subsection{Learning Criteria}
\label{sec:learncrit}
%Cross Entropy in genere; Che può essere binary se è single o multilabel, altrimenti Softamx Cross Entropy
\sm{Following the distinction among the user preferences introduced in }Section~\ref{sec:explanation_styles}, here we focus on the loss functions that are optimized to train a LEN to \sm{develop the capability of providing explanations accordingly to such preferences}, that are the outcome of our previous experiences in \cite{ciravegna2020human,ciravegna2020human}.
\sm{For simplicity, here we will not distinguish the different computational pipelines, thus referring to a single generic LEN block with $q$ output units in all the case of \textsc{interpretable classification}, \textsc{explaining a black-box}, and \textsc{interpretable clustering}. Given an input sample, for each of the $r$ output concepts LENs yield a FOL rule $\varphi_i$, $i=1,\ldots,r$. We will use the notion of \textit{support of $\bar{f}_i$}  to indicate the subset of data samples on which the $i$-th output concept holds true, and \textit{support or rule $\varphi_i$} to indicate the subset of data samples for which the FOL rule $\varphi_i$ holds true.} %We will use the notation $\bar{Y}(c) \in \bar{Y}$ to indicate the function that returns the binary label vector associated to a generic input $c \in C$. With an abuse of notation, we will use $C$ also to indicate the set of available training inputs in the concept space. Moreover, $f_i$ is the function that returns the $i$-th output of the LEN, $i=1,\ldots,r$, and $\bar{Y}_i(c)$ is the associated $i$-th binary label.

% \paragraph{Class-driven Criteria.} 
\textsc{Interpretable classification. } 
%In the case of \emph{Supervised Explanations}, we aim at providing explanations of certain classes. In this sense, we want our model $f$ to be active whenever the class we aim to explain is also active.
% (i.e. $f_i(c) = Y_i(c) = 1$)
% We do not distinguish here whether the LEN is performing an \textit{interpretable classification} ($f_i\simeq Y_i$) or it is \textit{explaining an existing classifier} ($f_i \simeq g_i$), since for what concerns the optimization function it does not make any difference.
%Let us assume the interpretable classification case. The case of explaining a black-box model $g$ can be obtained by replacing $Y_i(c)$ with $g_i(c)$ in the loss unctions. The only difference in the two cases is that while $Y_i(c) \in \{0, 1\}$ is a discrete membership function, $g_i(c) \in [0,1]$ provides the probability of class assignment.
%Further, for sake of simplicity, in what follows we will assume $f: C=X\rightarrow E=Y$.
\sm{Training a LEN by supervised learning is what is needed in order to create the conditions to extract explanations over precise classes. There are three different specificity levels of the explanations that can be enforced, focusing on IF, Only IF or IFF rules, }
\begin{eqnarray*}
\text{IF}: && \bar{f}_i \rightarrow \varphi_i \\
\text{Only IF}: && \varphi_i \rightarrow  \bar{f}_i \\
\text{IFF}: && \bar{f}_i \leftrightarrow \varphi_i
\end{eqnarray*}
where $i=1,\ldots,r$.
\sm{IF rules mean that, in the extreme case, for each example of class $i$ we want the $i$-th output of the LEN to score one (and not necessarily vice-versa). In other words, the support of $\bar{f}_i$ has to be included in the support of the rule.}
%and each of them provide a superset of a specific class assignment and therefore requires the support of the antecedent to be included in the support of the consequent (i.e. $\{c\in C: \bar{Y}_i(c)=1\}\subseteq C_i$).
\sm{This behavior} can be achieved by minimizing a hinge loss,
\begin{equation}
L_{\rightarrow}(\bar{y}_i,f_i,\mathcal{C}) = \sum_{c\in \mathcal{C}} \max\{0, \bar{y}_i(c) - f_i(c)\}\qquad  i \in [1,  r].\label{eq:IF}
\end{equation}
 Following a symmetric approach, in Only IF rules it may be the case of a class to be explained in terms of some lower-level concepts. \sm{This principle is easily enforced} by switching the two terms of the loss function in Eq. \ref{eq:IF},
\begin{equation}
L_{\leftarrow}(\bar{y}_i,f_i,\mathcal{C}) = \sum_{c\in \mathcal{C}} \max\{0, f_i(c) - \bar{y}_i(c)\}\qquad  i \in [1,  r].\label{eq:IF2}
\end{equation}
\sm{Both in IF and Only IF rule, in order to make the learning problem well posed, further conditions on $f$ must be included, to define its behaviour in the space areas not covered by the data and to avoid trivial solutions with constant $f$.}
At last, LEN can learn double implication rules (IFF) in which an explanation can completely characterize a certain class. %These rules require the support of the LEN and the support of the class to be strictly equal.
%For this reason,
\sm{Any} function penalizing points for which $f_i(c)\not=y_i(c)$ may be employed in this scenario, such as the Mean Square Error loss,
\begin{equation}
L_{\leftrightarrow}(\bar{y}_i,f_i,\mathcal{C}) = \sum_{c\in \mathcal{C}} |f_i(c) - \bar{y}_i(c)|\sm{^2} \qquad  i \in [1,  r], \label{eq:IFF}
\end{equation}
or the classic Cross-Entropy loss.
%IFF loss function is preferred when a LEN performs E2E \textit{interpretable classification}, since we want the output of \sm{$f$} to be as close as possible to \sm{$\bar{Y}$} in order to maximize the classification accuracy. 
% In this latter case if we want the same LEN to explain different, mutually exclusive classes, a Softmax activation function can be also employed.  


\textsc{Explaining a black-box. } In this case, the output of the LEN is forced to mimic the one of the black-box $g$. A coherence loss can be exploited to reach this goal,
\begin{equation}
L_{g}(g_i,f_i,\mathcal{C}) = \sum_{c\in \mathcal{C}} |f_i(c) - g_i(c)|\sm{^2} \qquad  i \in [1,  r]. \label{eq:coher}
\end{equation}

%the explanations provided by LENs are first-order logic formulas, and this newly devised pieces of knowledge can be reused and enforced on the output of the classifier $g$. This is commonly considered in the generic \emph{learning from constraints} framework \cite{gnecco2015foundations}, and it may be of particular interest, especially for semi-supervised settings. A similar strategy has already been considered e.g. in \cite{ciravegna2020constraint}, where a set of FOL formulas have been, at first extracted from data, and then converted into continuous loss functions to be injected in the learning objective.
%At last, the extracted formulas can also be used to check the behaviour of the classifier on test data, e.g. to detect adversarial samples as done in \cite{melacci2020domain}.

\textsc{Interpretable clustering. }
% \paragraph{Mutual Information Criterion}
% \paragraph{Relations among Concepts.}
\sm{Generic explanations can be achieved by means of fully unsupervised  principles from Information Theory.} As a matter of fact, the maximization of the Mutual Information (MI) index between the input concept space $C$ and the \sm{output concept space} $E$ allows the LEN to
be trained in a fully unsupervised way \cite{ciravegna2020constraint}. More specifically, a max-MI criterion (see \cite{melacci2012unsupervised} for further details) \sm{leads to the development of a LEN that has the tendency of producing 1-hot activation scores,} such that $\forall c \in \mathcal{C}$ only one $f_i(c) = 1$, while the others are close to zero. \sm{In a sense, it enforces the LEN to cluster the data in a way that each input sample belongs to a single cluster.}
In order to define the MI index, \sm{we have to model the probability distribution $P_{i|c}(f)$, that is the probability of $f_i$ to be active (close to 1) on sample $c$ -- we implemented it using the softmax operator on the LEN output.} %Following the classic notation of discrete MI, 
%$E$ is a discrete random variable associated to the output of the LEN functions while $C$ is the variable related to the data in the concept space.
The penalty term to minimize \sm{to train the LEN} is minus the MI index,
\begin{equation}
    L_{MI}(f,\mathcal{C}) = - H_{E}(f,\mathcal{C}) + H_{E|C}(f,\mathcal{C}) \ ,
	\label{eq:MI}
\end{equation}
where $ H_{E}$ and $ H_{E|C} $ denote  the entropy and the conditional entropy functions associated to the aforementioned probability distribution, respectively, and measured over the whole $C$, as in  \cite{ciravegna2020constraint}. 
%An outcome of the maximization of the MI index is that the supports of the explaining functions will tend to partition the input space $X$, i.e., $X=\bigcup_{j=1}^mX_j$ and $X_j\cap X_k=\emptyset$, for $j\neq k$ (see \cite{melacci2012unsupervised,betti2019cognitive} for further details).

\sm{Of course, in all the computational pipelines} in which a classifier $g$ is also employed,
%In the particular case of a LEN providing explanations for an existing classifier $g$, 
the available supervision is enforced on $g$ as well, e.g., by means of the Cross-Entropy loss. As a side note, we remark that what we are describing in a fully supervised setting can be trivially extended to the semi-supervised one, as we already investigated in \cite{ciravegna2020constraint,ciravegna2020human}. 




\subsection{FOL Rule Extraction}
\label{sec:logic_rule_extr}
\sm{Once a LEN has been trained, it can associate one or more explanations for each output concept. We indicate with $\varphi_{i,\cdot}$ the explanation of concept $i$, where the second subscript can index either a single data sample $c$, $\varphi_{i,c}$, or a group $S$ of data samples, $\varphi_{i,S}$. As it will become clear shortly, extracting FOL rules out of a trained LEN can be done by inspecting its inputs/outputs accordingly to a Boolean interpretation of them. Whenever this is independently done for each single input sample, we get back \textsc{example-level explanations}, that we also refer to as \textit{local explanations}. Differently, whenever the explanations covers an entire category of examples, we talk about \textit{global explanations}, distinguishing between \textsc{class-level explanations} and \textsc{cluster-level explanations}. {\color{red}[I still don't understand what kind of explanations we can provide]}}

 %As already mentioned, the explanations may hold on different input sub-portions. In terms of FOL formulas, this means that the extracted rules will be satisfied on different subsets of the concept space. For instance, we may consider example-level explanations, i.e. explanations focusing on individual class assignments. Example-level explanations can be aggregated into clusters up to overall class-level explanations. However, we may also be interested in frequent co-occurrences or global principles among different classes.
 

\sm{In detail,} any LEN $f=(f_1,\ldots,f_r)$ requires both its inputs and outputs to belong to the real-unit interval. This apparent limitation allows any $f_i$, for $i=1,\ldots,r$, to be easily converted into a Boolean function $\bar{f}_i$, e.g. by thresholding its I/O, e.g., with respect to $0.5$ value. Therefore, any Boolean function $\bar{f}_i$ is converted into a FOL formula $\varphi_i$ in Disjunctive Normal Form (DNF) \cite{mendelson2009introduction} by means of its truth-table, see Fig.~\ref{fig:tt2form}.
%Given $f: C \rightarrow E$, 
\sm{In order to support the following descriptions, }
we define the set $O_i = \{c\in C:\ \bar{f}_i(c)=1\}$ as the set of all the $[0,1]$-valued concept tuples that make true the $i$-th output concept/explanation, i.e., the \emph{support} of $\bar{f}_i$. %For instance, if we are interested in targeted explanations only, any $O_i$ will generally consist in the set of inputs that are classified as belonging to the $i$-th class by the LEN.
% \paragraph{Local Explanation}
% \paragraph{Example-Level Explanation}

%\sm{Each output concept $i$ is associated to one of more explanations $\varphi_i,\cdot$, depending on its granularity level. In what follows, we described the case }

\textsc{Example-level explanations. }
Given $c\in O_i$, the booleanization of its continuous features may provide a natural way to get a logical explanation at example-level $\varphi_{i,c}$ as a FOL formula. In particular, \sm{if we indicate with $c_j,\ j=1,\ldots,k$ the human understandable name of the $j$-th input concept}, for any $c\in O_i$, we can consider the following as the \emph{local explanation} of the $i$-th output $f_i$ on example $c$,
\begin{equation}
    \varphi_{i,c} = \tilde{c}_1\wedge\ldots\wedge\tilde{c}_k \qquad\mbox{where } \tilde{c}_j:= 
    \begin{cases}
        \bar{c}_j, & \mbox{if }c_j \geq 0.5\\
        \neg \bar{c}_j, &\mbox{if } c_j < 0.5\\
    \end{cases}\ ,    
    \mbox{ for $j=1,\ldots,k$.}
    \label{eq:locexp}
\end{equation}
\begin{figure}[t]
\centering
    \includegraphics[width=0.8\textwidth]{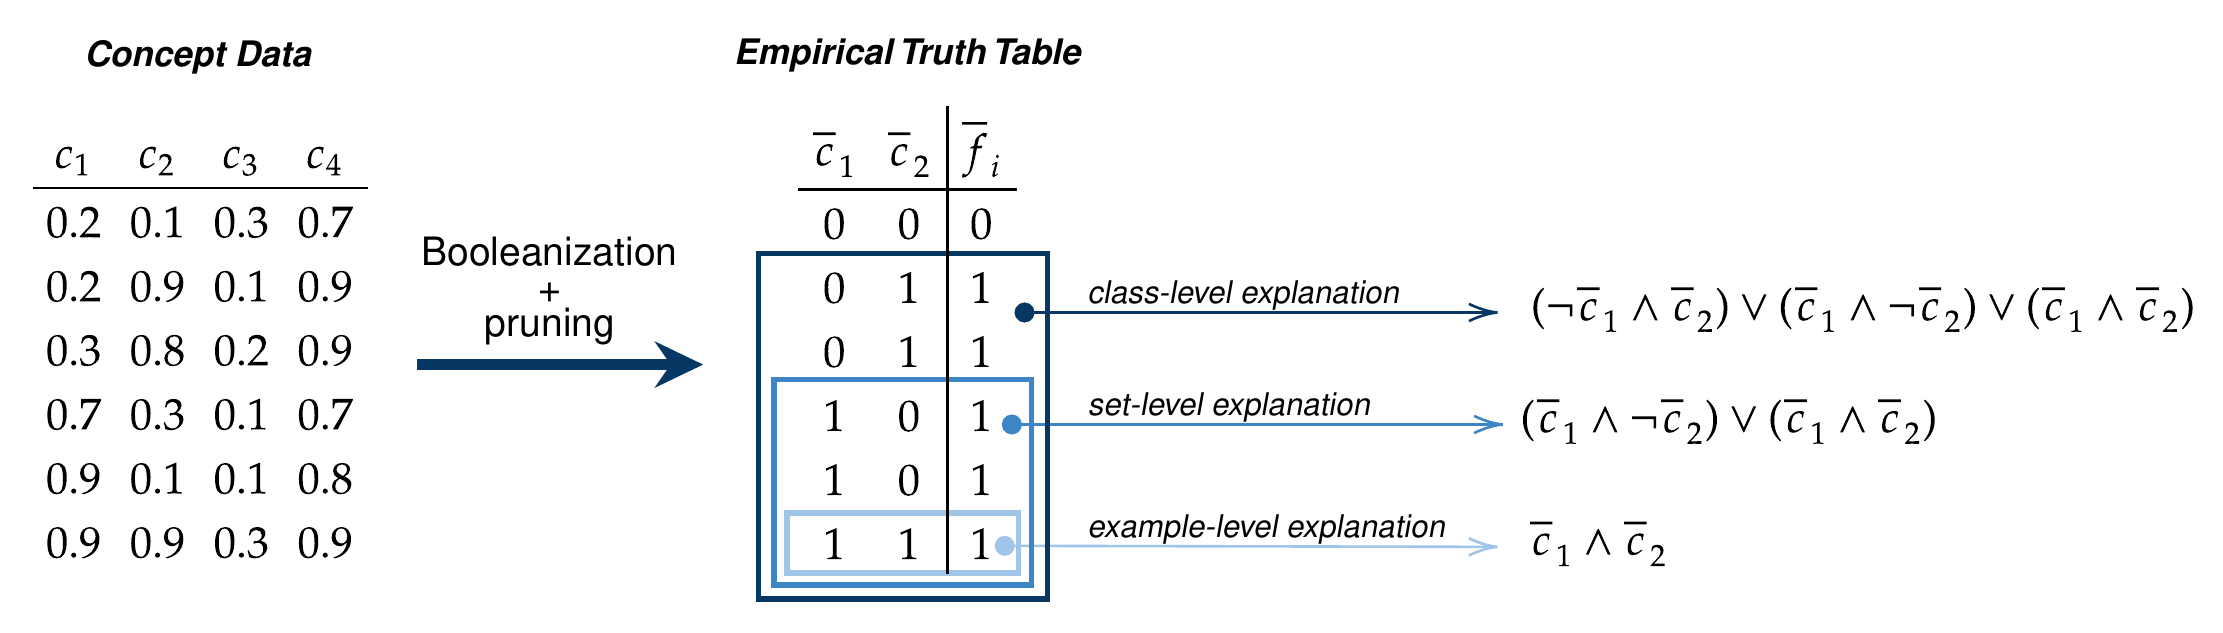}
    \caption{Extracting a logic formula from the truth-table of a binary boolean function $\bar{f}$.}
    \label{fig:tt2form}
\end{figure}
% \paragraph{Aggregated Explanation}
%\textsc{Aggregated explanation. }


%By considering Eq. \ref{eq:locexp} for any $c\in S$, and aggregating all the example-level explanations, we may easily provide a \emph{Cluster Explanation} $\varphi_{i,S}$ for a subset of samples $S \subseteq C_i$ as
\begin{equation}
    \varphi_{i,S} = \displaystyle\bigvee_{c \in S}\varphi_{i,c} = \displaystyle\bigvee_{c \in S}\tilde{c}_1\wedge\ldots\wedge\tilde{c}_k
\label{eq:agg_exp}
\end{equation}
%Any formula $\varphi_{i,S}$ can be thought of as a $\{0,1\}$-valued mapping defined on $C$, that is equal to 1 exactly on a cluster $S \subseteq C_i\subseteq C$. We may also get an explicit explanation relating $\varphi_{i,S}$ and the $i$-th output $f_i$ by the FOL formula:
%\[
%\forall c\in S:\ \varphi_{i,S}(c)\rightarrow \bar{f}_i(c)
%\]
% \paragraph{Global Explanation}
% \paragraph{Class-Level Explanation}

\textsc{Class-level explanation. }
We can aggregate local explanations associated to data belonging to a set $S \subseteq O_i$, yielding $\varphi_{i,S}$,
By considering Eq. \ref{eq:agg_exp} with $S=O_i$, i.e., aggregating all the example-level \sm{explanations of class $i$}, we get an overall explanation $\varphi_i$ for the \sm{LEN} output $f_i$.
\begin{equation}
    \varphi_i = \displaystyle\bigvee_{c \in C_i}\varphi_{i,c} = \displaystyle\bigvee_{c \in C_i}\tilde{c}_1\wedge\ldots\wedge\tilde{c}_k.
\label{eq:glo_exp}
\end{equation}
Also in this case, any formula $\varphi_i$ can be thought of as a $\{0,1\}$-valued mapping, that is equal to 1 exactly on $O_i\subseteq C$. We may get as \emph{global explanation} a FOL formula relating $\varphi_i$ and the $i$-th output $f_i$ by means of
\[
\forall c\in C:\ \bar{f}_i(c)\leftrightarrow\varphi_i(c).
\]
% RECURSION\_STEP
% \paragraph{Compounding Explanations}
%\textsc{Compounding explanations. }

Both example-level, aggregated and class-level explanations can be recursively applied in case a cascading LENs or a single LEN with multiple $[0,1]$-valued layers are considered. For instance, given a cascading LEN as \sm{the one of Fig.~\ref{fig:CascadeExplainer}}, we may get both local and global explanation of the concepts in \sm{$E_1 = C_2$ with respect to the ones in $C_1$, so as the concepts in $E_2$ with respect to the ones in $C_2$ and, in turn, in $C_1$}. The modularity of FOL formulas allows the composition of concepts at different levels that may express arbitrary complex relationships among them.

% \paragraph{Aggregation of Cluster-Level Explanations}
\textsc{Cluster-level explanations. }
In the case in which the maximum MI criterion (Eq. \ref{eq:MI}) is used to drive the learning problem, each $\varphi_i$ will generally hold on a sub-portion of the concept space $O_i\subseteq C$. {\color{red}[This is also true for the supervised case, what is the difference?]} However, we may get a FOL providing a global explanation by means of the disjunction
$\varphi = \varphi_1\vee\ldots\vee\varphi_r$, indeed $C_1\cup\ldots\cup C_r=C$. Since the formula $\varphi$ can be very complex, if we are interested in simpler global explanations we may  convert $\varphi$ into an equivalent $\varphi'$ in \emph{Conjunctive Normal Form} (CNF). In particular, there exist $r'$ and clauses $\varphi'_1,\ldots,\varphi'_{r'}$ such that: 
\[
\varphi=\bigvee_{i=1}^r\varphi_i \equiv \bigwedge_{i=1}^{r'}\varphi'_i=\varphi'.
\]
As a result, we get the following global explanations for $i=1,\ldots,r':
\forall c\in C:\ \varphi'_i(c)$.
Unfortunately, converting a boolean formula into CNF can lead to an exponential explosion of the formula; in the following, we will see how to address this problem. 
% However, after having converted each $\varphi_i$ in CNF, the conversion can be computed in polynomial time with respect to the number of minterms in each $\varphi_i$ \cite{russell2016artificial}.

\begin{example}
\label{ex:xor}
Let's consider the boolean $xor$ function, defined by $xor(0,0)=xor(1,1)=0$, $xor(1,0)=xor(0,1)=1$. 
Let $f$ be a LEN that has been trained to approximate the $xor$ function in the input space $C=[0,1]^2$. Then, if we consider e.g. the inputs $c^1=(0.2,0.7)$, $c^2=(0.6, 0.3)$, we get $\bar{c}^1=(0,1)$, $\bar{c}^2=(1,0)$, and therefore $\bar{f}_1(c^1)=\bar{f}_1(c^2)=1$. These examples yield respectively the local explanations $\varphi_{1,c^1}=\neg \bar{c}_1\wedge \bar{c}_2$ and $\varphi_{1,c^2}=\bar{c}_1\wedge\neg \bar{c}_2$, and the class-level explanation for $f_1$ is given by $\varphi_i=(\neg \bar{c}_1\wedge \bar{c}_2)\vee(\bar{c}_1\wedge\neg \bar{c}_2)$. In the same way, we may get the class-level explanation for the output $f_0$. In the end, the following formulas represent the supervised explanations of the false and true classes, respectively:
\[
\forall c:\ \bar{f}_0(c)\leftrightarrow (\neg \bar{c}_1\wedge\neg \bar{c}_2)\vee(\bar{c}_1\wedge \bar{c}_2)\qquad\mbox{and}\qquad
\forall c:\ \bar{f}_1(c)\leftrightarrow (\neg \bar{c}_1\wedge \bar{c}_2)\vee(\bar{c}_1\wedge\neg \bar{c}_2)
\]
The two global explanations correctly match the truth table of the boolean $xor$ function.

\begin{figure}
    \centering
    \includegraphics[width=0.7\textwidth]{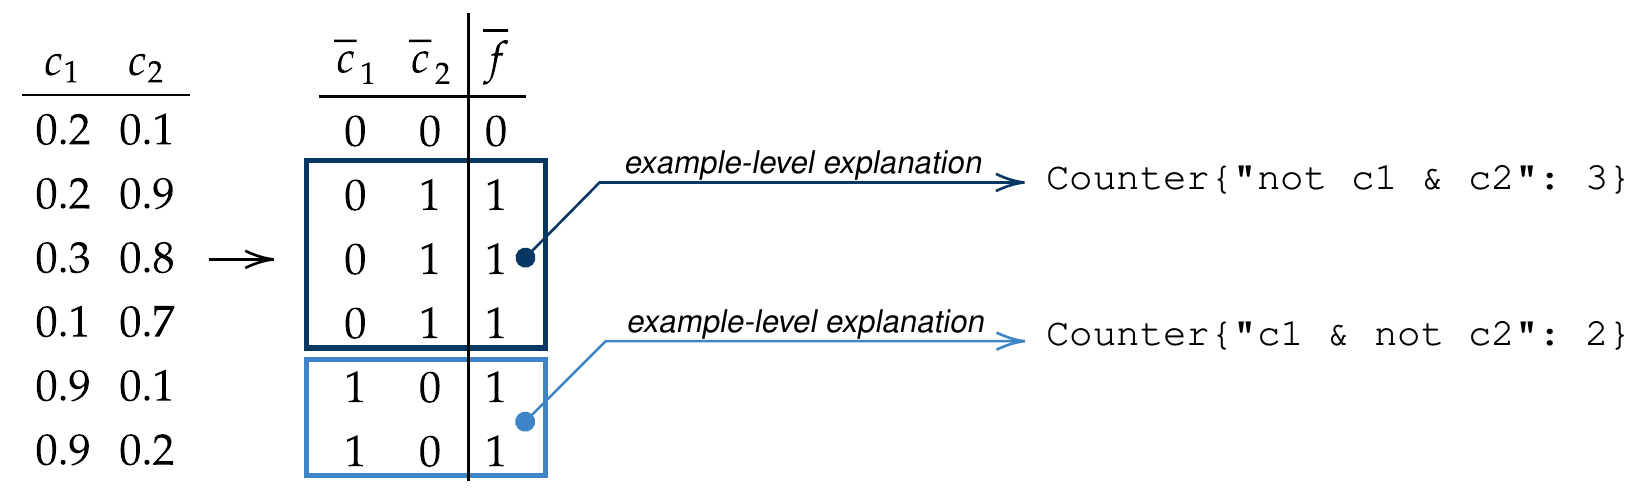}
    \caption{Aggregation of concept tuples with the same booleanization yields a common example-level explanation, and do not complicate the class-level explanation. For any example-level explanation, we may count how many samples it explains. Infrequent explanations may then be pruned to avoid explanation overfitting.}
    \label{fig:tt2form_freq}
\end{figure}

% If we then consider that $f$ is composed of two hidden and one output neurons, we may want to explain the behaviour of each node. In particular, we may get that the first hidden neuron is represented by $ \tilde{h}_1^1  \leftrightarrow \neg \textit{c}_1\wedge \textit{c}_2$ 
% while the second $ \tilde{h}_2^1  \leftrightarrow \textit{c}_1\wedge \neg \textit{c}_2$. The output neurons $h^2 = f$ can be also represented in terms of the hidden neurons $f \leftrightarrow h_1^1 \vee h_2^1$ which in turns can be described again in terms of input concepts $f \leftrightarrow (\neg \textit{c}_1\wedge \textit{c}_2) \vee ( \textit{c}_1\wedge \neg\textit{c}_2)$.

\end{example}

% \paragraph{Remarks}
The method described so far illustrates how logic-based explanations can be formally aggregated to produce a range of explanations, from the characterization of individual observations to formulas explaining the model predictions for all the samples of a target class.
The formula for a whole class can be obtained by aggregating all the minterms corresponding to local explanations of all the observations having the same class label.
In theory, this procedure may lead to overly long formulas as each minterm may increase the complexity of the explanation. In practice, we observe that many observations share the same logic explanation, hence their aggregation does not change the complexity of the class-level formula (Fig. \ref{fig:tt2form_freq}). In general, class-level explanations can be provided by aggregating just the most common explanations extracted from samples with the same class label, avoiding a sort of "explanation overfitting" with the inclusion of noisy minterms which may correspond to outliers. To summing up, a possible limitation of this naive approach can be the readability of the logical rules, for instance in case (i) the number of input features (the length of any minterm) $d \gg 1$, (ii) the size of the support $|C_i|$ is very large (possibly getting too many different minterms for any $f_i$). For these reasons, possible approaches to maintain an easy-to-understand set of very concise logical rules are fundamental to provide an useful explanation, e.g. as decision support. More details on how to select the most meaningful explanation terms are provided in Sec. \ref{sec:parsimony}.


\subsection{Parsimony criteria} \label{sec:parsimony}
When humans compare a set of explanations outlining the same outcomes, they tend to have an implicit bias towards the simplest one \cite{aristotlePosterior,mackay2003information}. Over the years, researchers have proposed many approaches to integrate "\textit{the law of parsimony}" into learning machines.
Here we describe a few fundamental parsimony criteria which may help in developing and implementing a variety of Logically Explained Networks. A specific combination of the following methodologies may be adopted or ignored depending on end-user requirements on the explanations and on the classification performance.
% \subsubsection{Occam's razors}
% \paragraph{Occam's razors}
% \textsc{Occam's Razors. }
Bayesian priors \cite{wilson2020case} and weight regularization \cite{kukavcka2017regularization} are just some of the most famous techniques to put in practice the Occam's razor principles in the fields of statistics and machine learning.
Among such techniques, $L1$-regularization \cite{santosa1986linear} has been recently shown quite effective for neural networks providing logic-based explanations \cite{ciravegna2020human} as it encourages weight sparsity \cite{tibshirani1996regression}:
% \begin{equation}
    $\lambda ||W||_1$.
% \end{equation}
By shrinking the less important weights %'s values 
to zero, this regularization technique completely removes some weights %altogether in the limit, 
leading to sparse configurations. This allows to ignore the associated input features and, therefore, to provide simpler explanations. For this reason, all out-of-the-box LENs presented in the next section are trained using this parsimony criterion.

\subsubsection{Pruning strategies}
\label{sec:pruning}
The action of parsimony criteria, such as regularizers or human priors, influences the learning process %of learning machines 
towards specific local minima. Once the model has finally converged to the desired region of the optimization space, the effort can be speed up and finalized by pruning the neural network \cite{lecun1989optimal,hassibi1993second}. The pruning strategy has a profound impact both on the quality of the explanations but also on the learning capacity model and, as a result, on the classification performance as well \cite{frankle2018lottery}. Here we present three effective pruning strategies specifically devised for LENs.

% \paragraph{Node-level pruning}
\textsc{Node-level pruning. }
A straightforward approach to pruning consists in defining the maximum \textit{fan-in} (number of non-pruned connections) for each neuron of a feed-forward neural network. We refer to this strategy as \textit{Node-level pruning}.
%A fan-in pruning strategy generates a feed-forward graph where each neuron has the same number of incoming non-pruned connections. 
At the end of the training process, the absolute value of the weight matrix $W_i$ is computed for each layer $i=1,\dots,L$. 
The node-level approach prunes one by one the weights with the smallest absolute value, such that each neuron in the network has a fixed number of incoming non-pruned weights $q \geq 2$. The parameter $q$ must be decided a priori and determines the learning capacity of the pruned model as well as the complexity of the logic formulas which can be extracted. To get reasonably simple explanations, the parameter $q$ may range between $2$ and $9$ \cite{miller1956magical,cowan2001magical,ma2014changing}). Recent work on explainer networks has shown how node-level pruning strategies may lead to fully explainable models  \cite{ciravegna2020constraint}. However, we will show in the experimental section that this pruning strategy strongly reduce the classification performances.

% \paragraph{Network-level pruning}
\textsc{Network-level pruning. }
In order to overcome the heavy reduction of the learning capacity of the node-level pruned models, we introduce here the \textit{Network-level pruning}. 
Indeed, the main aim of pruning is to only reduce the number of input terms involved in the final explanations. By directly limiting the number of input features considered by the network, we can achieve this result with a lighter impact on the overall model. 
Once the network has converged, the Frobenius norm of the first-layer weight matrix $W_1$ is computed: $w_1 = ||W_1||_2$. The vector $w_1$ is then re-scaled in the interval $[0,1]$:
\begin{equation}
    w_1' = \frac{w_1}{\max w_1}
\end{equation}
In this way, $w_1'$ gives a normalized score to rank input feature by importance. The \textit{Network-level strategy} consists in pruning all the input features where $w_1' < w_t$, where $w_t$ is a threshold set a priori (usually $w_t = 0.5$). Alternatively, %the $\mu$ approach may 
we can also retain the $q$ most important input features and prune the others for the entire first layer, as done in the \textit{Node-level pruning} for each single node. %The parameter $q$ is user-defined and may range between $2$ and $9$ to get sensibly compact explanations \cite{miller1956magical,cowan2001magical,ma2014changing}. 
This pruning strategy is far less stringent compared to the node-level pruning as it affects only the first layer and it does not prescribe a fixed fan-in for each neuron.

% \paragraph{ReLU pruning}
% \paragraph{Example-level Pruning}
\textsc{Example-level pruning. }
Example-level pruning is a particular strategy exploiting the well-studied local linearity property of neural networks whose activation functions in all hidden layers are Rectified Linear Units (ReLu Networks) \cite{hahnloser2000digital}. 
% \paragraph{Local Linearity}
For any input $x \in \mathbb{R}^d$, the initial Directed Acyclic Graph (DAG) ${\cal G}$ describing the structure of a ReLu Network, is reduced to ${\cal G}_{x}$,
which only keeps the units corresponding to active neurons and the corresponding arcs (firing path). 
Since all neurons operate in ``linear regime'' (affine functions), as stated in the following, 
the transformation $z: X \rightarrow Y$, which  is the composition of affine functions, corresponds to a single affine function $f^*(x) = W x + b$. 
\begin{theorem}
	Let $\{h_1,\ldots,h_L \}$ a collection of affine functions, where
% 	\[
		$h_{i}: X_{i} \mapsto Y_{i}: x \mapsto W_{i} x + b_{i}$
% 	\]
	and $\forall i=1,\ldots, L-1: \ \ X_{i+1} \subset Y_{i}$, then, 
% 	\[
		$z(x) = h_{L} \circ h_{L-1} \circ \dots \circ h_{2} \circ h_{1} x.$
% 	\]
	is affine and we have $f^*(x) = W x + b$, where
	\begin{equation}
	    W(L) = \prod_{\kappa=1}^{L} W_{\kappa}, \qquad 
		b(L) = \sum_{\kappa=0}^{L-1}  b_{L-\kappa} \prod_{h=0}^{\kappa} W_{L-h+1}  
	\end{equation}
	and $W_{L+1}:=I$.
	\label{theorem:affine}
\end{theorem}

Therefore, for a given input $x$ an affine function $f^*(x)$ can be devised. Notice that Theorem \ref{theorem:affine} only requires hidden layers node to be equipped with a ReLU activation function: nor the input nor the output nodes needs to employ it. %On the contrary, output nodes may be equipped with a sigmoid activation for binary or multi-label classification or a softmax activation function in case of multiclass.
Since the function $f^*(x)$ is affine, its interpretation is already much easier than considering the initial deep network $f(x) = h_{L} \circ h_{L-1} \circ \dots \circ h_{2} \circ h_{1} x$. Indeed, for each sample we can calculate the Frobenius norm of the corresponding weight matrix $w_L = ||W(L)||_2$. At last, similarly to what is done in the network-level pruning, we can retain the most important input features which satisfy $w'_L > w_t$, where again $w'_L = \frac{w_L}{\max w_L}$ and $w_t$ is set to 0.5. 


\section{Out-of-the-box LENs}\label{sec:outofthebox}


Crafting state-of-the-art fully interpretable models is not an easy task; rather, there is a trade-off between interpretability and performances.
The proposed framework is designed to provide the building-blocks to create a wide range of models having different interpretability-VS-accuracy
% interpretability-VS-explainability-VS-performance
trade-offs.
Here, we show how to combine the methods presented in the previous section to design three different out-of-the-box LENs (Fig. \ref{fig:out-of-the-box}): a) the $\psi$ network, as proposed in \cite{ciravegna2020constraint} which is a fully interpretable model with limited learning capacity and providing mediocre explanations; b) the $\mu$ network, a neural model providing high-quality explanations, great learning performances and modest interpretability;  c) the ReLU network, a black box model ensuring state-of-the-art learning performance and good explanations at the cost of very low interpretability. The characteristics of these three LENs are also resumed in Tab. \ref{tab:LENs}.


\begin{table}[ht]
\centering
\caption{Out-of-the-box LENs summary.}
\label{tab:LENs}
\resizebox{\textwidth}{!}{
\begin{tabular}{llllll}
\toprule
\textbf{LEN}                            & \textbf{Pruning} & \textbf{Activation}  & \textbf{Learning}  & \textbf{Explanation}   & \textbf{Interpretability}\\
\midrule

$\psi$ Network (Fig. \ref{fig:psi_net}) & Node-level        & Sigmoid                       & Low                           & Low                               & Very high     \\
$\mu$ Network (Fig. \ref{fig:mu_net})   & Network-level     & Any                           & High                          & Very high                         & High          \\
ReLU Network (Fig. \ref{fig:relu_net})  & Example-level     & ReLU                          & Very high                     & High                              & Low           \\

\bottomrule
\end{tabular}
}
\end{table}


\begin{figure}[ht]
    \centering
     
     \begin{subfigure}{1\textwidth}
         \centering
         \includegraphics[width=0.6\textwidth]{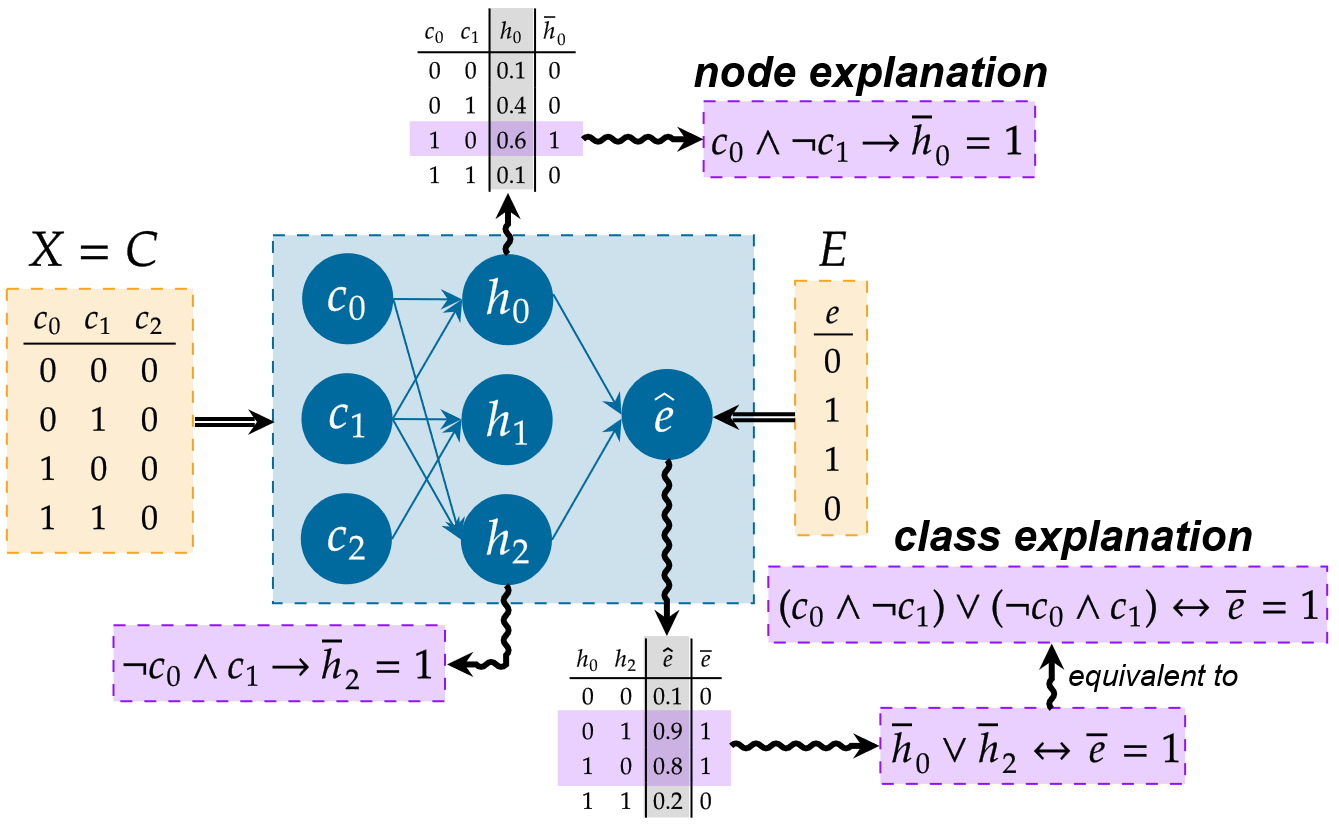}
         \caption{$\psi$ network (Subsection \ref{subsec:psi}).}
         \label{fig:psi_net}
     \end{subfigure}\\
     
     \begin{subfigure}{0.47\textwidth}
         \centering
         \includegraphics[width=1\textwidth]{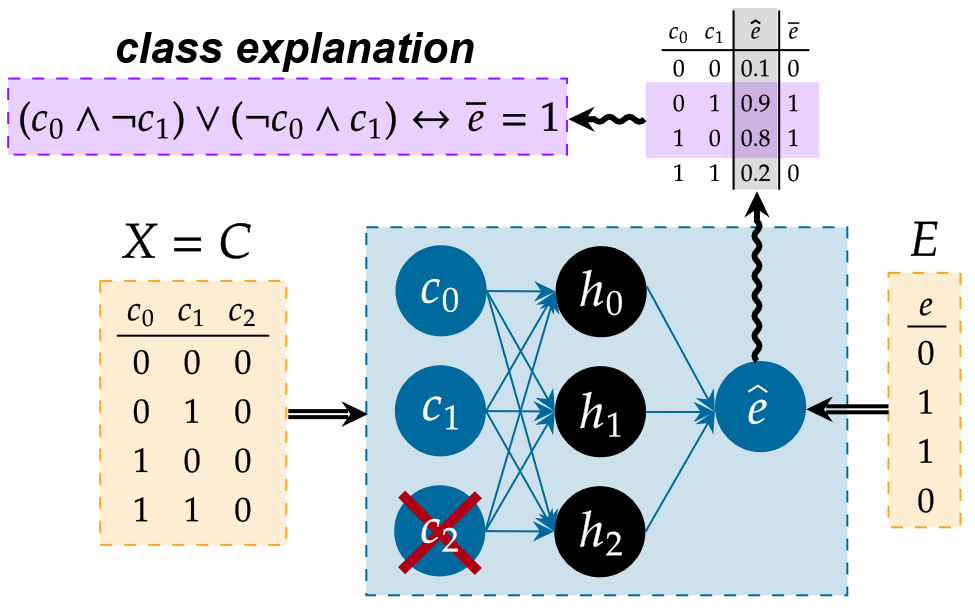}
         \caption{$\mu$ network (Subsection \ref{subsec:mu}).}
         \label{fig:mu_net}
     \end{subfigure}
     \qquad
     \begin{subfigure}{0.47\textwidth}
         \centering
         \includegraphics[width=1\textwidth]{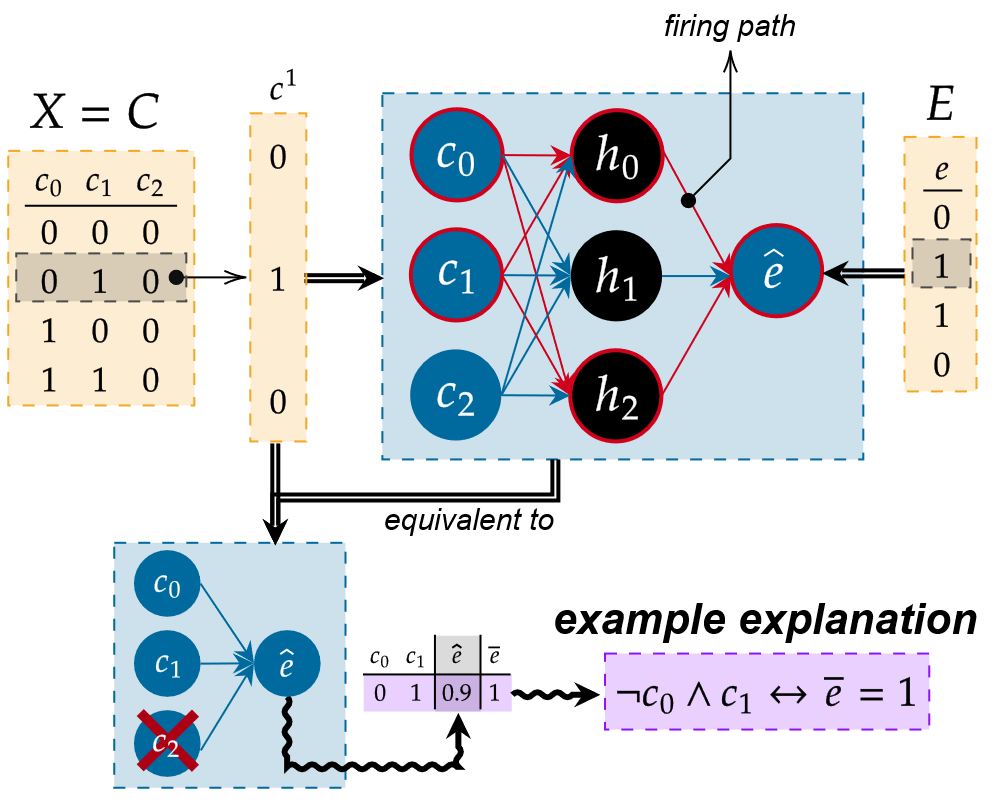}
         \caption{ReLU network (Subsection \ref{subsec:relu}).}
         \label{fig:relu_net}
     \end{subfigure}
     
    \caption{Out-of-the-box LENs. (a) $\psi$ networks 
    %(Subsection \ref{subsec:psi}) 
    only admit $[0,1]$-valued neurons with low fan-in, hence we can associate a boolean formula to each neuron by analysing its I/O truth-table. (b) $\mu$ networks 
    %(Subsection \ref{subsec:mu}) 
    do not have interpretable hidden neurons but the input concepts are drastically pruned which allows to provide simple network-level explanations. (c) ReLU networks 
    %(Subsection \ref{subsec:relu}) 
    supply explanations for each sample by means of the equivalent affine transformation. However, nor the nodes, nor the network can be logically interpreted.}
    \label{fig:out-of-the-box}
\end{figure}

\subsection{The $\psi$ network} \label{subsec:psi}
A $\psi$ network is a Logically Explained Network already proposed by \cite{ciravegna2020constraint,ciravegna2020human}. A $\psi$ network is based on three design principles: 
(i) all activation functions for all neurons (including hidden units) should be Sigmoid;
(ii) a strong L1-regularization is used in all layers to shrink the less important weight's values towards zero;
(iii) a Node-level pruning strategy, where each neuron of the network must have the same number of incoming non-pruned weights (suggested values are between 2 and 9). This number is directly proportional to the number of terms involved in the explanations. 
Also the number of hidden layers in the network needs to be set carefully, since the number of terms exponentially grows with the number of layers. 
% \begin{figure}
%     \centering
%     \includegraphics[scale=0.24]{figs/psi_nn.png}
%     \caption{Caption}
%     \label{fig:my_label}
% \end{figure}
The typical use case presented in the original work is a concept-bottleneck scenario. A black-box model $g$ (e.g. a convolutional neural network) is used to predict a set of categories $C$ from an unstructured data set $X$ (e.g. images). The authors used a $\psi$ network to explain the behaviour of a classifier $g$, i.e. $C \xrightarrow[]{f} E=g(X)$. The $\psi$ network is specifically designed to be a fully interpretable neural network, therefore, here we also show its performances as a classifier in different contexts. It can provide the whole set of logic-based explanations: example-level, aggregated, class-level, and it is the only LEN providing also compounding node by node explanations. As a matter of fact, thanks to the node-level pruning strategy, the $\psi$ network allows to interpret (and extract a corresponding logic formulas) from each node. 
Recalling Example \ref{ex:xor}, a $\psi$ network with two hidden nodes may learn the logic formula 
\begin{equation}
\forall c:\ \bar{f}_1(c)\leftrightarrow (\neg \bar{c}_1\wedge \bar{c}_2)\vee(\bar{c}_1\wedge\neg \bar{c}_2),
\label{eq:xor}
\end{equation}
with hidden nodes learning $h_1(c) \leftrightarrow (\neg \bar{c}_1\wedge \bar{c}_2)$, $h_2(c) \leftrightarrow ( \bar{c}_1\wedge \neg\bar{c}_2)$ and output node $f_1 \leftrightarrow h_1 \vee h_2$.
A $\psi$ network can be seen as a Cascading LEN where each layer corresponds to a new level of LEN. However, the network is always trained as a whole since no symbolic concept is provided at each level. Furthermore, also the explanations are always given in terms of input features for this reason. 
As reported in Fig. \ref{fig:psi_net}, this network provides the highest level of interpretability since the $\psi$ network provides for an explanation of the behaviour of each neuron. 
On the contrary, the strong regularization and the restrictive pruning strategy lead to poor classification accuracy making $\psi$ networks hard to train and not suitable for solving complex categorical learning problems. Besides, the provided explanations can be very expressive but they can be not outstanding as expected, due to the limited learning performance. 

\subsection{The $\mu$ network}  \label{subsec:mu}
A $\mu$ network is a LEN based on a standard multi-layer perceptron. A $\mu$ network is based on two design principles:
    (i) a strong L1-regularization is used only in the first layer of the network;
    (ii) a Network-level pruning strategy, which only prune the  neurons (features).
After the pruning step, the $\mu$ network can be fine-tuned to adjust to the new configuration. No assumption need to be made nor on the hidden layers nor on the activation functions. However, by applying a Network-level strategy, the same set of retained features is used for the whole network. On the one side, this allows to logically-interpret the network and, therefore, to provide explanations. On the other side, this may represent a severe limitations for multi-class classification since each class may rely on few features, but these may be very different between each class. Therefore, in the multi-class experiments of Sec. \ref{sec:experiments}, we train a set of light binary $\mu$ networks, one for each class. 

%This LEN can provide a wide range of logic-based explanations (i.e. local, cluster, and class-level).
%For each $\mu$ network, an explanation is provided in terms of the input concepts. 
Recalling Ex. \ref{ex:xor}, a $\mu$ network with variable number of hidden layers, may learn the logic formula in \ref{eq:xor}.
The Network-level strategy in this case should not prune any input features since both $c_1$ and $c_2$ are important for the final classification. In case instead also some redundant features are present, they are discard in favor of $c_1$ and $c_2$ as shown in Fig. \ref{fig:mu_net}. 
%As described in Sec. \ref{sec:logic_rule_extr} 
For some points the network will learn the aggregated explanations:
\begin{equation}
\forall c \in S_1: \neg c_1 \wedge c_2 \rightarrow f_1(c) \quad \text{and} \quad \forall c \in S_2: c_1 \wedge \neg c_2 \rightarrow f_1(c). 
\end{equation}
The two explanations can be then considered altogether to explain the class $C_1$: 
\begin{equation}
\forall c\in C:\ \bar{f}_1(c)\leftrightarrow\varphi_1(c) = \bigvee_{c \in C_i}\varphi_{i,c} =
 (\neg \bar{c}_1\wedge \bar{c}_2) \vee ( \bar{c}_1\wedge \neg\bar{c}_2).
 \label{eq:mu}
\end{equation}

Thanks to the permissive pruning strategy, the learning capacity of the network remains intact for the most part. As a consequence, $\mu$ networks are suitable for solving and explaining more complex categorical learning problems. The quality of the explanations provided by the $mu$ networks are among the higher between the proposed models. At last, a mild-level of interpretability is also guaranteed since it can be logically interpreted at a network-level. 

\subsection{The ReLU network}  \label{subsec:relu}
Another example of LEN which provides a different accuracy-vs-interpretability trade-off is the ReLU network. %is a special case of a $\mu$ network sharing most of its characteristics but with a few different properties. 
It is based on three design principles:
    (i) all activation functions for all \emph{hidden} neurons are rectified linear units;
    (ii) a mild L1-regularization in all layers of the network;
    (iii) an Example-level pruning strategy, i.e. a specialized pruning strategy for each sample.
The pruning employed in this LEN is an example-level pruning, which is available since it employs rectified linear units activation functions. %, i.e. a pruning strategy which is applied for each sample. 
This is not a limitations since it is one of the most widely used and efficient activation functions employed in deep learning \cite{glorot2011deep,ramachandran2017searching}.
On the contrary, this pruning strategy, does not cut the connections of the LEN $f$ as it is applied on the affine function $f^*$ directly to get a custom explanation for each observation. This means that the original capacity of the model is fully preserved, eventually leading to state-of-the-art classification performances. However, this type of pruning does not provide any insights of the model behaviour and may not always lead to optimum explanations.

Recalling again Example \ref{ex:xor}, a ReLu network with variable number of hidden layers, may learn the correct logic formula by aggregating local examples as it is done in \ref{eq:mu}. However, the local explanations of a certain point $c$ may not be as correct as the ones provided by the $\mu$ networks. Indeed, it can be demonstrated that the corresponding affine function $f*$, actually corresponds to the nearest decision boundary to the points. 
% On the other hand, an example-based pruning strategy may be provide more unstable explanations as the pruning may be negatively affected by the presence of outliers.
Therefore, the corresponding weights may miss some important features to explain $c$. A Relu network sometimes may explain the XOR problems with the wrong formula:
\begin{equation}
\forall c\in C:\ \bar{f}_1(c)\leftrightarrow\varphi_1(c) = \bigvee_{c \in C_i}\varphi_{i,c} =
 (\neg \bar{c}_1) \vee (\neg\bar{c}_2).
\end{equation}
Summing up, this LEN does provide the best performances in terms of classification accuracy thanks to the example-level pruning strategy. However, this comes at the cost of poor model interpretability and mild explanation capacity. 

% \begin{figure}
%     \centering
%     \includegraphics[scale=0.3]{figs/relu_nn.png}
%     \caption{Caption}
%     \label{fig:my_label}
% \end{figure}


\section{Benchmarking out-of-the-box LENs} \label{sec:experiments}
In this section, we quantitatively assess the quality of the explanations and the performance of Logically Explained Networks compared to state-of-the-art white-box models. Each task is uniquely defined by the tuple "pipeline / explanation style". The summary of each task is reported in Table \ref{tab:datasets}.
A brief description of each task, the corresponding dataset and all the related experimental details are exposed in Subsection \ref{sec:exp_details}. In Subsection \ref{sec:exp_metrics} six quantitative metrics are defined and used to compare LENs with state-of-the-art methods.

\begin{table}[ht]
\centering
\caption{Experiments.}
\label{tab:datasets}
\resizebox{\textwidth}{!}{
\begin{tabular}{llll}
\toprule
\textbf{Dataset} & \textbf{Description} & \textbf{Explanation Style} & \textbf{Pipeline}\\
\midrule

MIMIC-II (Fig. \ref{fig:E2EExplainer})                      & \small{Predict patient survival from clinical data}       & Interpretable classification  & E2E \\
MNIST E/O (Fig. \ref{fig:CMBExplainer})                         & \small{Predict parity from digit images}                  & Interpretable classification  & CB\\
CUB (Fig. \ref{fig:len})                                    & \small{Predict bird species from bird images}             & Interpretable classification  & CB\\
V-Dem (Fig. \ref{fig:CascadeExplainer})                     & \small{Predict electoral democracy from social indexes}   & Interpretable classification  & Cascading \\
MIMIC-II (EBB) (Fig. \ref{fig:explainablevsexplanation})    & \small{Predict patient survival from clinical data}       & Explaining black box       & E2E\\
MNIST E/O (IC) (Fig. \ref{fig:concept_relations})                    & \small{Cluster digit properties from digit images}        & Interpretable clustering      & CB\\
\bottomrule
\end{tabular}
}
\end{table}


% \subsection{Software tool and usability}
% \label{sec:tool}
In order to make the LENs framework accessible to the whole community, we released of a Python package\footnote{\url{https://pypi.org/project/deep-logic/}} with an extensive documentation on methods and out-of-the-box LENs. The Python code and the scripts used for the experiments, including parameter values and documentation, is freely available under Apache 2.0 Public License from a GitHub repository\footnote{\url{https://github.com/pietrobarbiero/deep-logic}}.

The Deep Logic library is designed to make out-of-the-box LENs accessible to researchers and neophytes by means of intuitive APIs requiring only a few lines of code to train and get explanations from a LEN (as shown in the code example \ref{code:example}).

\begin{lstlisting}[language=Python, label=code:example, caption=Example on how to use the Deep Logic library.]
import deep_logic as dl

# import train, validation and test data loaders
[...]

# instantiate a mu network
model = dl.models.MuNN(n_classes=n_classes, n_features=n_features,
                       hidden_neurons=[200], loss=torch.nn.CrossEntropyLoss(), 
                       l1_weight=0.001, fan_in=10)

# fit the model
model.fit(train_data, val_data, epochs=100, l_r=0.0001)

# get predictions on test samples
outputs, labels = model.predict(test_data)

# get first-order logic explanations for a specific target class
target_class = 1
formula = model.get_global_explanation(x_val, y_val, target_class)
# compute explanation accuracy
accuracy = dl.logic.test_explanation(formula, target_class, x_test, y_test)
\end{lstlisting}

% \textbf{Unless required by applicable law or agreed to in writing, software is distributed on an "as is" basis, without warranties or conditions of any kind, either express or implied.}

\subsection{Dataset and classification task details}
\label{sec:exp_details}
For the experimental analysis, we consider five categorical learning problems ranging from computer vision to medicine and democracy. Some datasets (e.g. CUB) were already annotated with high-level concepts (e.g. bird attributes) which can be exploited to train a concept bottleneck pipeline. For datasets without annotations for high-level concepts, we transform the input space into a predicate space (i.e. $\mathbb{R}^d \rightarrow [0,1]^d$) to make it suitable for training LENs. According to the considered data type, we evaluate and discuss the usage of  different LEN pipeline, classification and explanation style (see Tab. \ref{tab:datasets}).
For the sake of consistency, in all supervised experiments LENs were trained by optimizing Eq. \ref{eq:IFF}, therefore extracting IFF rules. However also Eq. \ref{eq:IF} \ref{eq.IF2} could be optimized, above all when explaining a black-box model.


\textsc{MIMIC-II - E2E Interpretable classification. }
The Multiparameter Intelligent Monitoring in Intensive Care II (MIMIC-II, \cite{saeed2011multiparameter,goldberger2000physiobank}) is a public-access intensive care unit (ICU) database consisting of 32,536 subjects (with 40,426 ICU admissions) admitted to
%medical, surgical, cardiovascular and neonatal ICUs, surgical recovery units, and coronary care units 
ICUs at a single tertiary care hospital. The dataset contains detailed description of a variety of clinical data classes: general,
%(e.g. patient demographics, hospital admission and discharge dates, hospital death dates, etc), 
physiological, % (e.g.	nurse-verified vital signs, blood pressure, heart rate, etc), 
results of clinical laboratory tests, % (e.g. hematology, blood chemistries, urinalysis, microbiology, etc), 
records of medications, fluid balance, %(e.g. solutions, urine, estimated blood loss, etc), 
and free text notes and reports of imaging studies (e.g. x-ray, CT, MRI, etc). In our experiments, we remove the text-based input features and 
%discretize some of the continuous features into a set of categories in order to get a one-hot encoded representation. For instance, 
we discretize blood pressure (BP) into five different categories (one-hot encoded): very low BP, low BP, normal BP, high BP, and very high BP. After such preprocessing step, we obtain an input space $X=C \subset [0,1]^d$ composed of $d=90$ key features. 
The task consists in training a classifier function to identify recovering ($Y=1$) or dying ($Y=0$) patients, after 28 days from ICU admission. In particular, we consider the case of
% {\bf Interpretable classification. }
\textit{Interpretable classification} where an End-to-End LEN $X=C \rightarrow E=Y$ is employed to carry out the classification task.
But we also considered the case of 

\textsc{MIMIC-II (EBB) - {E2E Explaining a black-box model}. } On the same dataset, a second task is set up. A black-box model $g$ $X=C \rightarrow Y$ is employed to solve the classification task, with predictions $g(C) \approx Y$. The end-to-end model $f$ $X=C \rightarrow E=g(C)$ instead is trained to mimic the behaviour of the black box $g$.

% \subsubsection{Concept bottleneck explainers}
% \label{sec:exp_cbm}

% \paragraph{MNIST Even/Odd}
\textsc{MNIST Even/Odd - {CB Interpretable classifications}. }
The Modified National Institute of Standards and Technology database (MNIST, \cite{lecun1998mnist}) contains a large collection of images representing handwritten digits. The input space $X \subset \mathbb{R}^{28\times 28}$ is composed of 28x28 pixel images while the concept space $C \subset [0,1]^{10}$ is represented by digits from $0$ to $9$. 
However, the task we aim to solve is slightly different from the common digit-classification. In the case of 
% {\bf Interpretable classification}
\textit{interpretable classification}, indeed, assuming $Y \subset [0,1]^2$, we are interested in determining if a digit is either odd or even, and explain the assignment to one of these classes in terms of the high-level concepts $C$ (digits). The mapping $X \rightarrow C$ is learned by a ResNet10 classifier $g$ \cite{he2016deep}  trained from scratch, while a LEN $f$ is used to learn both the mapping and the explanation as a function $C=g(X) \rightarrow E=Y$. 

% The $\mu$ network is equipped with a single hidden layer with 10 neurons and the $L_1$ loss weight $\lambda = 10^{-2}$. 
% The $ReLU$ network is equipped with two hidden layers composed of 30, 10 hidden neurons respectively and $\lambda = 10^{-3}$. 
% The $\psi$ network at last is equipped with no hidden layers, $\lambda = 10^-3$ and fan-in = 5. 
% All networks have been trained for 200 epochs with learning rate = $10^ {-3}$.

\textsc{MNIST E/O (IC) - {CB Interpretable clustering}. }
 The same dataset has been used to perform
% {\bf Interpretable Clustering}
\textit{Interpretable clustering}.  We consider a concept space $C \subset [0,1]^{12}$ which comprise both the digits and the even/odd labels. The mapping $X \rightarrow C$ is learned again by a Resnet10 model $g$ trained as a multi-label classifier, while the LEN $f$ performs clustering from $C=g(X) \rightarrow E$, where $E \subset [0,1]^{2}$ space, in order two extract two clusters. 
% In this case, 
% the $\mu$ network is equipped with two hidden layer with 20, 10 neurons respectively and the $L_1$ loss weight $\lambda = 10^{-3}$. 
% The $ReLU$ network is equipped with two hidden layers composed of 50, 30 hidden neurons and $\lambda = 10^{-4}$. 
% The $\psi$ network at last is equipped with no hidden layers, $\lambda = 10^{-2}$ and fan-in = 2. 
% The $\mu$ and the $ReLU$ networks have been trained for 100 epochs with learning rate = $10^{-3}$ while for the $\psi$ network is equal to $10^{-2}$.

%Quantitative results are reported in Table \ref{tab:exp_metrics_mnist_cbm} while Table \ref{tab:exp_formula_mnist_cbm} shows for each fold the explanation extracted from trained explainers.
\textsc{CUB - CB Interpretable Classification .}
The Caltech-UCSD Birds-200-2011 dataset (CUB, \cite{wah2011caltech}) is a fine-grained classification dataset. It includes 11,788 images representing $r = 200$ ($Y \subset [0,1]^{200}$) different bird species. 312 binary attributes have been also collected for each image representing visual characteristics (color, pattern, shape) of particular parts (beak, wings, tail, etc.). Attributes annotations, however, is quite noisy. Similarly to \cite{koh2020concept}, we denoised attributes by considering class-level annotations, i.e. a certain attribute is set as present only if it is also present in at least 50\% of the images of the same class. Furthermore we only considered attributes present in at least 10 classes after this refinement. In the end, a total of $d = 108$ attributes ($C \subset [0,1]^{108}$) have been retained. The mapping $X \rightarrow C$ from images to attribute concepts is performed again with a ResNet10 model $g$ trained from scratch while a LEN $f$ learns the final function $C = g(X) \rightarrow E=Y$.


\textsc{V-Dem - Cascade Interpretable classification. }
Varieties of Democracy (V-Dem, \cite{pemstein2018v,coppedge2021v}) is a dataset containing a collection of indicators of latent regime characteristics over 202 countries from 1789 to 2020. The database include $d_1 = 483$ low-level indicators $C_1 \subset [0,1]^{d_1}$ (e.g. media bias, party ban, high-court independence, initiatives permitted, etc), $d_2 = 82$ mid-level indices $C_1 \subset [0,1]^{d_2}$ (e.g. freedom of expression, freedom of association, equality before the law, etc), and 5 high-level indices of democracy principles (i.e. electoral, liberal, participatory, deliberative, and egalitarian). In the experiments a binary classification problem is considered to identify electoral democracies ($Y=1$) from non-electoral democracies ($Y=0$). Cascading LENs $f_1$ and $f_2$ are trained to learn the map $C_1 \rightarrow C_2 \rightarrow E=Y$.



\subsection{Quantitative metrics for model and explanations}
\label{sec:exp_metrics}
Seven metrics are used to compare the performance of LENs with respect to state-of-the-art approaches.
While measuring classification metrics is necessary for models to be viable in practice to perform interpretable classification tasks, assessing the quality of the explanations is required to justify their use for explainability. In contrast with other kind of explanations, logic-based formulas can be evaluated quantitatively. Given a classification problem, first we extract a set of rules from a trained model and then we test each explanation on an unseen set of samples.
The results for each metric are reported in terms of the mean and the standard error of the mean, computed over a 10-fold cross validation \cite{krzywinski2013error}. Only in the CUB experiments a 5-fold cross validation is performed due to timing issues related to BRL (each training of BRL on CUB lasts about 3 hours).
For each experiment we measure: 
% (1) the test accuracy of the classifier, (2) the test accuracy of the explanation, (3) the complexity of the explanation, (4) the fidelity of the explanation with respect to the classifier, (5) the elapsed time required to extract the explanations, (6) the consistency of the explanation over different runs, and (7) the normalized mutual information (for unsupervised tasks only). 
% \cite{andrews1995survey}. 

\begin{itemize}
\item The \textsc{model accuracy} measures how well the classifier correctly identifies the target class (see Table. \ref{tab:model-accuracy}). When the model is the classifier itself (i.e. interpretable classification), this metric represents the accuracy of the model. Instead, when the model explain the predictions of a black box classifier, this metric represents the accuracy of the black box classifier.
\item The \textsc{explanation accuracy} measures how well the extracted logic formula correctly identifies the target  class (see Table. \ref{tab:explanation-accuracy}).
\item The \textsc{complexity of an explanation} measures how hard would it be for a human being to understand the logic formula (see Table. \ref{tab:complexity}). This metric is computed by standardizing the explanations in disjunctive normal form and then by counting the number of terms of the standardized formula.
\item The \textsc{fidelity of an explanation} measures how well the predictions obtained using the extracted explanation match the predictions obtained using the classifier (see Table. \ref{tab:fidelity}). When the model is the classifier itself (i.e. interpretable classification), this metric represents the match between the extracted explanation and the model. Instead, when the model is explaining the predictions of a black box classifier, this metric represents the match between the extracted explanation and the black box classifier.
\item The \textsc{rule extraction} measures the time required to obtain an explanation from scratch. It is computed as the sum of the time required to train the (see Table. \ref{tab:extraction}) model and the time required to extract the formula from a trained model. This is justified by the fact that for some models, like BRL, training and rule extraction consist of just one simultaneous process.
\item The \textsc{consistency of an explanation} measures the similarity of the extracted explanations over different runs (see Table. \ref{tab:consistency}). It is computed by counting how many times the same concepts appear in the logic formulas over different folds of a cross-validation or over different initialization seeds.
% \item The \textsc{normalized mutual information} measures the quality of the clusters obtained in the interpretable clustering experiments. It is calculated as the mutual information of Eq. \ref{eq:MI}, divided by the Entropy $H_E$ so that it reports a number always comprehended between $[0,1]$.
\end{itemize}








\subsection{Results and Discussion}
% \textsc{Interpretable classification. } 
Experiments show how LENs generalize better than decision trees on complex Boolean functions (e.g. CUB and MIMIC-II) as already observed in \cite{tavares2020understanding} (Table. \ref{tab:model-accuracy}). For most experiments the formulas extracted from LENs are either better or almost as accurate as the formulas found by decision trees or mined by BRL (Table. \ref{tab:explanation-accuracy}). The complexity of LEN explanations is usually lower than the complexity of the rules extracted from a decision tree or mined by BRL. The complexity of decision tree formulas is never below 100 terms, making them useless for quick decision making (Table. \ref{tab:complexity}). White-box models like decision trees and BRL outperform LENs in terms of fidelity. Their predictions is directly based on the explanation therefore fidelity is always 100\%. However, the fidelity of the formulas extracted by the $\mu$ and the ReLU network is often higher than $90\%$. This means that almost any prediction has been correctly explained, making these networks very close to white boxes (Table. \ref{tab:fidelity}). BRL is the slowest rule extractor over all the experiments by one order of magnitude, while the decision tree is the fastest overall (Table. \ref{tab:extraction}). In terms of consistency there is not a dominant method (Table. \ref{tab:consistency}).

Fig. \ref{fig:multi-objective} shows the Pareto frontiers \cite{marler2004survey} for each experiment in terms of the complexity of the explanation and its classification error ($100 -$ classification accuracy). The simplest and most accurate formulas are found by the LENs, whose complexity is almost always below the maximum complexity laypeople can handle (i.e. complexity $\leq 9$ \cite{miller1956magical,cowan2001magical,ma2014changing}). Across all the experiments, there is at least one set of formulas extracted from out-of-the-box LEN dominating both BRL and decision trees.

For each dataset and for each method Table \ref{tab:best-rules} reports some compact FOL formula extracted. 


\textsc{Interpretable Clustering. } 
As introduced in the MNIST E/O dataset explanation we performed clustering starting from a Concept space composed of the 10 digits and the even/odd labels. The LEN are instructed two extract 2 clusters possibly respecting the even/odd division of digits. In Table \ref{tab:exp_metrics_mnist_mi} the metrics regarding this task are reported. We can see that all methods are capable to maximize the normalized mutual information. However only the $\psi$ network is capable to consistently explain the two clusters in terms of the important labels (even and odd), as we can see from the complexity of the rules (higher than 2 for the $\mu$ and ReLu net) and for the consistency of terms used in the explanation (100\% for the $\psi$ network). 
Other examples and application of Interpretable Clustering has been performed in \cite{ciravegna2020constraint, ciravegna2020human} employing the $\psi$ network only.

% \subsection{Other experiences}

% \textsc{Explanation as a defense}


\begin{table}[!h]
\centering
\caption{Model's accuracy (\%)}
\label{tab:model-accuracy}
\resizebox{\textwidth}{!}{
\begin{tabular}{lllllll}
\toprule
{} &         $\mu$ net &          ReLU net &        $\psi$ net &              Tree &               BRL & Black box \\
\midrule
\textbf{MIMIC-II     }  &  ${\bf 86.60 \pm 0.30}$ &  $85.36 \pm 0.78$ &  $84.01 \pm 0.09$ &  $79.56 \pm 0.80$ &  $86.15 \pm 0.51$ & N/A \\
\textbf{MIMIC-II (EBB)}  &  N/A &  N/A &  N/A &  N/A &  N/A  & $85.13 \pm 0.70$\\
\textbf{V-Dem         } &  $91.96 \pm 0.42$ &  $91.88 \pm 0.37$ &  $79.23 \pm 2.20$ &  $92.11 \pm 0.38$ &  ${\bf 92.23 \pm 0.38}$ & N/A \\
\textbf{MNIST}          &  $99.75 \pm 0.02$ &  $99.81 \pm 0.01$ &  $99.80 \pm 0.01$ &  ${\bf 99.96 \pm 0.01}$ &  $99.80 \pm 0.01$ & N/A \\
\textbf{CUB          }  &  ${\bf 92.26 \pm 0.28}$ &  $92.19 \pm 0.27$ &  $91.72 \pm 0.56$ &  $89.30 \pm 0.42$ &  $82.18 \pm 0.43$ & N/A \\

\bottomrule
\end{tabular}
}
\end{table}

\begin{table}[!h]
\centering
\caption{Explanation's accuracy (\%)}
\label{tab:explanation-accuracy}
\resizebox{\textwidth}{!}{
\begin{tabular}{llllll}
\toprule
{}                     &         $\mu$ net &          ReLU net &        $\psi$ net &              Tree &               BRL \\
\midrule
\textbf{MIMIC-II     } &  $85.08 \pm 0.48$ &  $82.09 \pm 1.38$ &  $82.83 \pm 0.66$ &  $79.56 \pm 0.80$ &   ${\bf86.15 \pm 0.51}$ \\
\textbf{MIMIC-II (EBB)} &  ${\bf85.75 \pm 0.51}$ &  $81.07 \pm 3.33$ &  $83.90 \pm 1.25$ &  $85.53 \pm 0.61$ &  $85.70 \pm 0.48$ \\
\textbf{V-Dem         } &  $90.81 \pm 1.24$ & ${\bf94.65 \pm 0.32}$ &  $80.29 \pm 2.99$ &  $92.11 \pm 0.38$ &  $92.23 \pm 0.38$ \\
\textbf{MNIST}         &  $99.67 \pm 0.01$ &  $98.04 \pm 1.60$ &  $75.47 \pm 0.46$ &  ${\bf99.96 \pm 0.01}$  &  $99.80 \pm 0.01$ \\
\textbf{CUB*         } &  ${\bf96.15 \pm 0.16}$ &  $93.98 \pm 1.97$ &  $80.41 \pm 2.31$ &  $89.30 \pm 0.42$ &  $82.18 \pm 0.43$ \\


\bottomrule
\end{tabular}
}
\end{table}

\begin{table}[!h]
\centering
\caption{Complexity}
\label{tab:complexity}
\resizebox{\textwidth}{!}{
\begin{tabular}{llllll}
\toprule
{}                     &        $\mu$ net &         ReLU net &       $\psi$ net &                 Tree &               BRL \\
\midrule
\textbf{MIMIC-II     } &  $5.10 \pm 0.35$ &  $23.40 \pm 11.20$ &  ${\bf2.60 \pm 0.16}$ &  $1342.60 \pm 16.94$ &  $20.70 \pm 4.08$ \\
\textbf{MIMIC-II (EBB)} &  $7.00 \pm 0.70$ &    $6.40 \pm 0.95$ &  ${\bf1.30 \pm 0.15}$ &   $432.10 \pm 16.46$ &  $22.90 \pm 4.13$ \\
\textbf{V-Dem         } &  $9.60 \pm 1.17$ &    $4.90 \pm 0.10$ &  ${\bf2.00 \pm 0.49}$ &    $294.10 \pm 7.88$ &   $8.70 \pm 0.97$ \\
\textbf{MNIST}         &  ${\bf22.00 \pm 4.67}$ &  $48.10 \pm 1.43$ &  $24.85 \pm 2.89$ &  $632.35 \pm 5.01$ &  $1291.05 \pm 234.40$ \\
\textbf{CUB          } &  $10.53 \pm 0.08$ &  $29.25 \pm 3.26$ &  $28.36 \pm 2.75$ &  $138.83 \pm 5.31$ &  ${\bf4.10 \pm 0.09}$ \\


\bottomrule
\end{tabular}
}
\end{table}

\begin{table}[!h]
\centering
\caption{Fidelity (\%)}
\label{tab:fidelity}
\resizebox{\textwidth}{!}{
\begin{tabular}{llllll}
\toprule
{}                     &         $\mu$ net &          ReLU net &        $\psi$ net &              Tree &               BRL \\
\midrule
\textbf{MIMIC-II     } &  $96.23 \pm 0.81$ &  $87.84 \pm 2.12$ &  $84.63 \pm 0.67$ &  ${\bf100.00 \pm 0.00}$ &  ${\bf100.00 \pm 0.00}$ \\
\textbf{MIMIC-II (EBB)} &  $92.28 \pm 0.90$ &  $86.58 \pm 4.00$ &  $90.32 \pm 1.27$ &   $93.07 \pm 0.53$ &   ${\bf94.82 \pm 0.50}$ \\
\textbf{V-Dem         } &  $91.52 \pm 1.13$ &  $94.62 \pm 0.37$ &  $82.45 \pm 1.80$ &  ${\bf100.00 \pm 0.00}$ &  ${\bf100.00 \pm 0.00}$ \\
\textbf{MNIST}         &  $99.90 \pm 0.03$ &  $98.14 \pm 1.60$ &  $75.53 \pm 0.46$ &  ${\bf100.00 \pm 0.00}$ &  ${\bf100.00 \pm 0.00}$ \\
\textbf{CUB*         } &  $97.82 \pm 0.15$ &  $95.37 \pm 2.06$ &  $81.89 \pm 2.35$ &  ${\bf100.00 \pm 0.00}$ &  ${\bf100.00 \pm 0.00}$ \\


\bottomrule
\end{tabular}
}
\end{table}

\begin{table}[!h]
\centering
\caption{Rule extraction time (s)}
\label{tab:extraction}
\resizebox{\textwidth}{!}{
\begin{tabular}{llllll}
\toprule
{} &        $\mu$ net &         ReLU net &       $\psi$ net &             Tree &              BRL \\
\midrule
\textbf{MIMIC-II     } &  $13.32 \pm 0.30$ &  $266.22 \pm 166.90$ &   $8.81 \pm 0.15$ &  ${\bf0.02 \pm 0.00}$ &  $495.59 \pm 7.13$ \\
\textbf{MIMIC-II (EBB)} &  $15.30 \pm 0.19$ &     $18.46 \pm 1.00$ &  $10.14 \pm 0.03$ &  ${\bf0.01 \pm 0.00}$ &  $543.43 \pm 3.39$ \\
\textbf{V-Dem         } &  $34.40 \pm 0.78$ &     $34.24 \pm 0.32$ &  $20.83 \pm 0.04$ &  ${\bf0.06 \pm 0.00}$ &   $53.69 \pm 0.41$ \\
\textbf{MNIST}         &  $173.24 \pm 6.77$ &  $221.07 \pm 4.06$ &  $236.71 \pm 3.36$ &  ${\bf2.04 \pm 0.04}$ &  $836.14 \pm 3.15$ \\
\textbf{CUB          } &  $726.19 \pm 2.43$ &  $660.30 \pm 121.16$ &  $2094.49 \pm 730.50$ &  ${\bf4.17 \pm 0.07}$ &  $9863.52 \pm 147.57$ \\

\bottomrule
\end{tabular}
}
\end{table}

\begin{table}[!h]
\centering
\caption{Rule consistency (\%)}
\label{tab:consistency}
\begin{tabular}{llllll}
\toprule
{} & $\mu$ net & ReLU net & $\psi$ net &     Tree &      BRL \\
\midrule
\textbf{MIMIC-II     } &   $51.00$ &  $26.00$ &    $37.14$ &  ${\bf81.50}$ &  $28.33$ \\
\textbf{MIMIC-II (EBB)} &   $41.18$ &  $35.56$ &    $43.33$ &  ${\bf60.36}$ &  $22.22$ \\
\textbf{V-Dem         }&   $71.67$ &  ${\bf98.00}$ &    $15.83$ &  $36.86$ &  $76.25$ \\
\textbf{MNIST}         &   $60.00$ &  ${\bf100.00}$ &    $50.00$ &  $50.95$ &  ${\bf100.00}$ \\
\textbf{CUB          } &   ${\bf58.82}$ &  $58.40$ &    $43.08$ &  $21.79$ &  $30.00$ \\

\bottomrule
\end{tabular}
\end{table}



\begin{figure}[!h]
    \centering
    \includegraphics[width=0.49\textwidth]{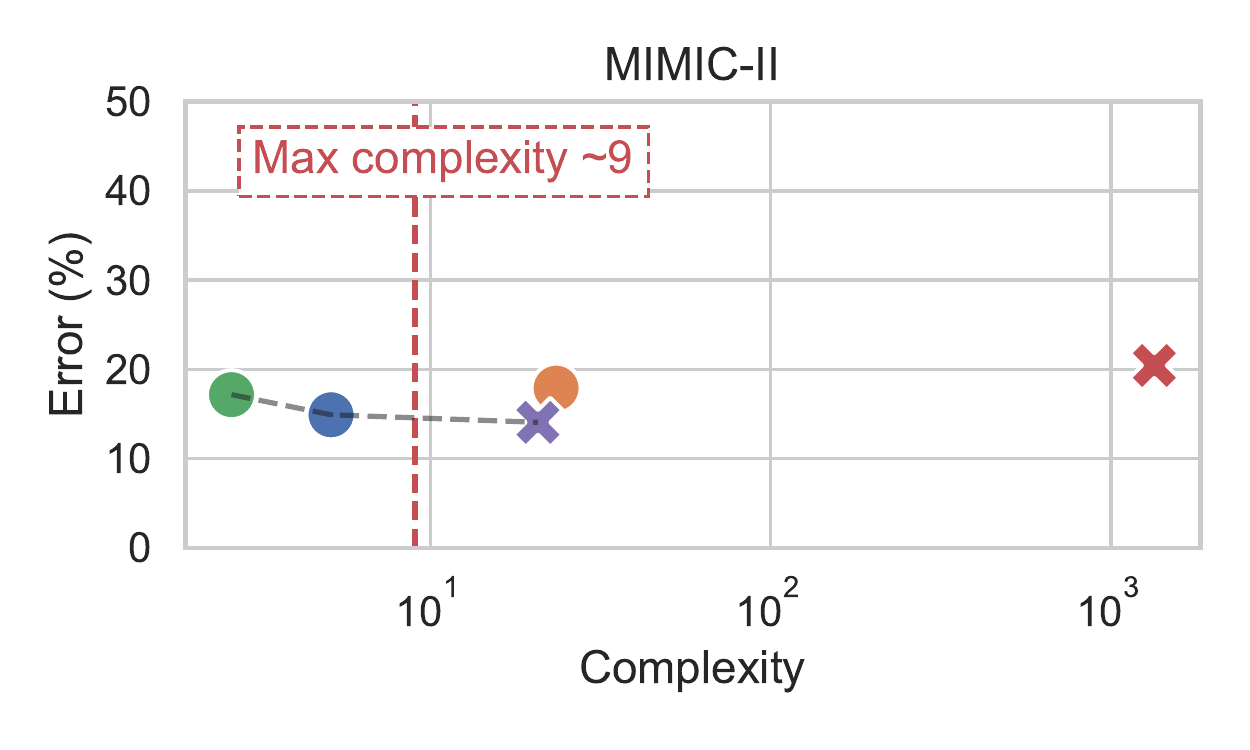}
    \includegraphics[width=0.49\textwidth]{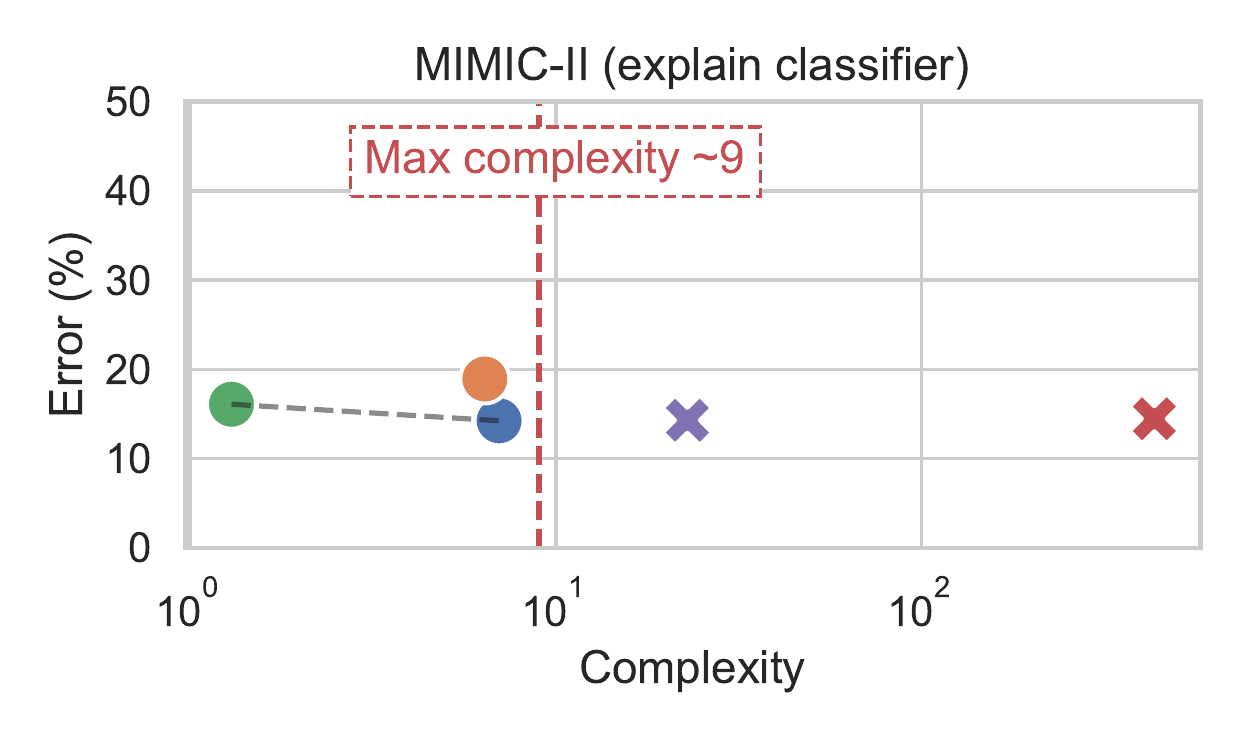}\\
    \includegraphics[width=0.49\textwidth]{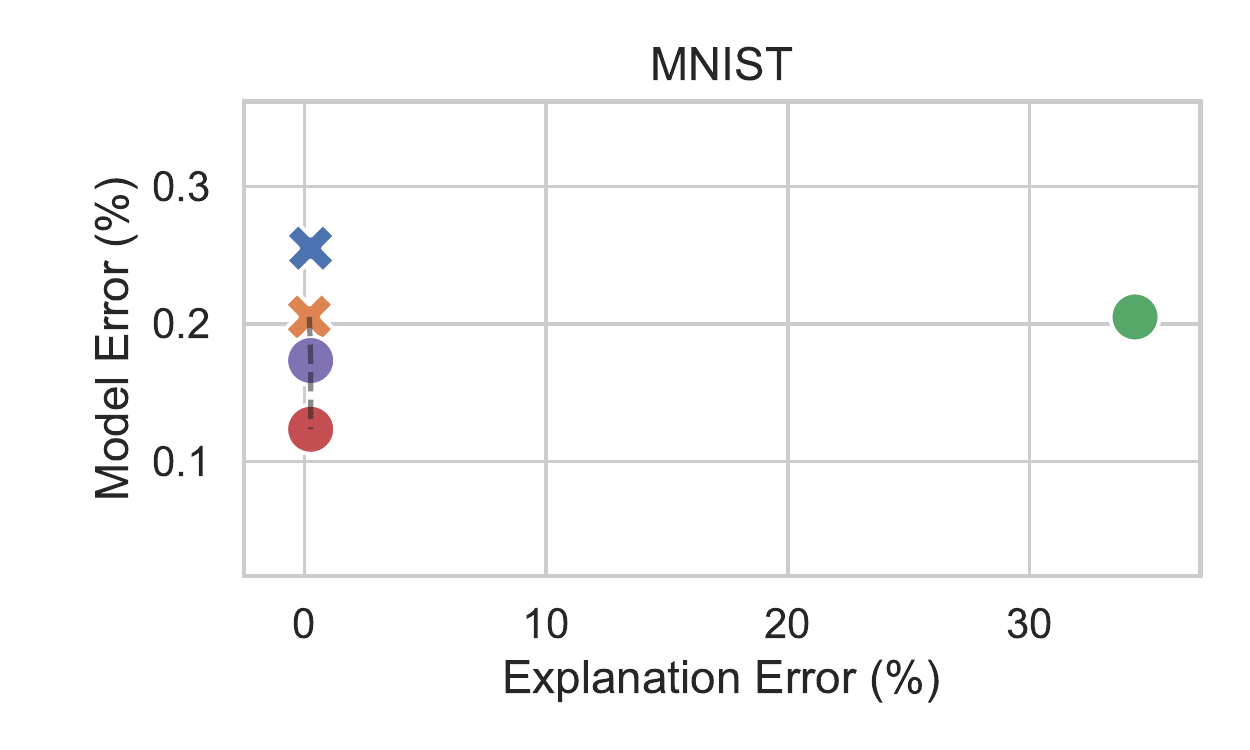}
    \includegraphics[width=0.49\textwidth]{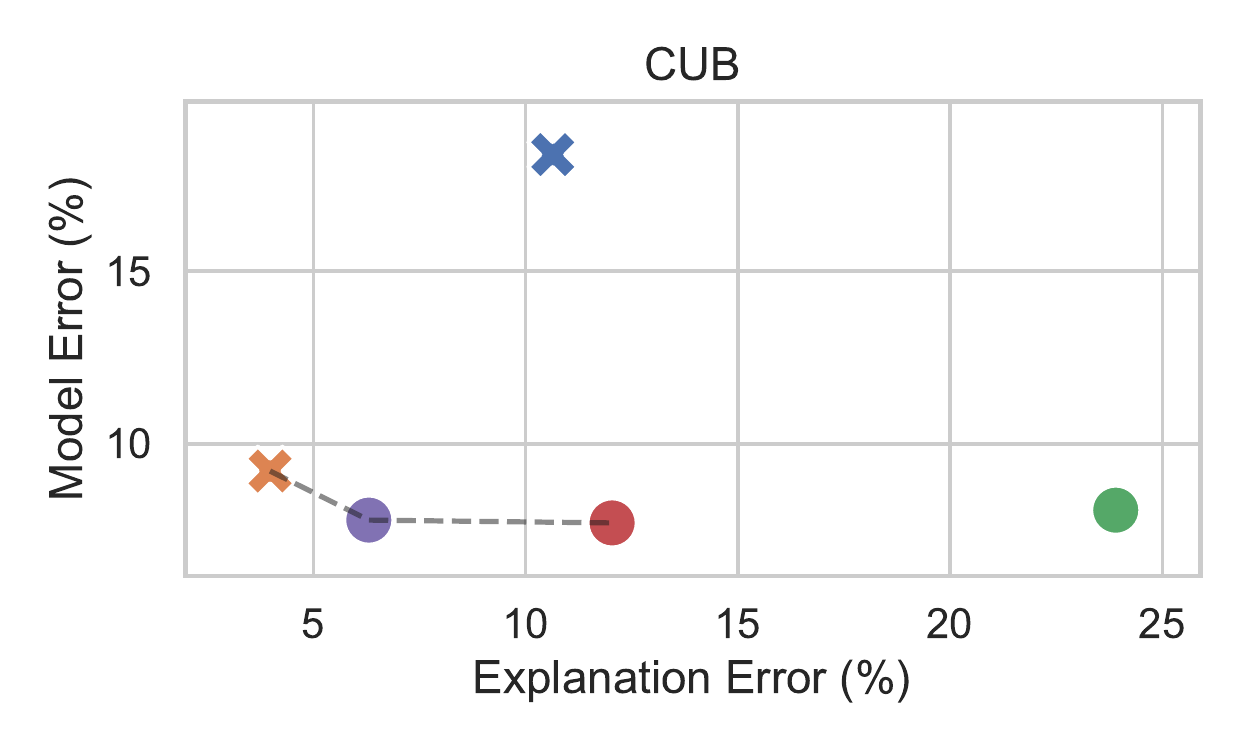}\\
    \includegraphics[width=0.49\textwidth]{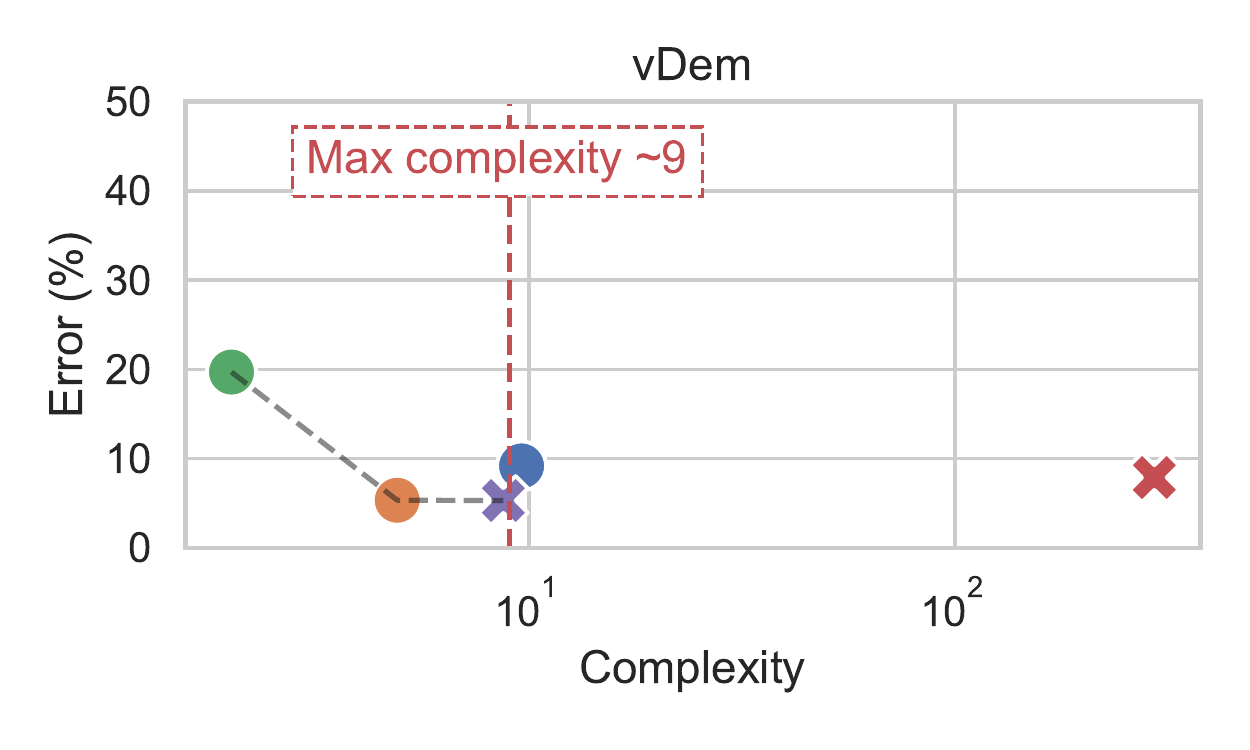}
    \\
    \includegraphics[width=0.7\textwidth]{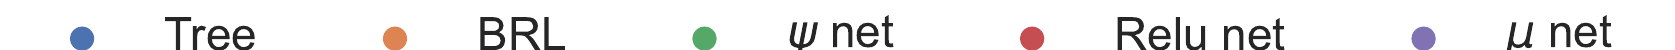}
    \caption{Pareto frontiers (dotted black line) in terms of average test error and average complexity of the explanations. Formulas out-of-the-box extracted from out-of-the-box LENs are reported as circles while BRL and decision trees as crosses. The vertical dotted red line marks the maximum explanation complexity laypeople can handle (i.e. complexity $\leq 9$ \cite{miller1956magical,cowan2001magical,ma2014changing}).}
    \label{fig:multi-objective}
\end{figure}

\begin{table}[!h]
\centering
\caption{MNIST Mutual Information}
\label{tab:exp_metrics_mnist_mi}
\resizebox{\textwidth}{!}{
\begin{tabular}{llllll}
\toprule
     Method & Model's accuracy (\%) & Exp. accuracy (\%) &       Complexity & Extraction time (s) & Rule consistency (\%) \\
\midrule
 $\psi$  net &     $99.90 \pm 0.01$ &           $99.90 \pm 0.01$ &  $2.00 \pm 0.00$ &     $0.33 \pm 0.15$ &             $100.00$ \\
 $\mu$ net &     $94.91 \pm 4.99$ &           $95.41 \pm 4.50$ &  $2.30 \pm 0.64$ &     $2.36 \pm 0.75$ &              $35.00$ \\
   ReLU net &     $96.87 \pm 3.04$ &           $95.97 \pm 3.94$ &  $2.15 \pm 0.39$ &     $4.15 \pm 1.62$ &              $45.00$ \\
\bottomrule
\end{tabular}
}
\end{table}





% \subsection{Rules Extracted}

% Please add the following required packages to your document preamble:
% \usepackage{multirow}
% \usepackage{graphicx}
{\renewcommand{\arraystretch}{2.5}
\begin{table}[!h]
\centering
\caption{A selection of some of the best rules extracted for each experiment.}
\label{tab:best-rules}
\resizebox{\textwidth}{!}{%
\begin{tabular}{lll}
\hline
\multicolumn{1}{l}{\textbf{Dataset}}    & \textbf{Model}  & \textbf{Rule} \\ \hline
\multirow{5}{*}{MIMIC-II}      & $\mu$ net  & $Death \leftarrow stroke \wedge age\_HIGH  \wedge \neg atrial\_fibrillation $  \\
                               & ReLU net   & $Death \leftarrow stroke \wedge age\_HIGH \wedge \neg atrial_fibrillation \wedge \neg sapsi\_first\_LOW \wedge \neg sapsi\_first\_HIGH $  \\
                               & $\psi$ net & $Death \leftarrow stroke \vee bun\_first\_NORMAL \vee sapsi\_first\_HIGH $  \\
                               & Tree       & $Death \leftarrow \quad ^*$formula is too long (1000+ terms) \\ 
                               & BRL        & $Death \leftarrow \makecell[l]{(stroke \wedge resp \wedge \neg age\_LOW \wedge \neg sapsi\_first\_LOW) \\
                               \vee (stroke  \wedge age\_HIGH \wedge \neg age\_LOW  \wedge  \neg sapsi\_first\_LOW) }$  \\ \hline
\multirow{5}{*}{MIMIC-II (EBB)} & $\mu$ net  & $Death \leftarrow atrial_fibrillation \wedge stroke \wedge \neg sapsi\_first\_HIGH \wedge \neg weight\_first\_NORMAL $  \\
                               & ReLU net   & $Death \leftarrow stroke \wedge \neg sapsi\_first\_LOW  \wedge  \neg sapsi\_first\_HIGH \wedge \neg sodium\_first\_LOW $  \\
                               & $\psi$ net & $Death \leftarrow stroke \wedge age\_HIGH $  \\
                               & Tree       & $Death \leftarrow  \quad ^*$formula is too long (100+ terms)  \\ 
                               & BRL        & $Death \leftarrow \makecell[l]{stroke \wedge age\_HIGH \wedge weight\_first\_LOW \wedge \neg sapsi\_first\_LOW) \\ \vee  (stroke \wedge platelet\_first\_HIGH \wedge weight\_first\_LOW \wedge \neg sapsi\_first\_LOW } $  \\  \hline
\multirow{5}{*}{MNIST}         & $\mu$ net  & $Even \leftarrow \neg One \wedge \neg Three \wedge \neg Five \wedge \neg Seven \wedge \neg Nine $  \\
                              & ReLU net   & $Even \leftarrow \makecell[l]{(Zero \wedge \neg One \wedge \neg Two \wedge \neg Three \wedge \neg Four \wedge \neg Five \wedge \neg Six \wedge \neg Seven \wedge \neg Eight \wedge \neg Nine) \\ 
                              \vee (Two \wedge \neg Zero \wedge \neg One \wedge \neg Three \wedge \neg Four \wedge \neg Five \wedge \neg Six \wedge \neg Seven \wedge \neg Eight \wedge \neg Nine) \\ 
                              \vee (Four \wedge \neg Zero \wedge \neg One \wedge \neg Two \wedge \neg Three \wedge \neg Five \wedge \neg Six \wedge \neg Seven \wedge \neg Eight \wedge \neg Nine) \\ 
                              \vee (Six \wedge \neg Zero \wedge \neg One \wedge \neg Two \wedge \neg Three \wedge \neg Four \wedge \neg Five \wedge \neg Seven \wedge \neg Eight \wedge \neg Nine) \\
                              \vee (Eight \wedge \neg Zero \wedge \neg One \wedge \neg Two \wedge \neg Three \wedge \neg Four \wedge \neg Five \wedge \neg Six \wedge \neg Seven \wedge \neg Nine) } $ \\
                              & $\psi$ net & $Even \leftarrow \makecell[l]{(Six \wedge Zero \wedge \neg One \wedge \neg Seven)  \vee (Six \wedge Zero \wedge \neg One \wedge \neg Three)  \\
                              \vee (Six \wedge Zero \wedge \neg Seven \wedge \neg Three)  \vee (Six \wedge \neg One \wedge \neg Seven \wedge \neg Three) \\
                              \vee (Zero \wedge \neg One \wedge \neg Seven \wedge \neg Three)  \vee (Six \wedge Zero \wedge \neg One \wedge \neg Seven \wedge \neg Three)}$  \\
                              & Tree       & $Even \leftarrow \quad ^*$formula is too long \\
                              & BRL        & $Even \leftarrow  \makecell[l]{(Six \wedge \neg Three \wedge \neg (Five \wedge \neg Two)) \vee (Eight \wedge \neg Nine \wedge \neg Six \wedge \neg Three \wedge \neg (Five \wedge \neg Two)) 
                              \\ \vee (Four \wedge \neg Nine \wedge \neg Six \wedge \neg Three \wedge \neg (Eight \wedge \neg Nine) \wedge \neg (Five \wedge \neg Two) \wedge \neg (Seven \wedge \neg Two)) \\ 
                              \vee (Two \wedge \neg One \wedge \neg Six \wedge \neg Three \wedge \neg (Eight \wedge \neg Nine) \wedge \neg (Five \wedge \neg Two) \\ \wedge \neg (Four \wedge \neg Nine) \wedge \neg (Seven \wedge \neg Nine) \wedge \neg (Seven \wedge \neg Two)) \\
                              \vee (Four \wedge \neg Six \wedge \neg Three \wedge \neg (Eight \wedge \neg Nine) \\ \wedge  \neg (Five \wedge \neg Two) \wedge \neg (Four \wedge \neg Nine) \wedge \neg (Seven \wedge \neg Nine) \wedge \neg (Seven \wedge \neg Two) \wedge \neg (Two \wedge \neg One)) \\
                              \vee (Zero \wedge \neg Four \wedge \neg Nine \wedge \neg Six \wedge \neg Three \wedge \neg (Eight \wedge \neg Nine) \wedge \neg (Five \wedge \neg Two) \wedge \neg (Four \wedge \neg Nine) \\
                              \wedge \neg (Nine \wedge \neg Zero) \wedge \neg (One \wedge \neg Two) \wedge \neg (Seven \wedge \neg Nine) \wedge \neg (Seven \wedge \neg Two) \wedge \neg (Two \wedge \neg One))
                              }$  \\ \hline
\multirow{5}{*}{CUB}          & $\mu$ net  & $ Black\ foot\ albatross \leftarrow \makecell[l]{  bill \ shape \ hooked \ seabird \ \wedge \  size \ medium \wedge \ wing \ pattern \ solid \\
                              \wedge \neg wing color \ black \wedge \neg  underparts\ color\ white \wedge \neg upper\ tail\ color\ grey \\
                              \wedge \neg breast\ color\ white \wedge \neg  throat\ color\ white \wedge \neg tail\ pattern\ solid \wedge \neg  crown\ color\ white} $  \\
                              & ReLU net   & $ Black\ foot\ albatross \leftarrow  \makecell[l]{ size\  medium  \wedge \neg  bill\  shape\  allpurpose  \\ 
                              \wedge \neg  upperparts\  color\  black  \wedge \neg  head\  pattern\  plain  \wedge \neg  under\  tail\  color\  yellow \\  \wedge \neg  under\  tail\  color\  black  \wedge \neg  nape\  color\  buff  \\
                              \wedge \neg  wing\  shape\  roundedwings  \wedge \neg  shape\  perchinglike  \\
                              \wedge \neg  leg\  color\  grey  \wedge \neg  leg\  color\  black  \wedge \neg  bill\  color\  grey  \\
                              \wedge \neg  bill\  color\  black  \wedge \neg  wing\  pattern\  multicolored }$\\
                              & $\psi$ net & $ Black\ foot\ albatross \leftarrow  \makecell[l]{(bill \ shape \ hooked\ seabird \wedge tail \ pattern \ solid \wedge \neg underparts \ color \ white \\
                              \wedge ( \neg  \ breast \ color \ white \vee \neg   \ wing \ color \ grey)) }$  \\
                              & Tree       & $ Black\ foot\ albatross \leftarrow  ^*$formula is too long (1000+ terms)  \\
                              & BRL        & $ Black\ foot\ albatross \leftarrow  \makecell[l]{( bill\  shape\  hooked\  seabird \wedge forehead\ color\ blue \wedge  \neg  bill\  color\  black \wedge  \neg  nape\  color\  white) \\
                              \vee ( bill\  shape\  hooked\  seabird \wedge  \neg  bill\  color\  black \wedge  \neg  nape\  color\  white \wedge  \neg  tail\  pattern\  solid)}$ \\ 
\hline
\multirow{5}{*}{V-Dem}         & $\mu$ net  & $Elect\_ Dem \leftarrow v2x\_freexp\_altinf \wedge v2x\_frassoc\_thick \wedge v2xel\_frefair \wedge v2x\_elecoff \wedge v2xcl\_rol $  \\
                               & ReLU net   & $Elect\_ Dem \leftarrow v2x\_freexp\_altinf \wedge v2xel\_frefair \wedge v2x\_elecoff \wedge v2xcl\_rol $  \\
                               & $\psi$ net & $Elect\_ Dem \leftarrow v2x\_frassoc\_thick \wedge v2xeg\_eqaccess $  \\
                               & Tree       & $Elect\_ Dem \leftarrow \quad ^*$formula is too long (1000+ terms)  \\
                               & BRL        & $Elect\_ Dem \leftarrow v2x\_freexp\_altinf \wedge v2x\_frassoc\_thick \wedge v2xel\_frefair \wedge v2x\_elecoff \wedge v2xcl\_rol $  \\ \hline
\end{tabular}%
}
\end{table}}



% These challenging or product-oriented contexts are the actual targets of XAI research. This great research effort have produced a variety of quite interesting and efficient approaches to unveil the decision process of black-box models. Some of the most common taxonomies are based on a few discriminative criteria (intrinsic interpretability VS post-hoc, model-specific VS model-agnostic, local VS global explanations), but the most important characteristic, i.e. the \textit{form} of the explanation, is often overlooked.

% include white-box models, model-agnostic approaches \cite{ribeiro2016model} and example-based explanations \cite{aamodt1994case,kim2016examples,barbiero2020uncovering}. 


% decision trees \cite{breiman1984classification}, or decision rules: oneR \cite{holte1993very}, RIPPER \cite{cohen1995fast}, Bayesian Rule Lists \cite{letham2015interpretable}).

% \begin{itemize}
%     \item many interesting works around explainability, from fully interpretable models (LR, DT, DR), to surrogates (LIME, Anchors, SHAP, etc) to example-based
%     \item great effort on scoring/ranking features/concepts
%     \item that's NOT the whole point
%     \item what matters (even more?) is how concepts are related (PDP? mah...)
%     \item what is the effort for the end user for analyzing a pairwise dependence plot or a ranking or a decision tree with depth 5?
%     \item good explanations must be simple
%     \item simple <-> few concepts involved? well yes, but...
%     \item traditional methods tend to assume: simplicity -> simple relationships among concepts (linear, max PDP)
%     \item we argue: why??
% \end{itemize}

% % -idee generali su che tipo di bestie c'è per fare expl.. 
% % -s'è già detto che i sistemi a regole sono più utili per fare supporto a umani.. che robe c'è in giro, perchè il nostro è più fiho
% % - il survey congnitivo dice che regole buone devono essere semplici.. -> pruning! che tipi di pruning usa sta gente che fa expl?

% What Is an Explanation? An explanation is the answer to a why-question (Miller 2017).


% to mention: (Bayesian Rule Lists: \cite{letham2015interpretable} tipo decision trees)

% \begin{itemize}
%     \item taxonomy
%     \begin{itemize}
%         \item intrinsic or post-hoc? LENs support both!
%         \item result of the interpretation:
%         \begin{itemize}
%             \item Feature summary statistic (feature importance or pairwise feature interactions or rank visualization)
%             \item Model internals (weights in linear models or the learned tree structure)
%             \item Data point (counterfactual explanations or identification of prototypes of predicted classes)
%             \item Intrinsically interpretable model
%         \end{itemize}
%         \item Model-specific or model-agnostic?
%         \item Local or global?
%     \end{itemize}
%     \item Properties of Explanation Methods
%     \begin{itemize}
%         \item Expressive Power is the "language" or structure of the explanations (IF-THEN rules, decision trees, a weighted sum, natural language or something else)
%         \item Translucency describes how much the explanation method relies on looking into the machine learning model
%         \item Portability 
%         \item Algorithmic Complexity
%     \end{itemize}
%     \item Properties of Individual Explanations
%     \begin{itemize}
%         \item Accuracy: How well does an explanation predict unseen data?
%         \item Fidelity: How well does the explanation approximate the prediction of the black box model?
%         \item Consistency: How much does an explanation differ between models that have been trained on the same task and that produce similar predictions?
%         \item Stability: How similar are the explanations for similar instances?
%         \item Comprehensibility: How well do humans understand the explanations?
%         \item Certainty: Does the explanation reflect the certainty of the machine learning model?
%         \item Degree of Importance: How well does the explanation reflect the importance of features or parts of the explanation?
%         \item Novelty: Does the explanation reflect whether a data instance to be explained comes from a "new" region far removed from the distribution of training data?
%         \item Representativeness: How many instances does an explanation cover?
%     \end{itemize}
%     \item good explanations
%     \begin{itemize}
%         \item Explanations are contrastive (Lipton 1990)
%         \item Explanations are selected (simple)
%         \item Explanations are social. They are part of a conversation
%         \item Explanations focus on the abnormal. People focus more on abnormal causes to explain events (Kahnemann and Tversky, 1981).
%         \item Explanations are truthful. Good explanations prove to be true in reality
%         \item Good explanations are consistent with prior beliefs of the explainee
%         \item Good explanations are general
%     \end{itemize}
%     \item interpretable models: logistic regression, decision trees, decision rules and the RuleFit algorithm
%     \item model agnostic: 
%     \begin{itemize}
%         \item plots: Accumulated local effects, Partial Dependence Plot, Individual Conditional Expectation
%         \item surrogates: Global Surrogate, Local Surrogate (LIME), \textbf{Scoped Rules (Anchors)} (many scenarios require discretization, many calls to the ML model), \textbf{SHAP} (SHapley Additive exPlanations)
%     \end{itemize}
%     \item example based: Counterfactual explanations, Prototypes
%     \item neural networks: Feature Visualization, Concepts, Modell Distillation (How can we explain a neural network with a simpler model?)
% \end{itemize}

% \paragraph{Occam's razors}
% In his Posterior Analytics, Aristotle stated: "We may assume the superiority ceteris paribus [other things being equal] of the demonstration which derives from fewer postulates or hypotheses" \cite{aristotlePosterior}. The \textit{law of parsimony} presented by the Greek philosopher has deeply influenced researchers and scientists across the centuries. In other words, when humans compare a set of explanations outlining the same outcomes, they tend to have an implicit bias towards the simplest one. Researchers have proposed many approaches to integrate this parsimony principle into learning machines over the years. Bayesian priors \cite{wilson2020case} and weight regularization \cite{kukavcka2017regularization} are just some of the most famous approaches. Among such techniques, $L1$-regularization \cite{santosa1986linear,tibshirani1996regression} has been recently shown quite effective for neural networks providing logic-based explanations \cite{ciravegna2020human} as it encourages sparsity by shrinking the less important weight's values to zero thus removing some weights altogether in the limit. Following \cite{ciravegna2020human}, the models analyzed in this work are mainly based on $L1$-regularization. However, in future works it may also worth exploring the integration of LENs with concept-based parsimony criteria \cite{chen2020concept} or with fuzzy-logic regularizers which have recently been used to combine deductive reasoning and human priors with deep learning \cite{marra2019lyrics}.




\section{Conclusion} \label{sec:conclusion}

\subsection{Limitations and future research directions}
The extraction of a first-order logic explanation requires symbolic input and output spaces. This constraint is the main limitation of our framework, as narrows the range of applications down to symbolic I/O problems. In some contexts, such as computer vision, the use of LENs may require additional annotations and attribute labels to get a consistent symbolic layer of concepts. However, recent work on automatic concept extraction may partially solve this issue leading to more cost-effective concept annotations \cite{ghorbani2019towards,kazhdan2020now}.

Another area to focus on might be the improvement of out-of-the-box LENs. The efficiency and the classification performances of fully interpretable LENs, i.e. $\psi$ network, is still quite limited due to the extreme pruning strategy. Even more flexible approaches, like $\mu$ networks, are not as efficient as standard neural models when tackling multi-class or multi-label classification problems, as they require a bigger architecture to provide a disentangled explanation for each class.

In our vision this framework would thrive and express its full potential by interacting with the external world and especially with humans in a dynamic way. In this case, logic formulas might be rewritten as sentences to allow for a more natural interaction with end users. Moreover, a dynamic interaction may call for an extended expressivity leading to higher-order or temporal logic explanations. Finally, in some contexts different neural architectures as graph neural networks might be worth exploring as they may be more suitable to solve the classification problem.


\subsection{Broader impact}
Current legislation in US and Europe binds AI to provide explanations especially when the economical, ethical, or financial impact is significant \cite{gdpr2017,law10code}. This work contributes to a lawful and safer adoption of some of the most powerful AI technologies allowing deep neural networks to have a greater impact on society. Extracting first-order logic explanations from deep neural networks enables satisficing knowledge distillation while achieving performances comparable with the state of the art. The formal language of logic provides clear and synthetic explanations, suitable for laypeople, managers, and in general for decision makers outside the AI research field. 

The experiments show how this framework can be used to aid bias identification and to make black boxes more robust to adversarial attacks by giving an explanation for the attack itself. As out-of-the-box LENs are easy to use even for neophytes and can be effectively used to understand the behavior of an existing algorithm, our approach might be used to reverse engineer competitor products, to find vulnerabilities, or to improve system design. From a scientific perspective, formal knowledge distillation from state-of-the-art networks may enable scientific discoveries or confirmation of existing theories.


\section*{Acknowledgments and Disclosure of Funding}
We thank ... for useful feedback and suggestions.

This work was partially supported by the European Union’s Horizon 2020 research and innovation programme under grant agreement No 848077.




\bibliographystyle{apalike}  % Sry Pietro, just had to
\bibliography{references}  %%% Remove comment to use the external .bib file (using bibtex).
%%% and comment out the ``thebibliography'' section.

\end{document}
